# Supplementary material for: Quancurrent: A Concurrent Quantiles Sketch
Source: arXiv:2208.09265 source file (2022-08-19)
Supplement: Supplementary file 2 [file ParameterExploration.tex]

\subsubsection{Compare b}
\FloatBarrier
\begin{figure*}[]
 \centering
    \begin{subfigure}[t]{0.49\textwidth}
    \includegraphics[width=\textwidth,trim={0 0.3cm 1.9cm 2.5cm},clip]{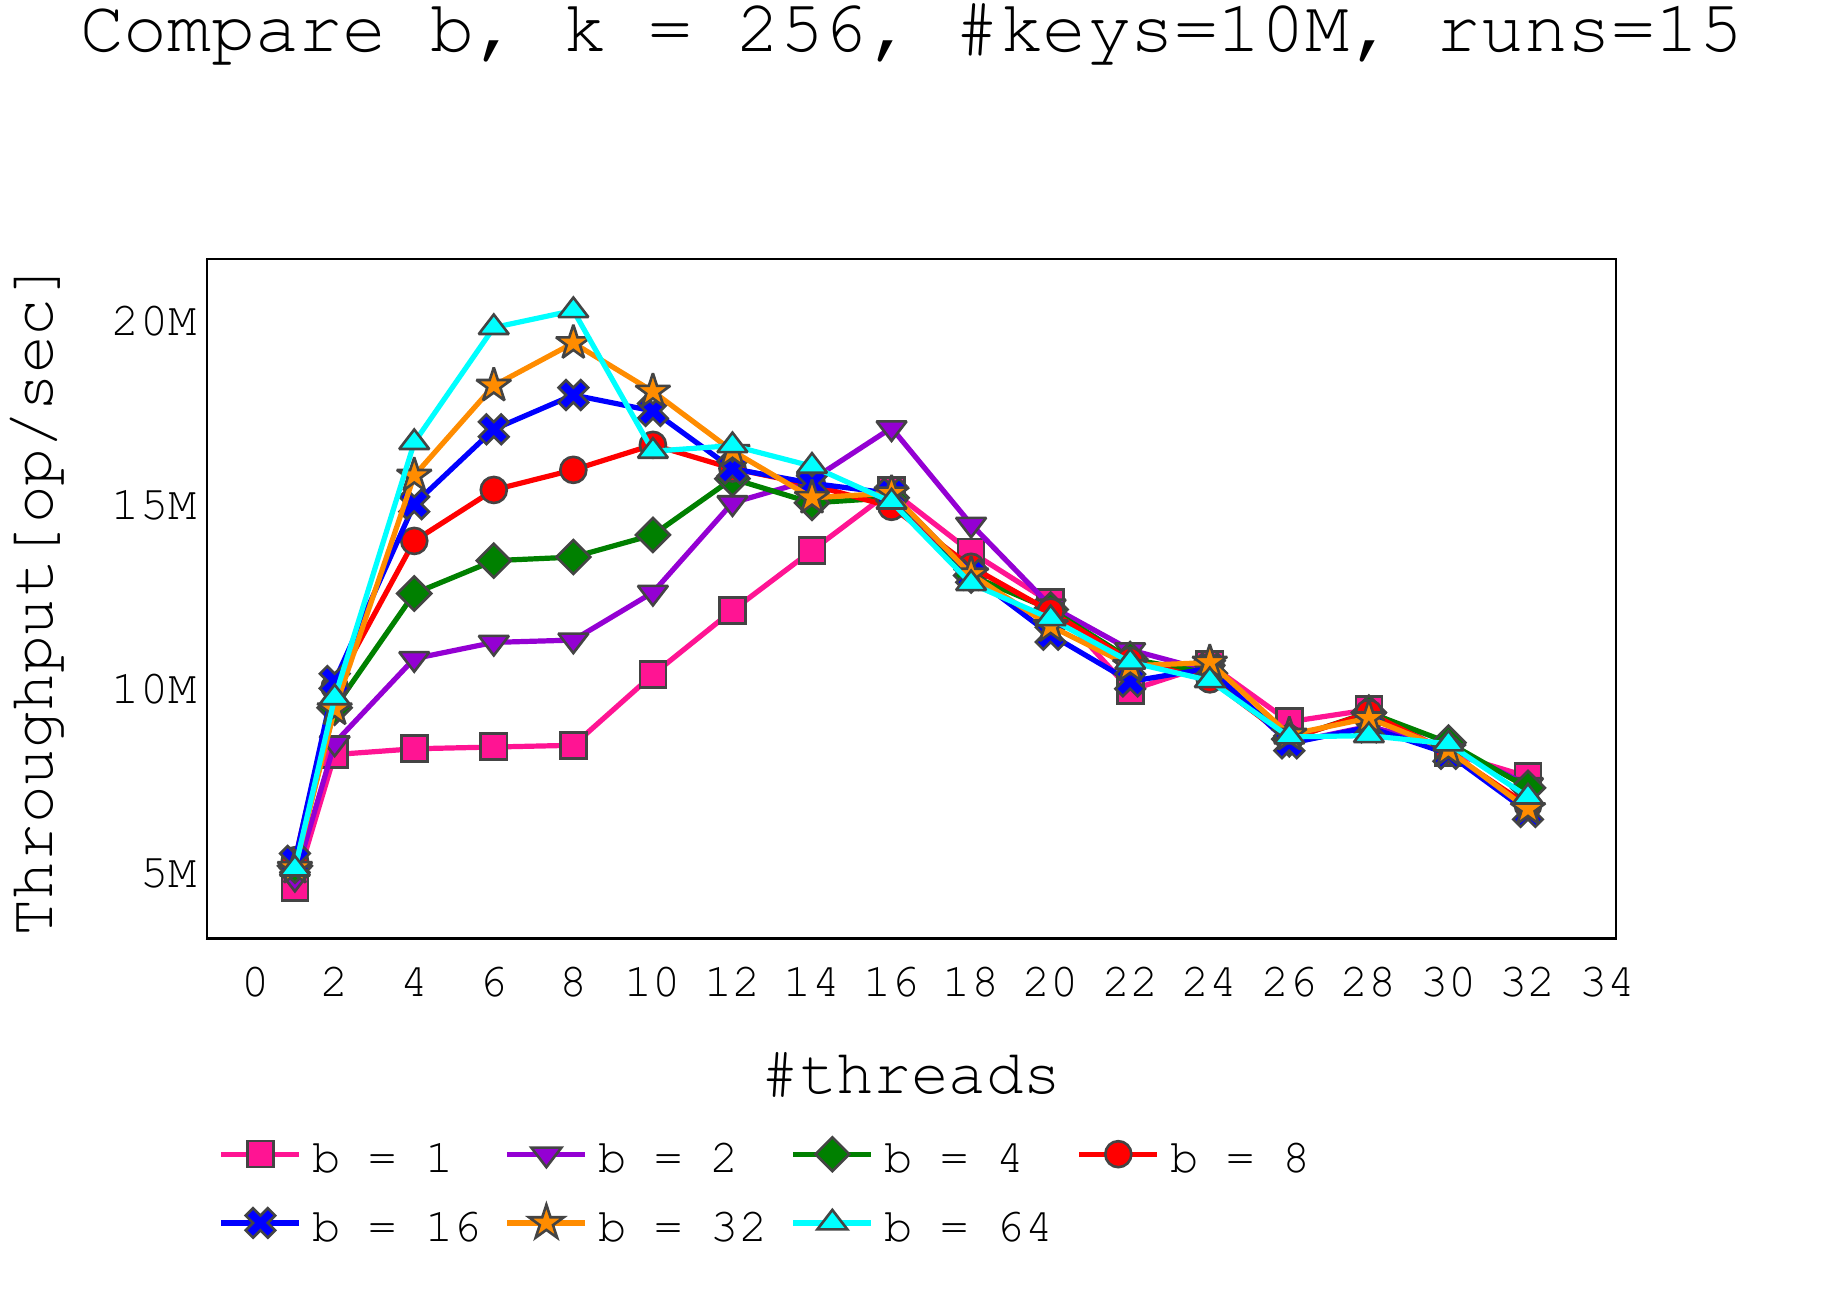}
    \caption{k = 256, 10M elements.}
    \label{fig: compare_b_k256_appendix}
    \end{subfigure}
    \hfill
    \begin{subfigure}[t]{0.49\textwidth}
    \includegraphics[width=\textwidth,trim={0 0.3cm 1.9cm 2.5cm},clip]{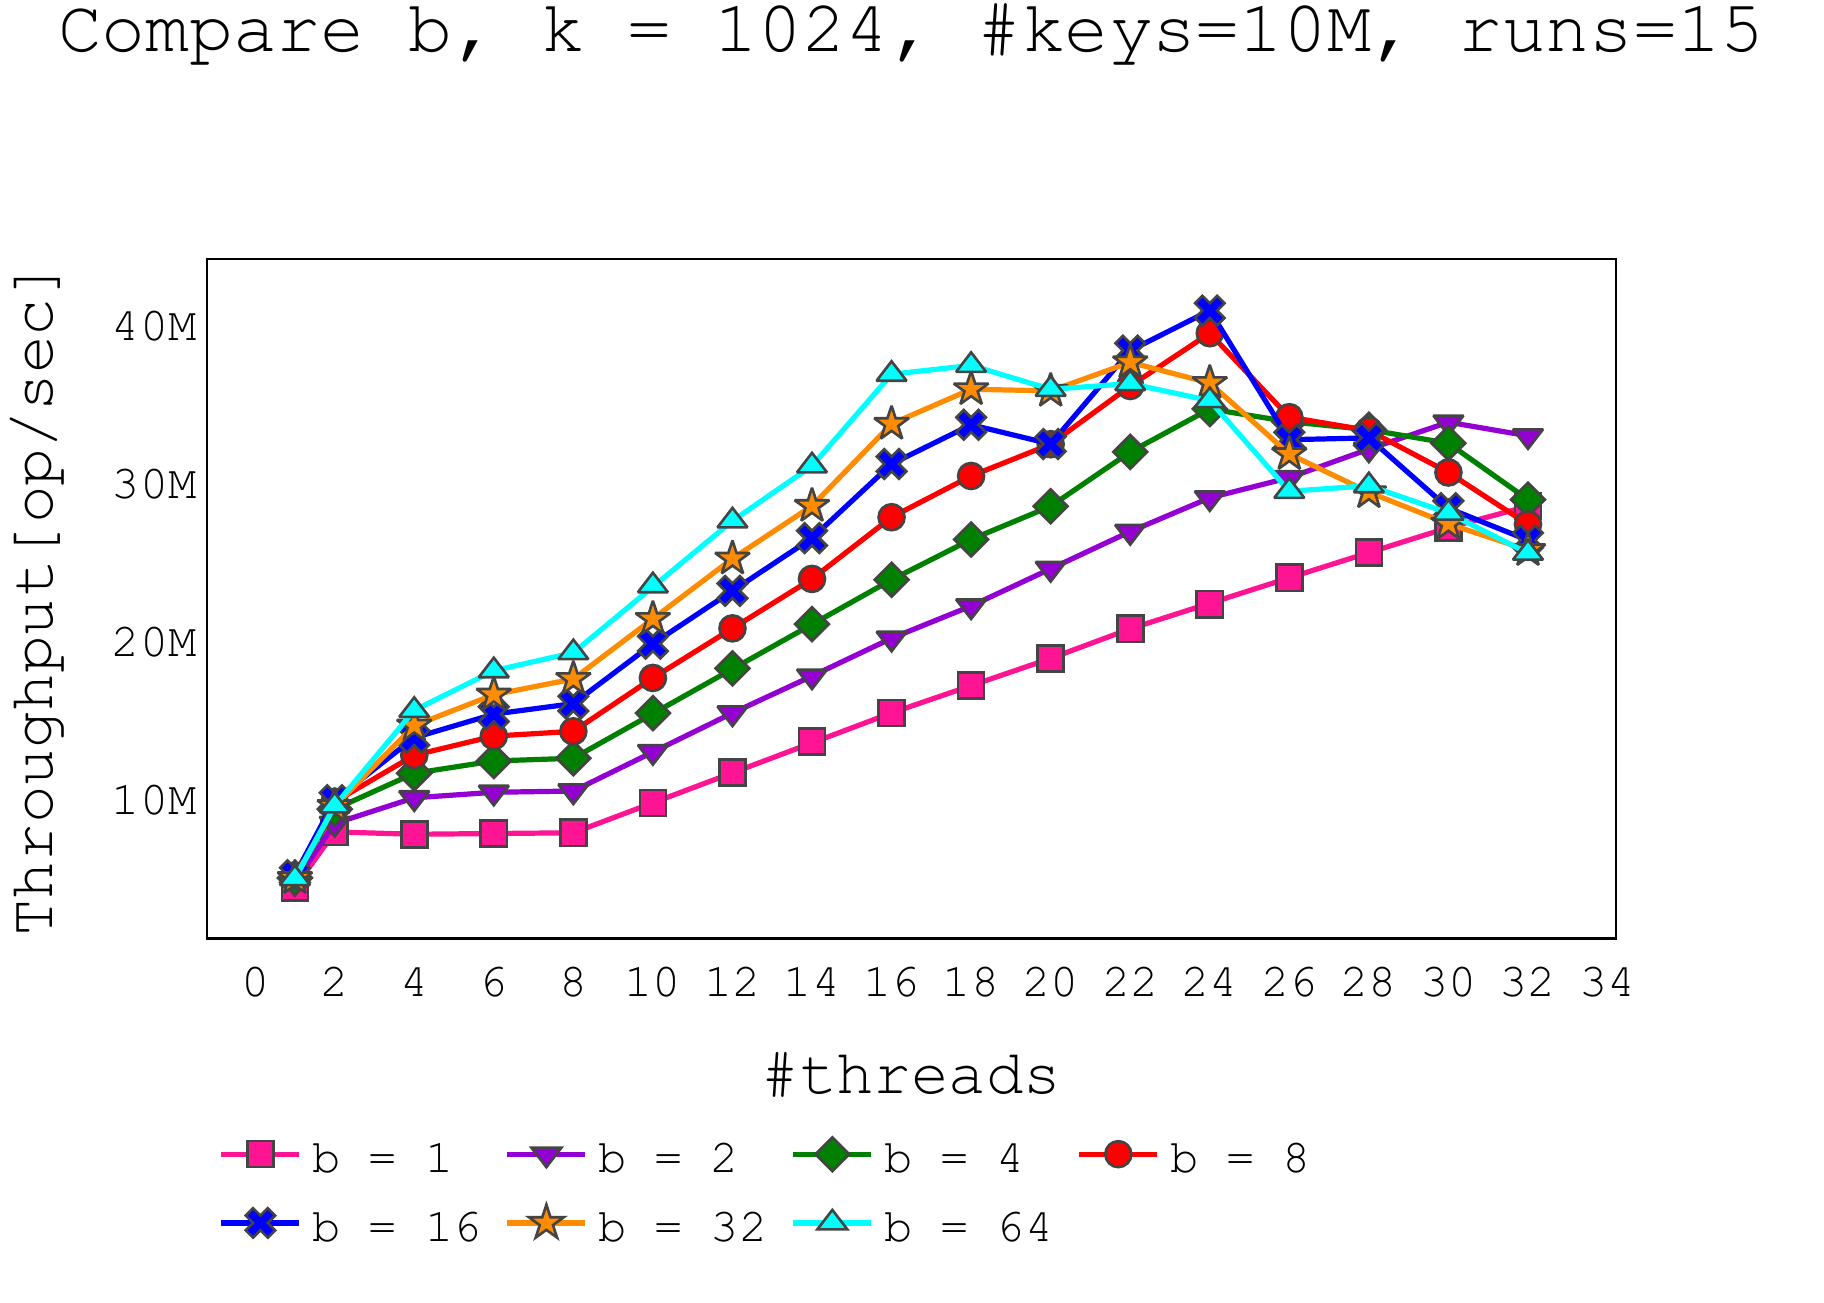}
    \caption{k = 1024, 10M elements.}
    \label{fig: compare_b_k1024_appendix}
    \end{subfigure}
    \vfill
    \begin{subfigure}[t]{0.49\textwidth}
    \includegraphics[width=\textwidth,trim={0 0.3cm 1.9cm 2.5cm},clip]{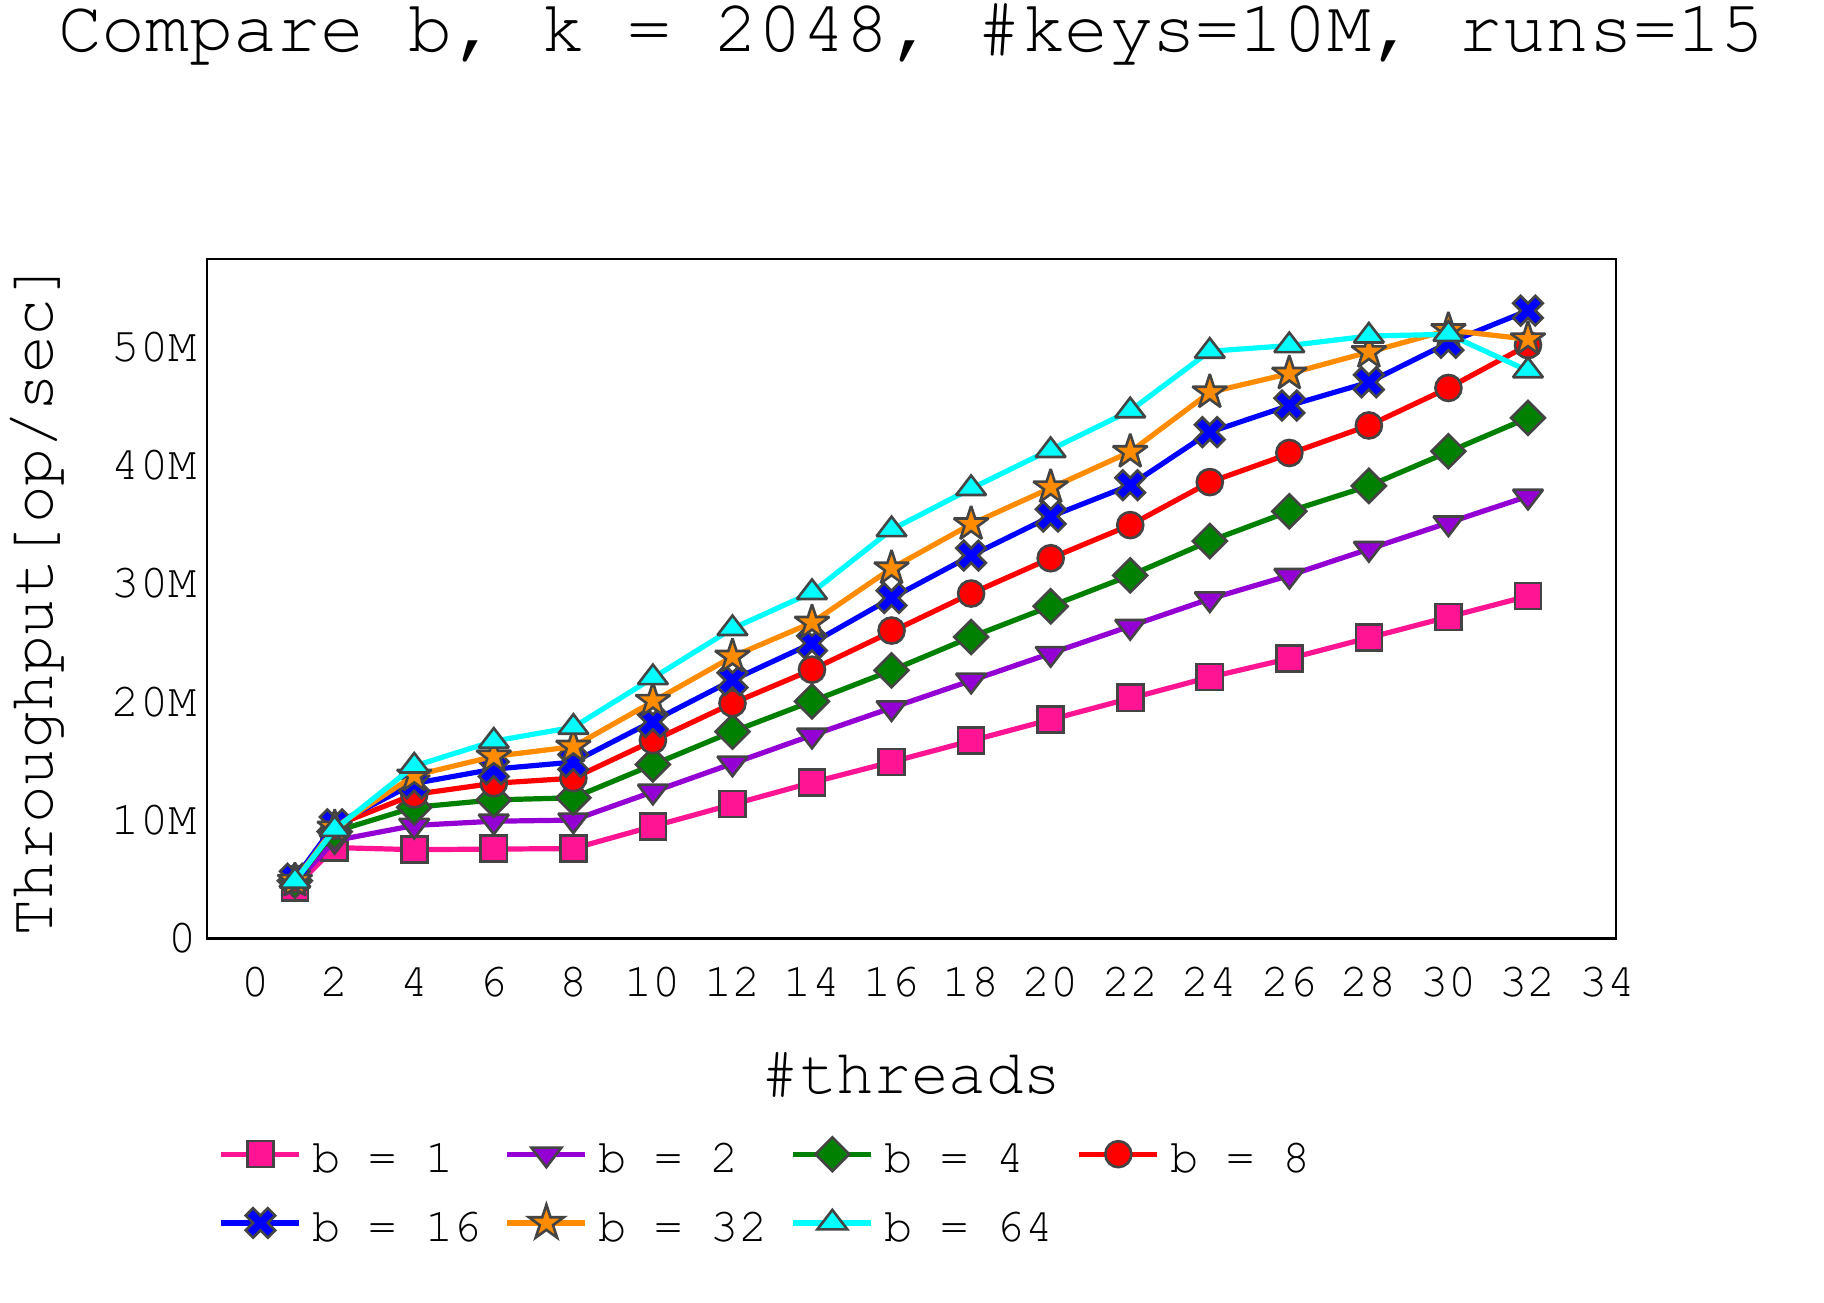}
    \caption{k = 2048, 10M elements.}
    \label{fig: compare_b_k2048_appendix}
    \end{subfigure}
    \hfill
    \begin{subfigure}[t]{0.49\textwidth}
    \includegraphics[width=\textwidth,trim={0 0.3cm 1.9cm 2.5cm},clip]{images/graphs/parameters/oracle_Quancurrent_blocking_numa_compare_b_k4096_keys10M_Tup32_runs15_03-07-2022_17-15-06.pdf}
    \caption{k = 4096, 10M elements.}
    \label{fig: compare_b_k4096_appendix}
    \end{subfigure}
    \caption{\mysketch compare b.}
    \label{fig: compare_b_appendix}
\end{figure*}
\FloatBarrier

\newpage
\subsubsection{Compare k}
\begin{figure*}[]
 \centering
    \begin{subfigure}[]{\textwidth}
    \centering
    \includegraphics[height=170pt,width=0.7\textwidth,trim={0 0.3cm 1.9cm 2.5cm},clip]{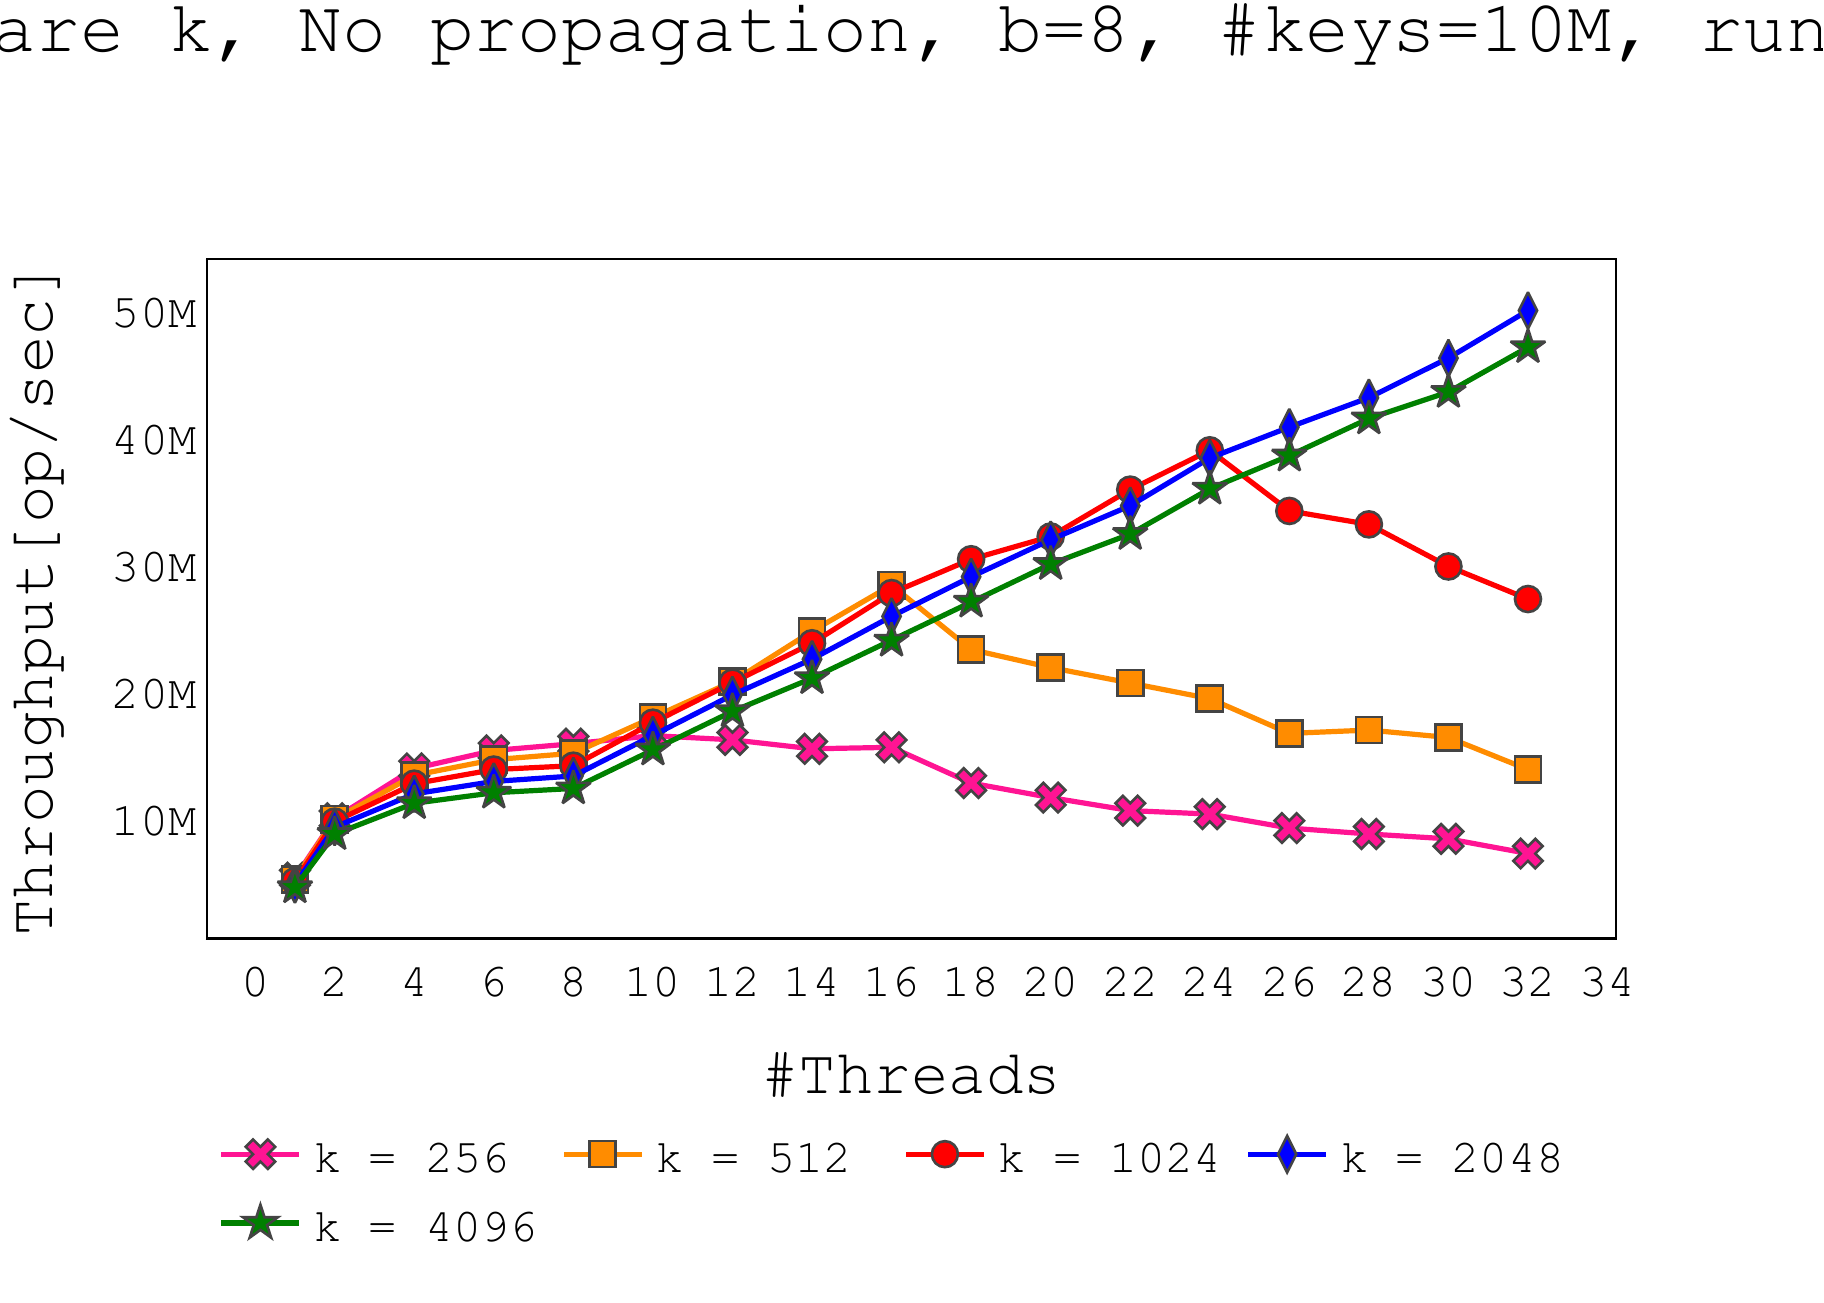}
    \caption{b = 8, 10M elements.}
    \label{fig: compare_k_b8_appendix}
    \end{subfigure}
    \vfill
    \vfill
    \begin{subfigure}[]{\textwidth}
    \centering
    \includegraphics[height=170pt, width=0.7\textwidth,trim={0 0.3cm 1.9cm 2.5cm},clip]{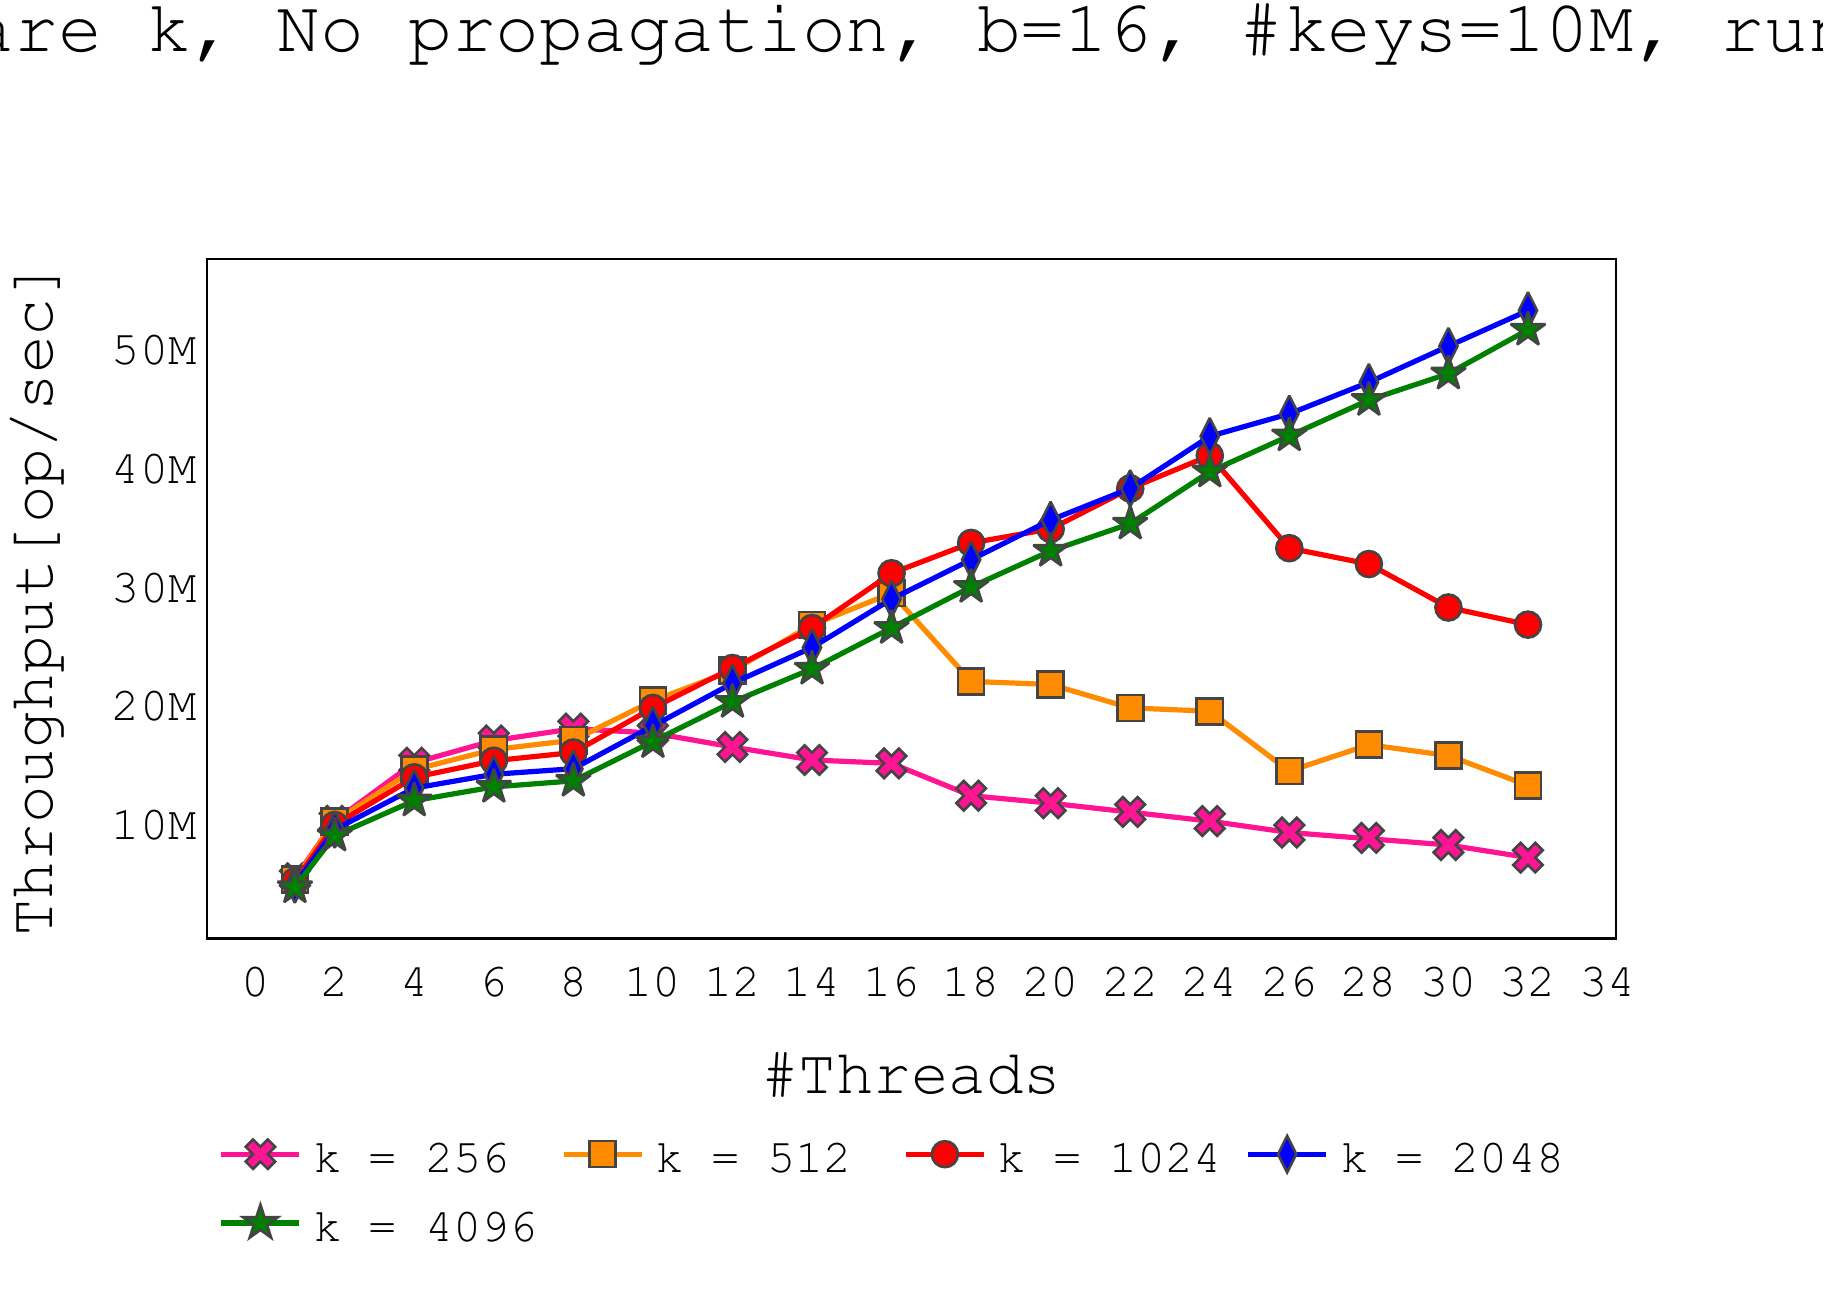}
    \caption{b = 16, 10M elements.}
    \label{fig: compare_k_b16_appendix}
    \end{subfigure}
    \vfill
    \vfill
    \begin{subfigure}[]{\textwidth}
    \centering
    \includegraphics[height=170pt, width=0.7\textwidth,trim={0 0.3cm 1.9cm 2.5cm},clip]{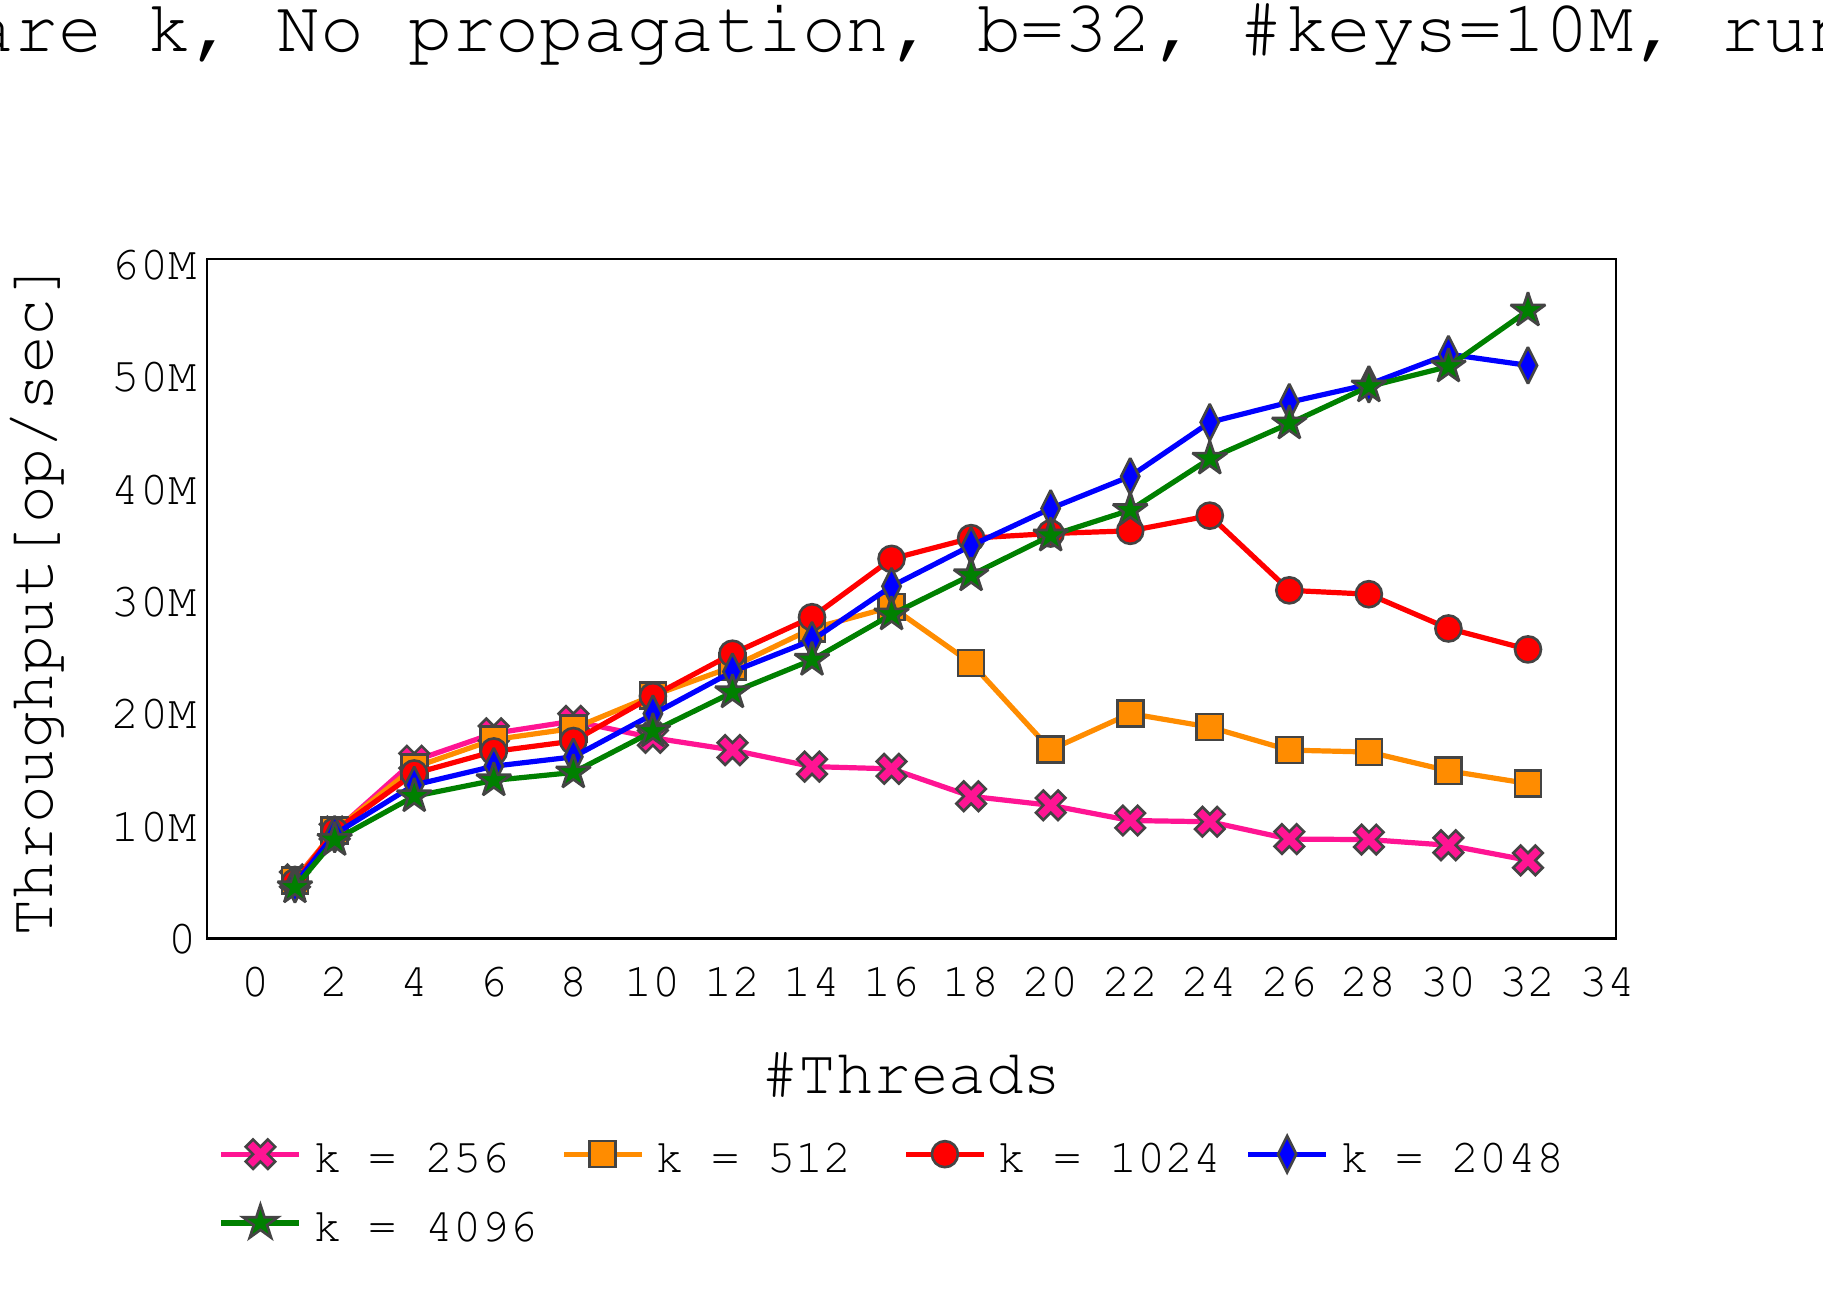}
    \caption{b = 32, 10M elements.}
    \label{fig: compare_k_b16_appendix}
    \end{subfigure}
   
    \caption{\mysketch compare k.}
    \label{fig: compare_k_appendix}
\end{figure*}
\FloatBarrier

\newpage
\subsubsection{Compare Rho}
\begin{figure*}[]
 \centering
    \begin{subfigure}[]{\textwidth}
    \centering
    \includegraphics[height=170pt,width=0.5\textwidth,trim={0 0cm 1.2cm 2cm},clip] {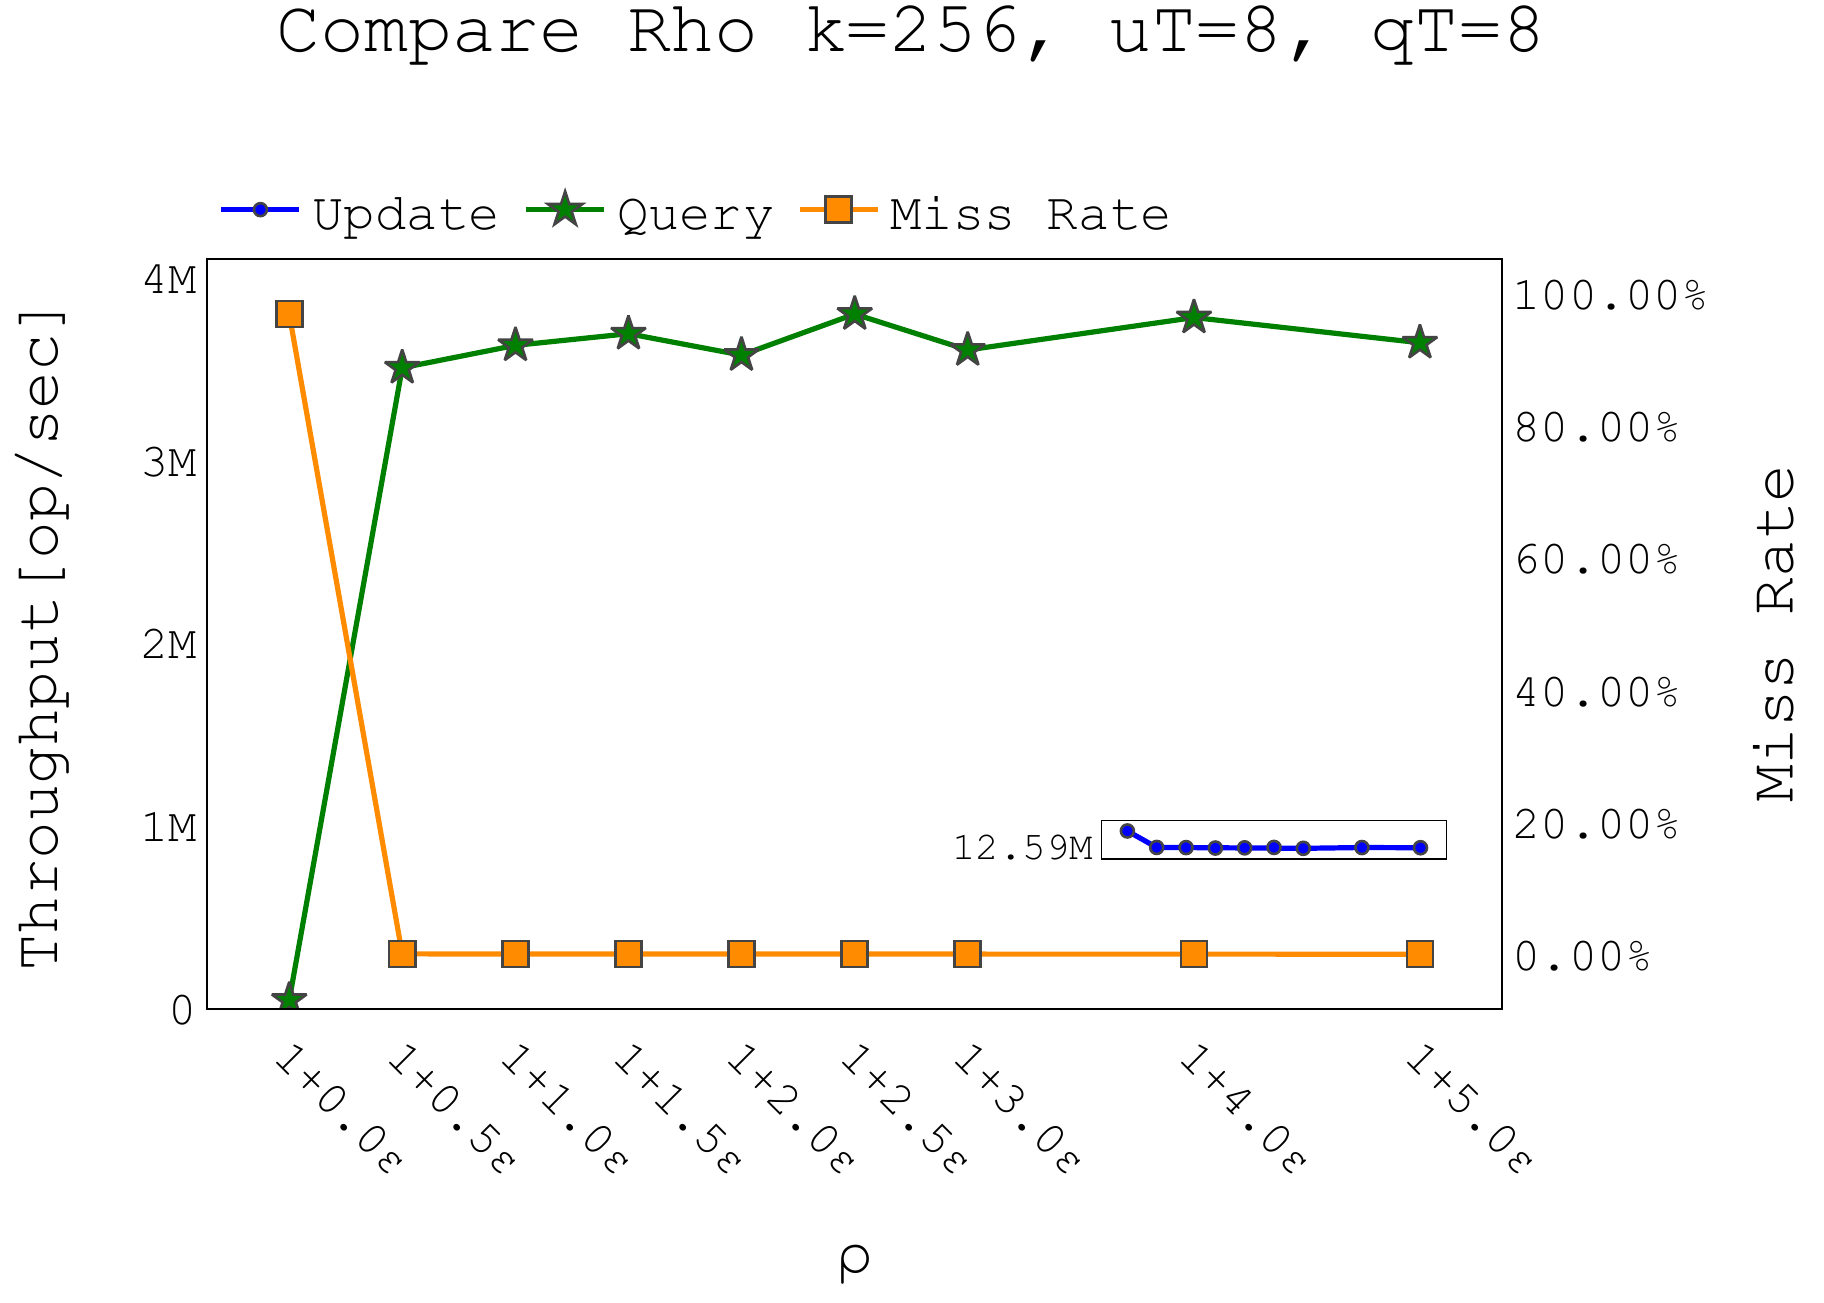}
    \caption{8 update threads, 8 query threads, 10M elements.}
    \label{fig: compare_rho_k256_8-8_appendix}
    \end{subfigure}
    \vfill
    \vfill
    \begin{subfigure}[]{\textwidth}
    \centering
    \includegraphics[height=170pt,width=0.5\textwidth,trim={0 0cm 1.2cm 2cm},clip] {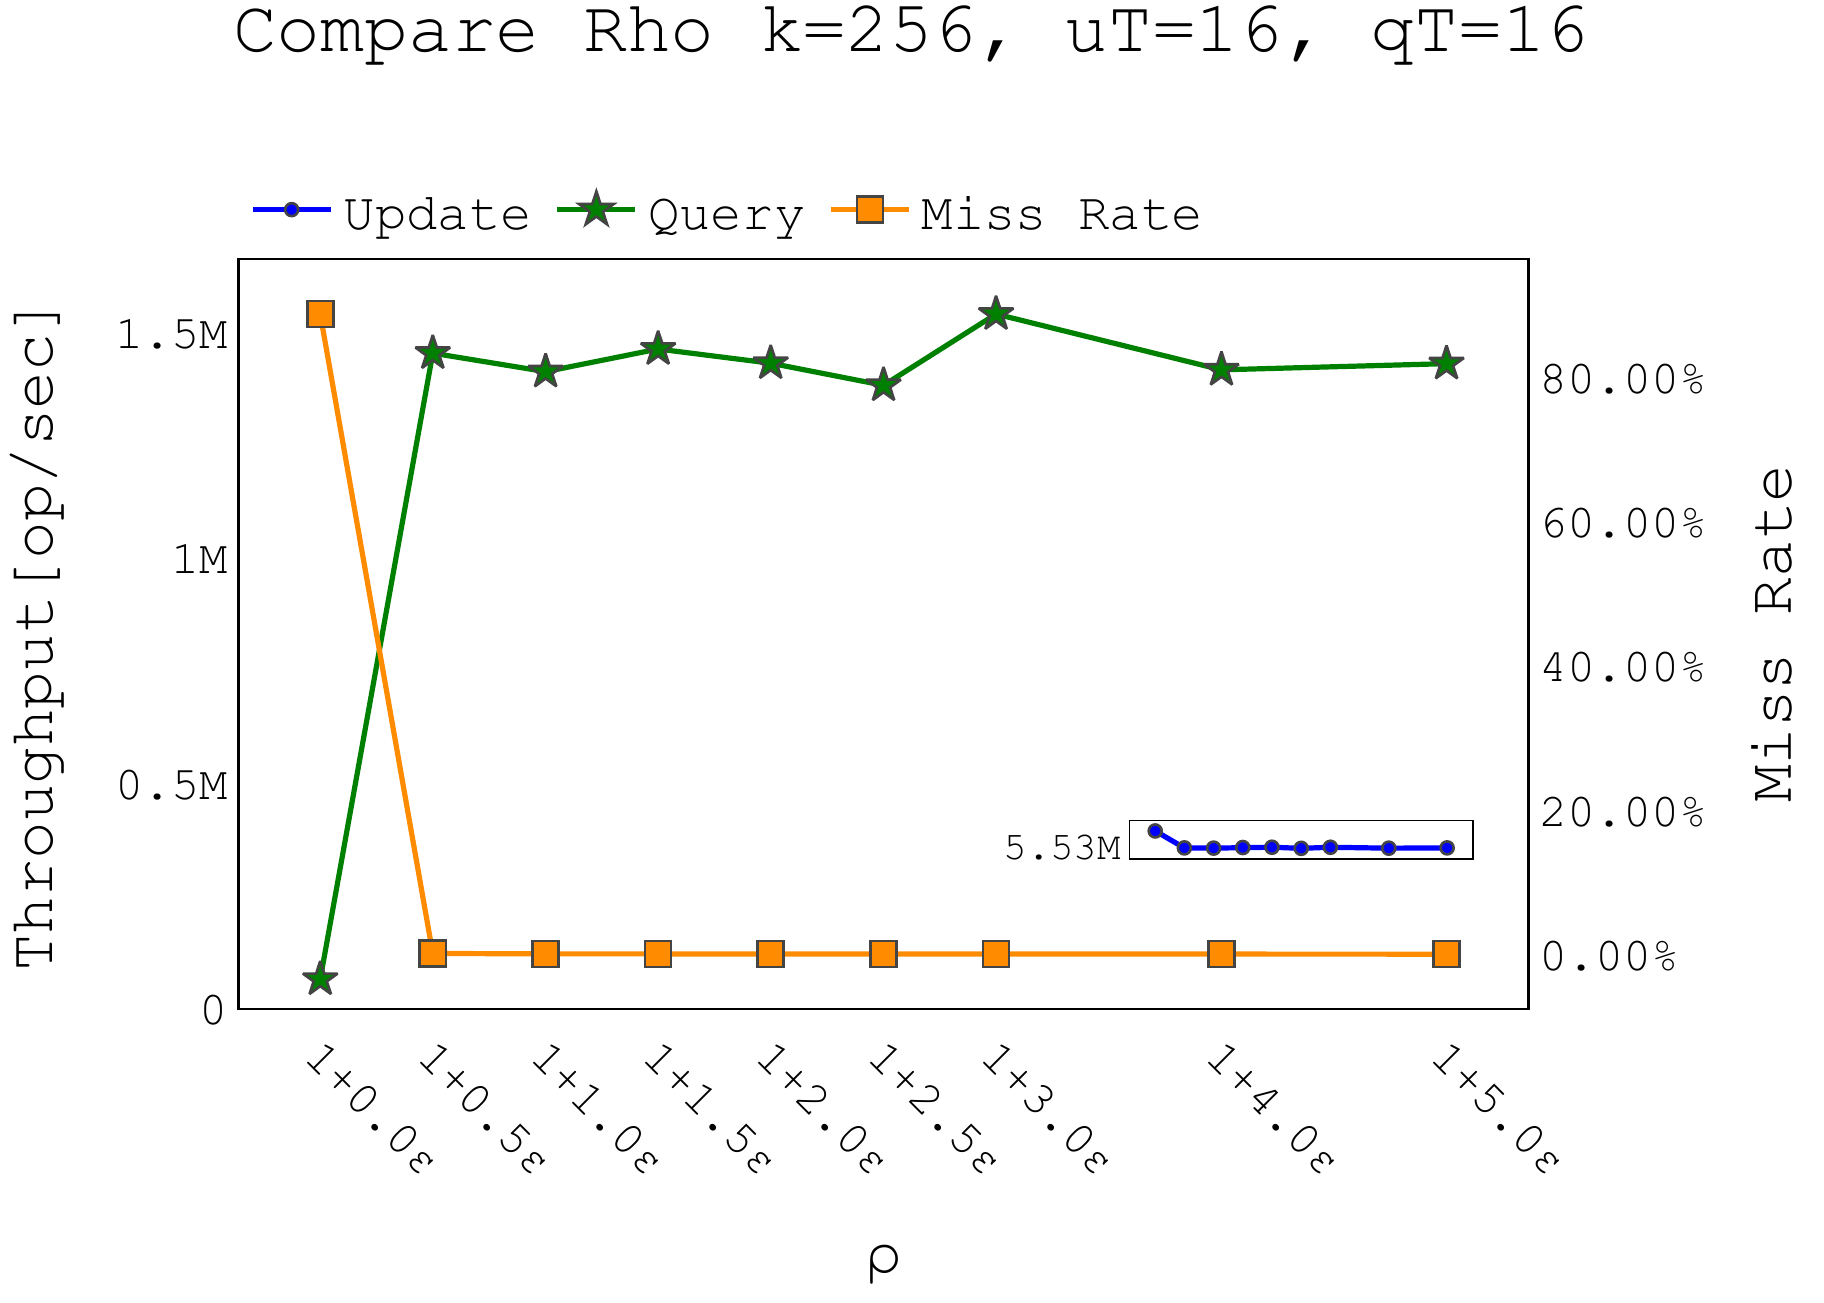}
    \caption{16 update threads, 16 query threads, 10M elements.}
    \label{fig: compare_rho_k256_16-16_appendix}
    \end{subfigure}
    \vfill
    \vfill
    \begin{subfigure}[]{\textwidth}
    \centering
    \includegraphics[height=170pt,width=0.5\textwidth,trim={0 0cm 1.2cm 2cm},clip] {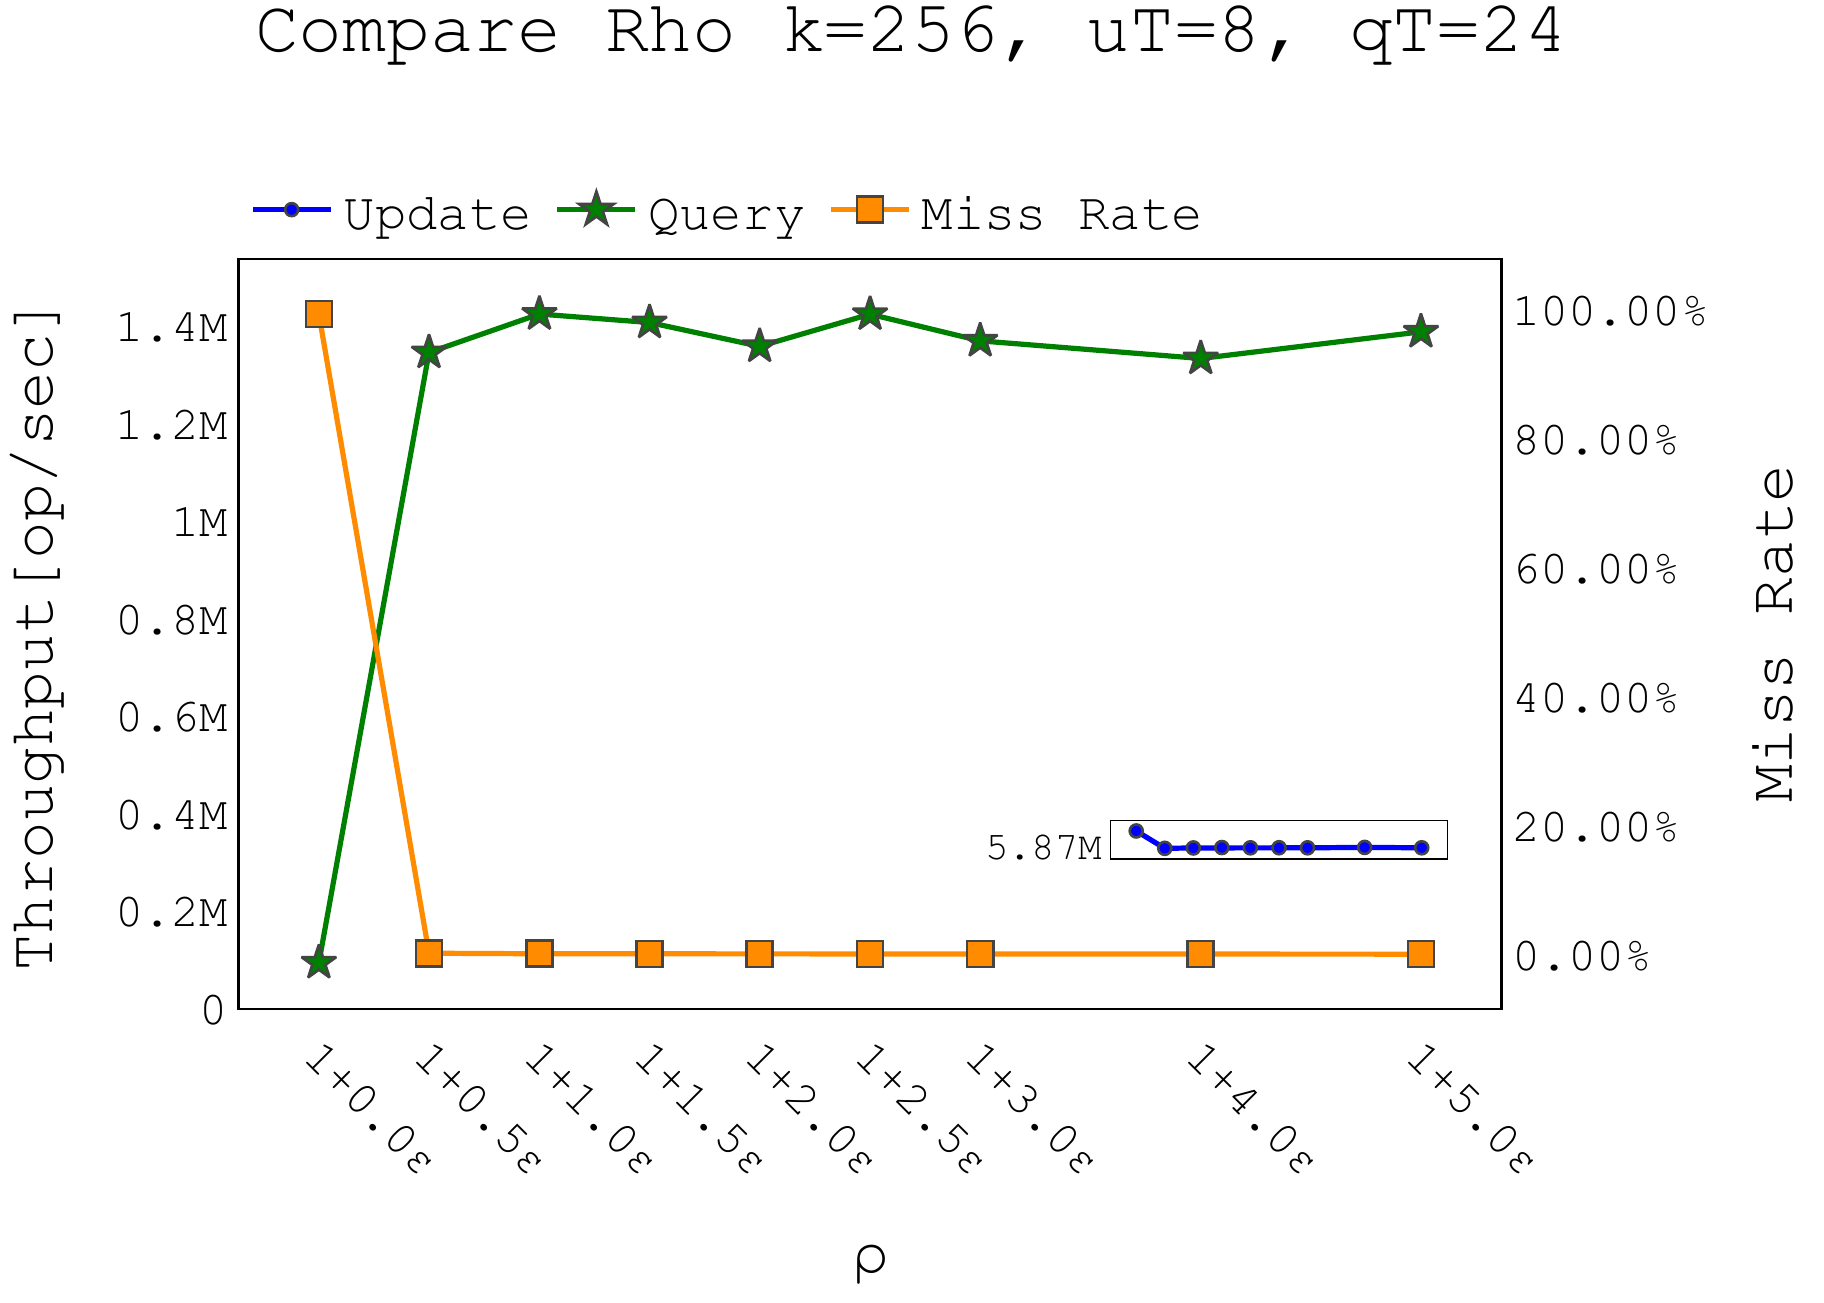}
    \caption{8 update threads, 24 query threads, 10M elements.}
    \label{fig: compare_rho_k256_8-24_appendix}
    \end{subfigure}
   
    \caption{\mysketch compare rho, k = 256.}
    \label{fig: compare_rho_k256_appendix}
\end{figure*}
\FloatBarrier

\newpage
\begin{figure*}[]
 \centering
    \begin{subfigure}[]{\textwidth}
    \centering
    \includegraphics[height=170pt,width=0.5\textwidth,trim={0 0cm 1.2cm 2cm},clip] {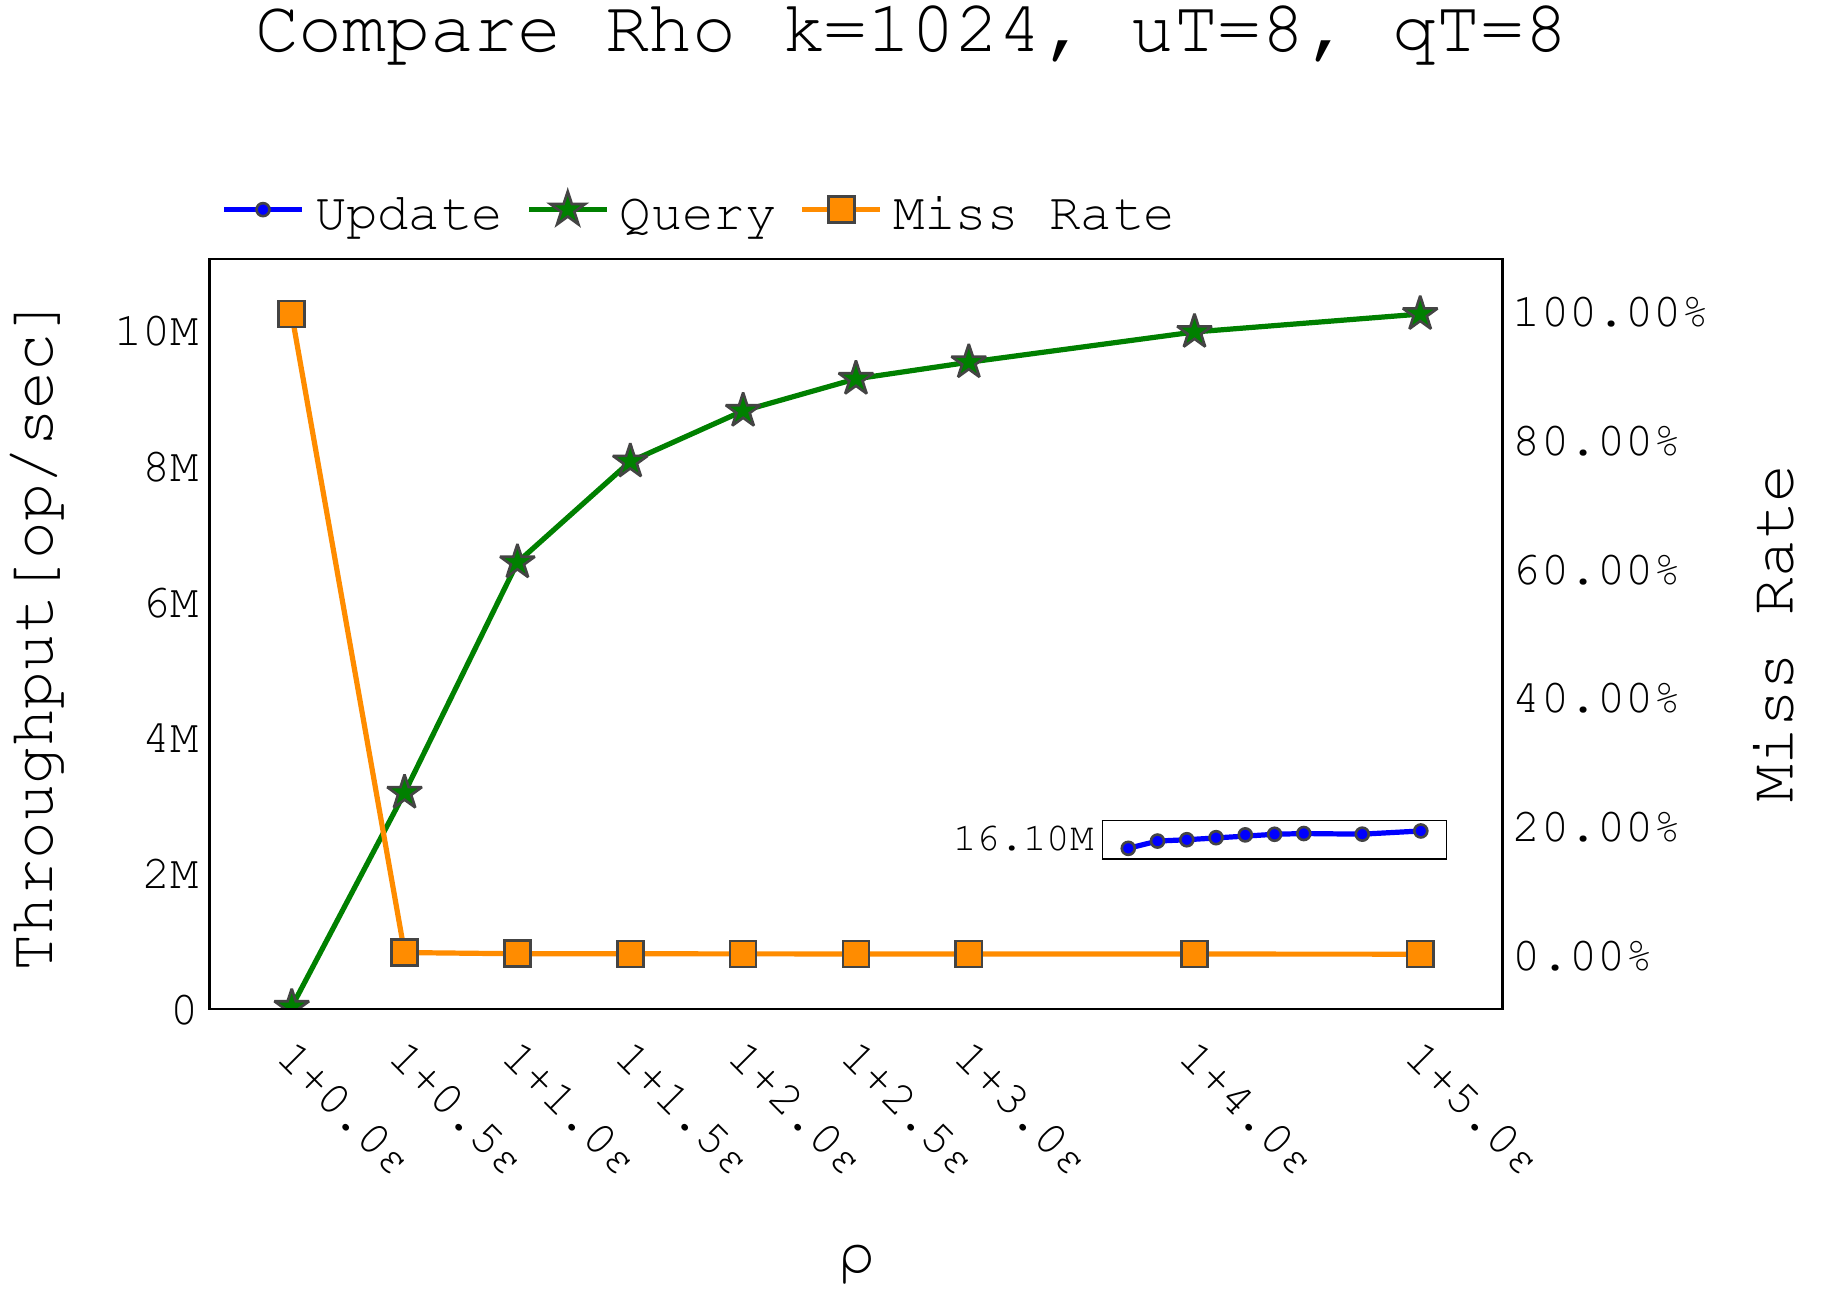}
    \caption{8 update threads, 8 query threads, 10M elements.}
    \label{fig: compare_rho_k1024_8-8_appendix}
    \end{subfigure}
    \vfill
    \vfill
    \begin{subfigure}[]{\textwidth}
    \centering
    \includegraphics[height=170pt,width=0.5\textwidth,trim={0 0cm 1.2cm 2cm},clip] {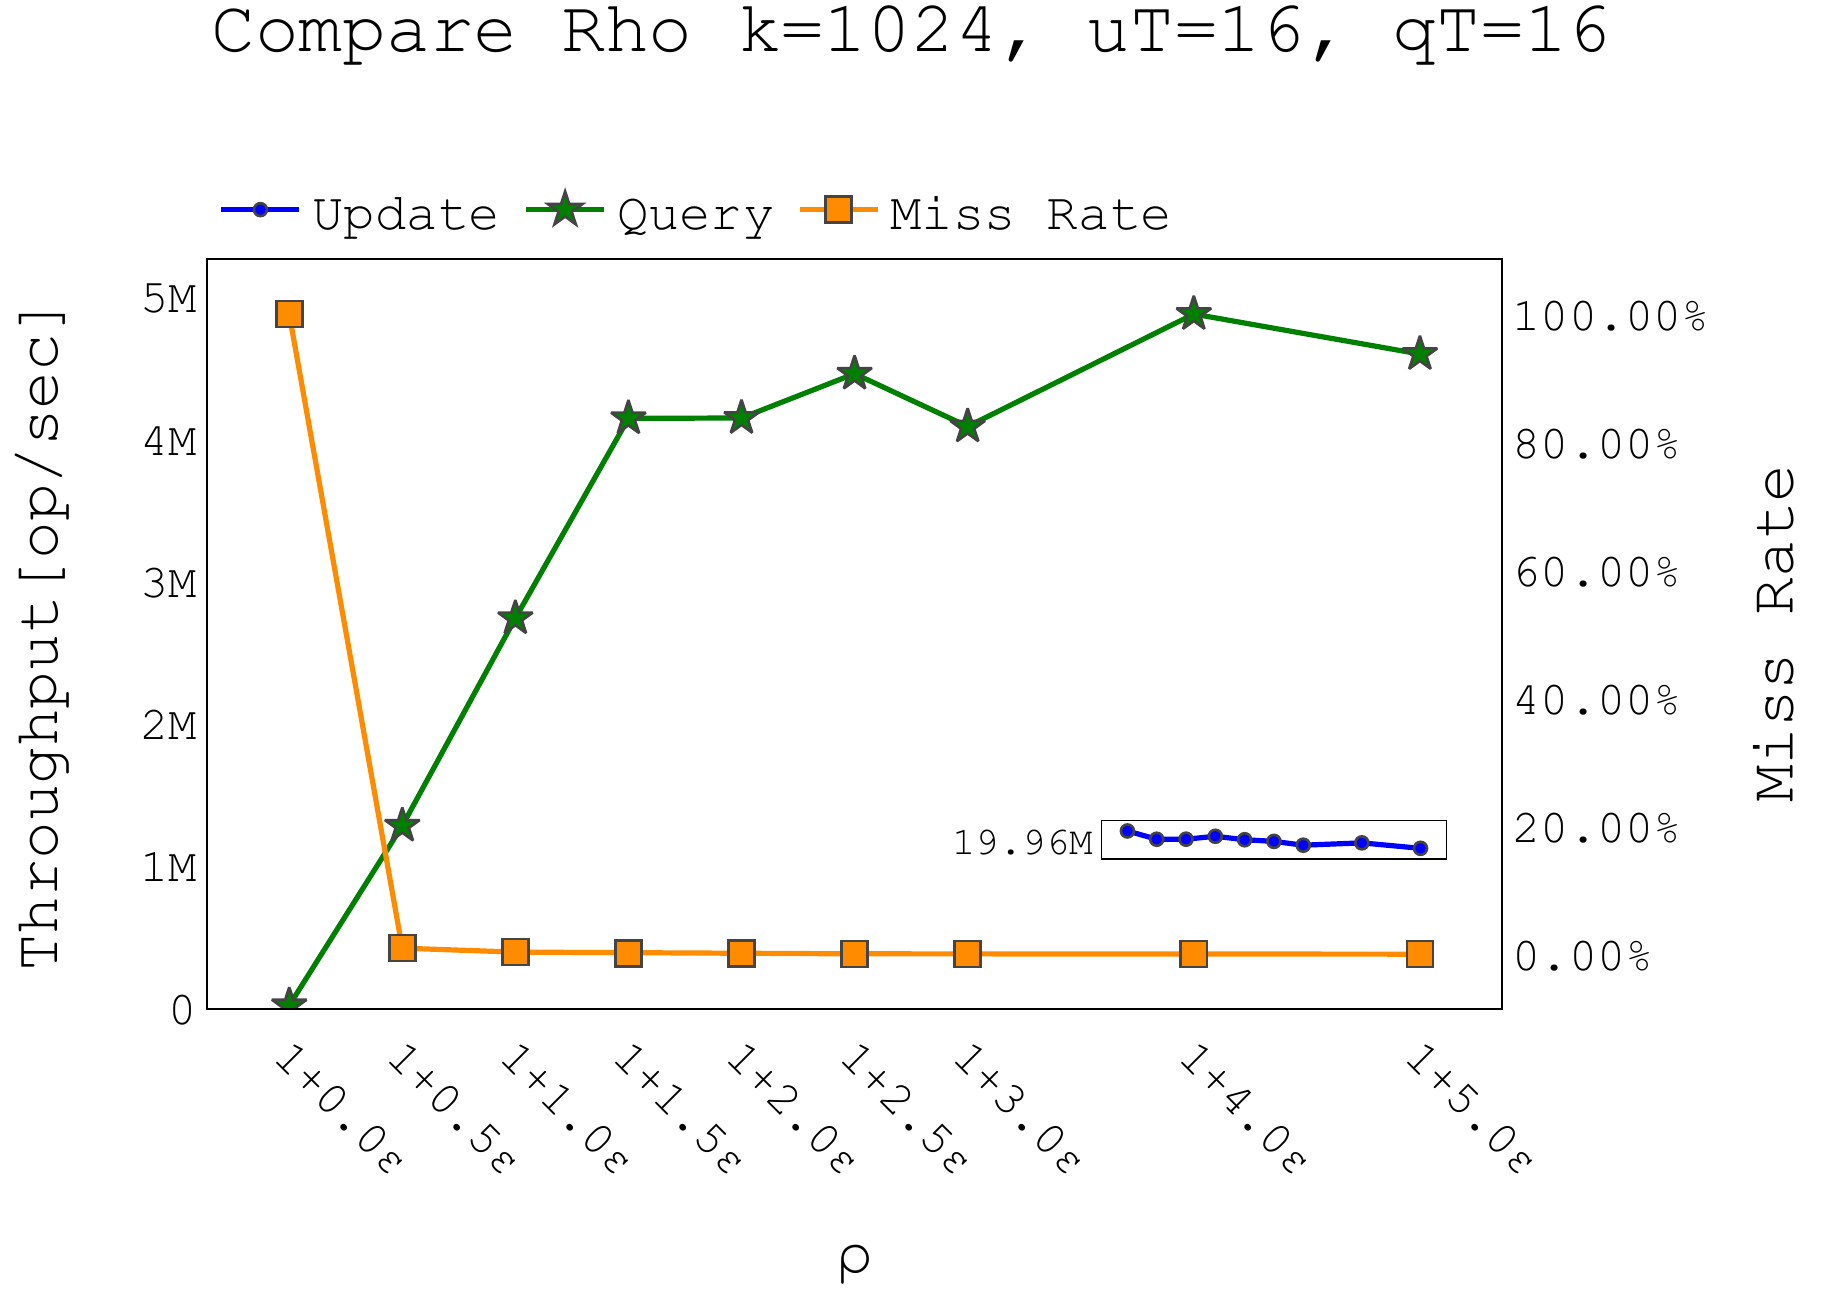}
    \caption{16 update threads, 16 query threads, 10M elements.}
    \label{fig: compare_rho_k1024_16-16_appendix}
    \end{subfigure}
    \vfill
    \vfill
    \begin{subfigure}[]{\textwidth}
    \centering
    \includegraphics[height=170pt,width=0.5\textwidth,trim={0 0cm 1.2cm 2cm},clip] {images/graphs/parameters/oracle_Quancurrent_compare_rho_blocking_numa_k1024_b16_runs15_pre10M_pT1_keys10M_uT8_qT24_05-07-2022_16-30-12.pdf}
    \caption{8 update threads, 24 query threads, 10M elements.}
    \label{fig: compare_rho_k1024_8-24_appendix}
    \end{subfigure}
   
    \caption{\mysketch compare rho, k = 1024.}
    \label{fig: compare_rho_k1024_appendix}
\end{figure*}
\FloatBarrier

\newpage
\begin{figure*}[]
 \centering
    \begin{subfigure}[]{\textwidth}
    \centering
    \includegraphics[height=170pt,width=0.5\textwidth,trim={0 0cm 1.2cm 2cm},clip] {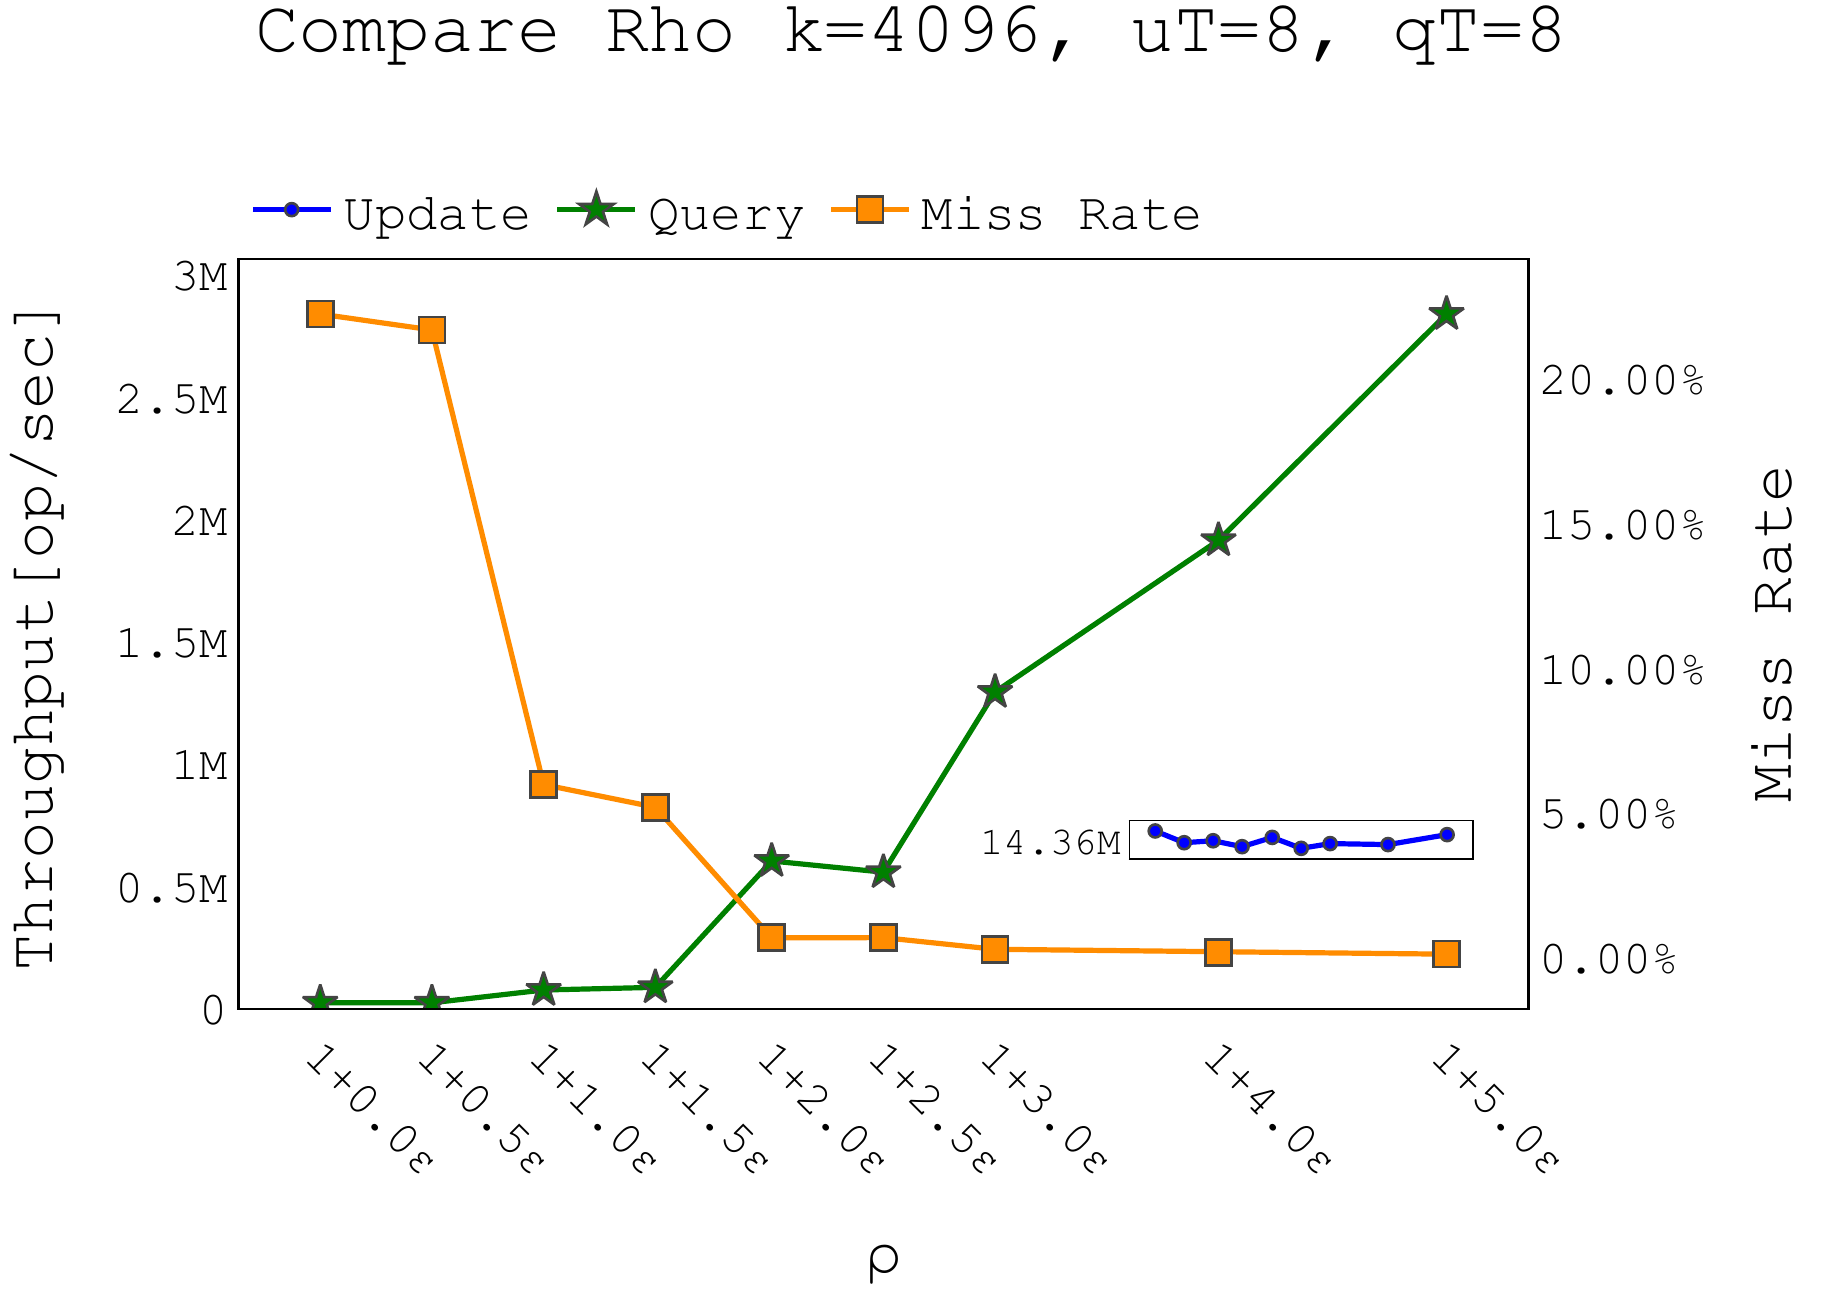}
    \caption{8 update threads, 8 query threads, 10M elements.}
    \label{fig: compare_rho_k4096_8-8_appendix}
    \end{subfigure}
    \vfill
    \vfill
    \begin{subfigure}[]{\textwidth}
    \centering
    \includegraphics[height=170pt,width=0.5\textwidth,trim={0 0cm 1.2cm 2cm},clip] {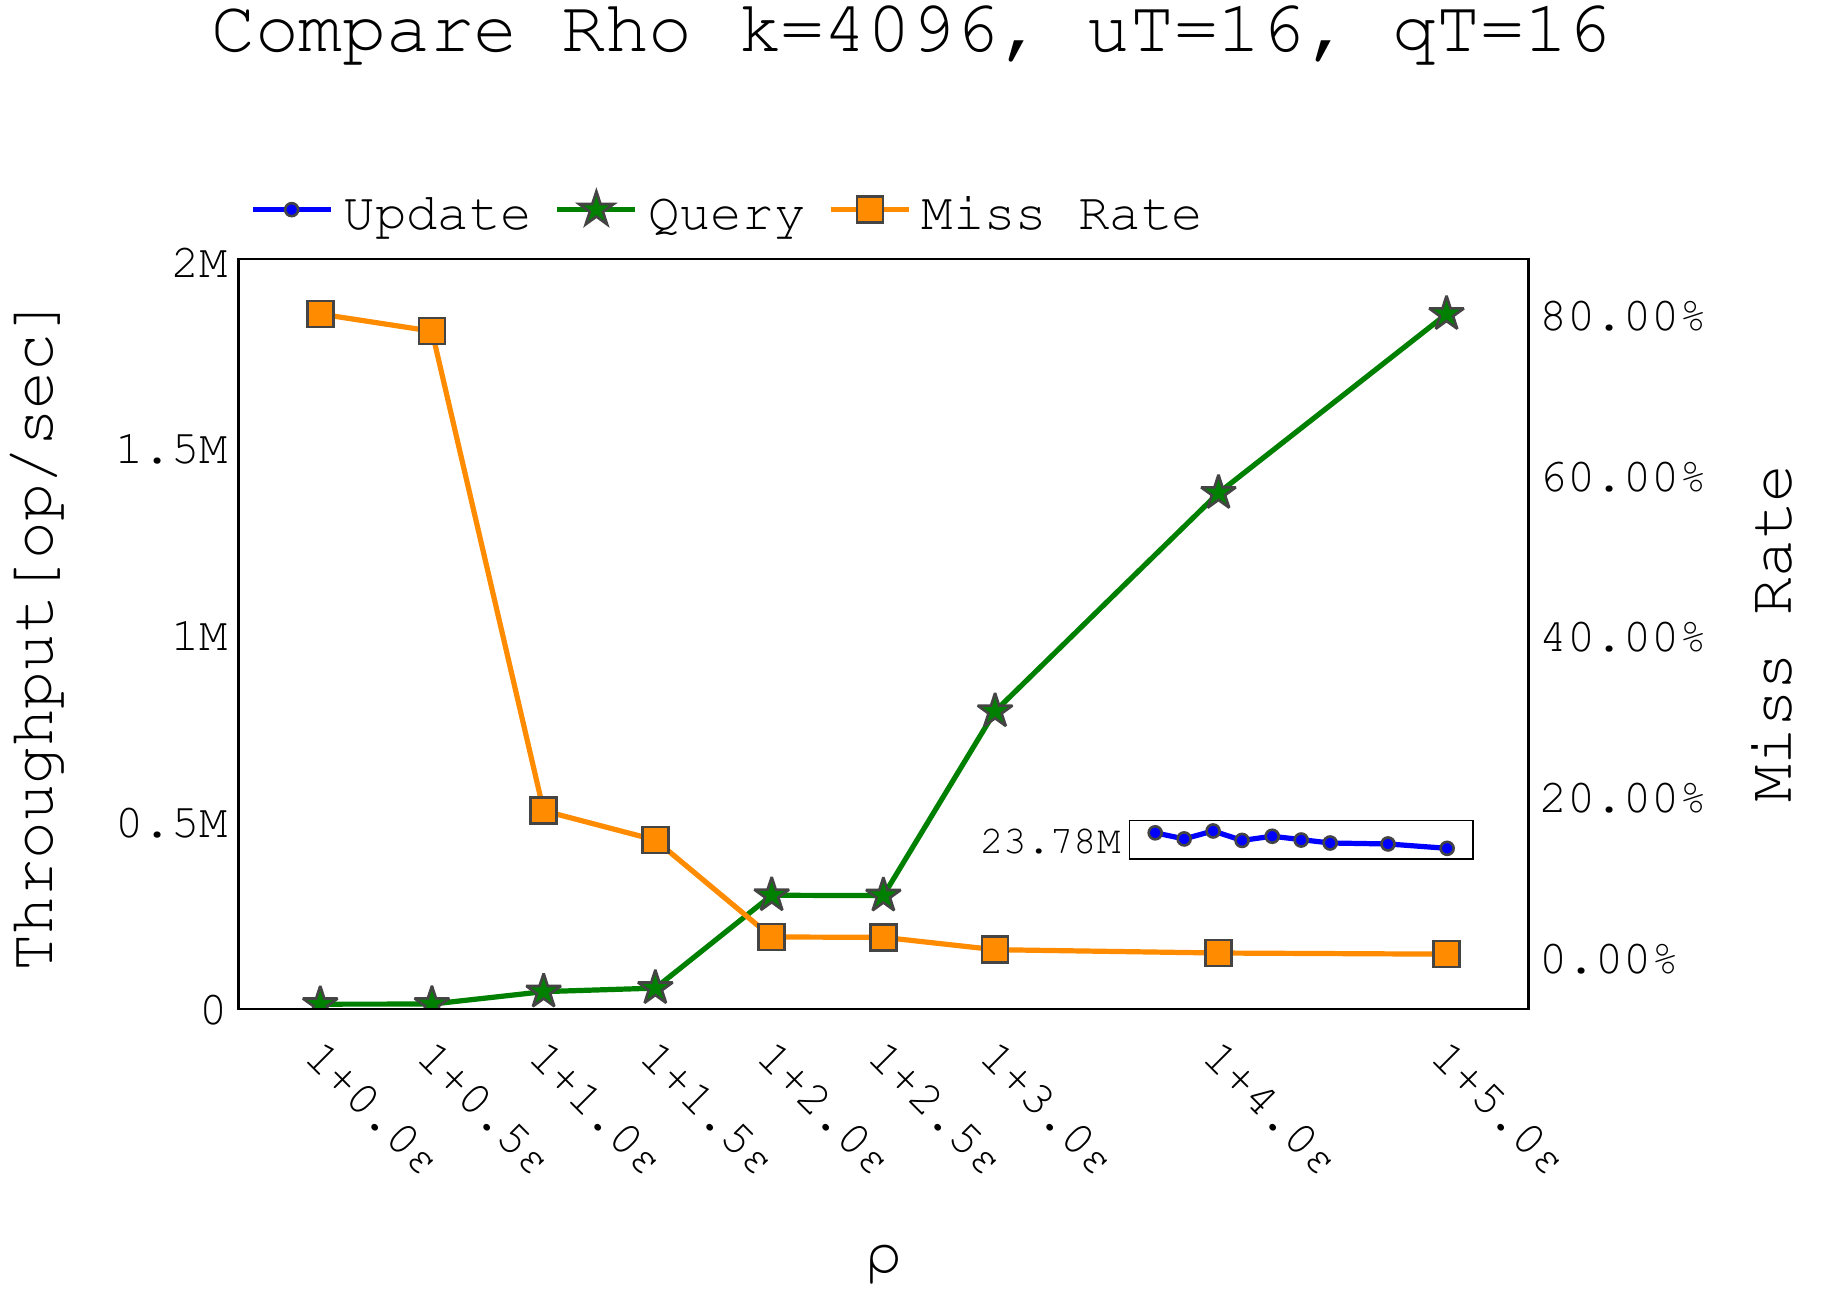}
    \caption{16 update threads, 16 query threads, 10M elements.}
    \label{fig: compare_rho_k4096_16-16_appendix}
    \end{subfigure}
    \vfill
    \vfill
    \begin{subfigure}[]{\textwidth}
    \centering
    \includegraphics[height=170pt,width=0.5\textwidth,trim={0 0cm 1.2cm 2cm},clip] {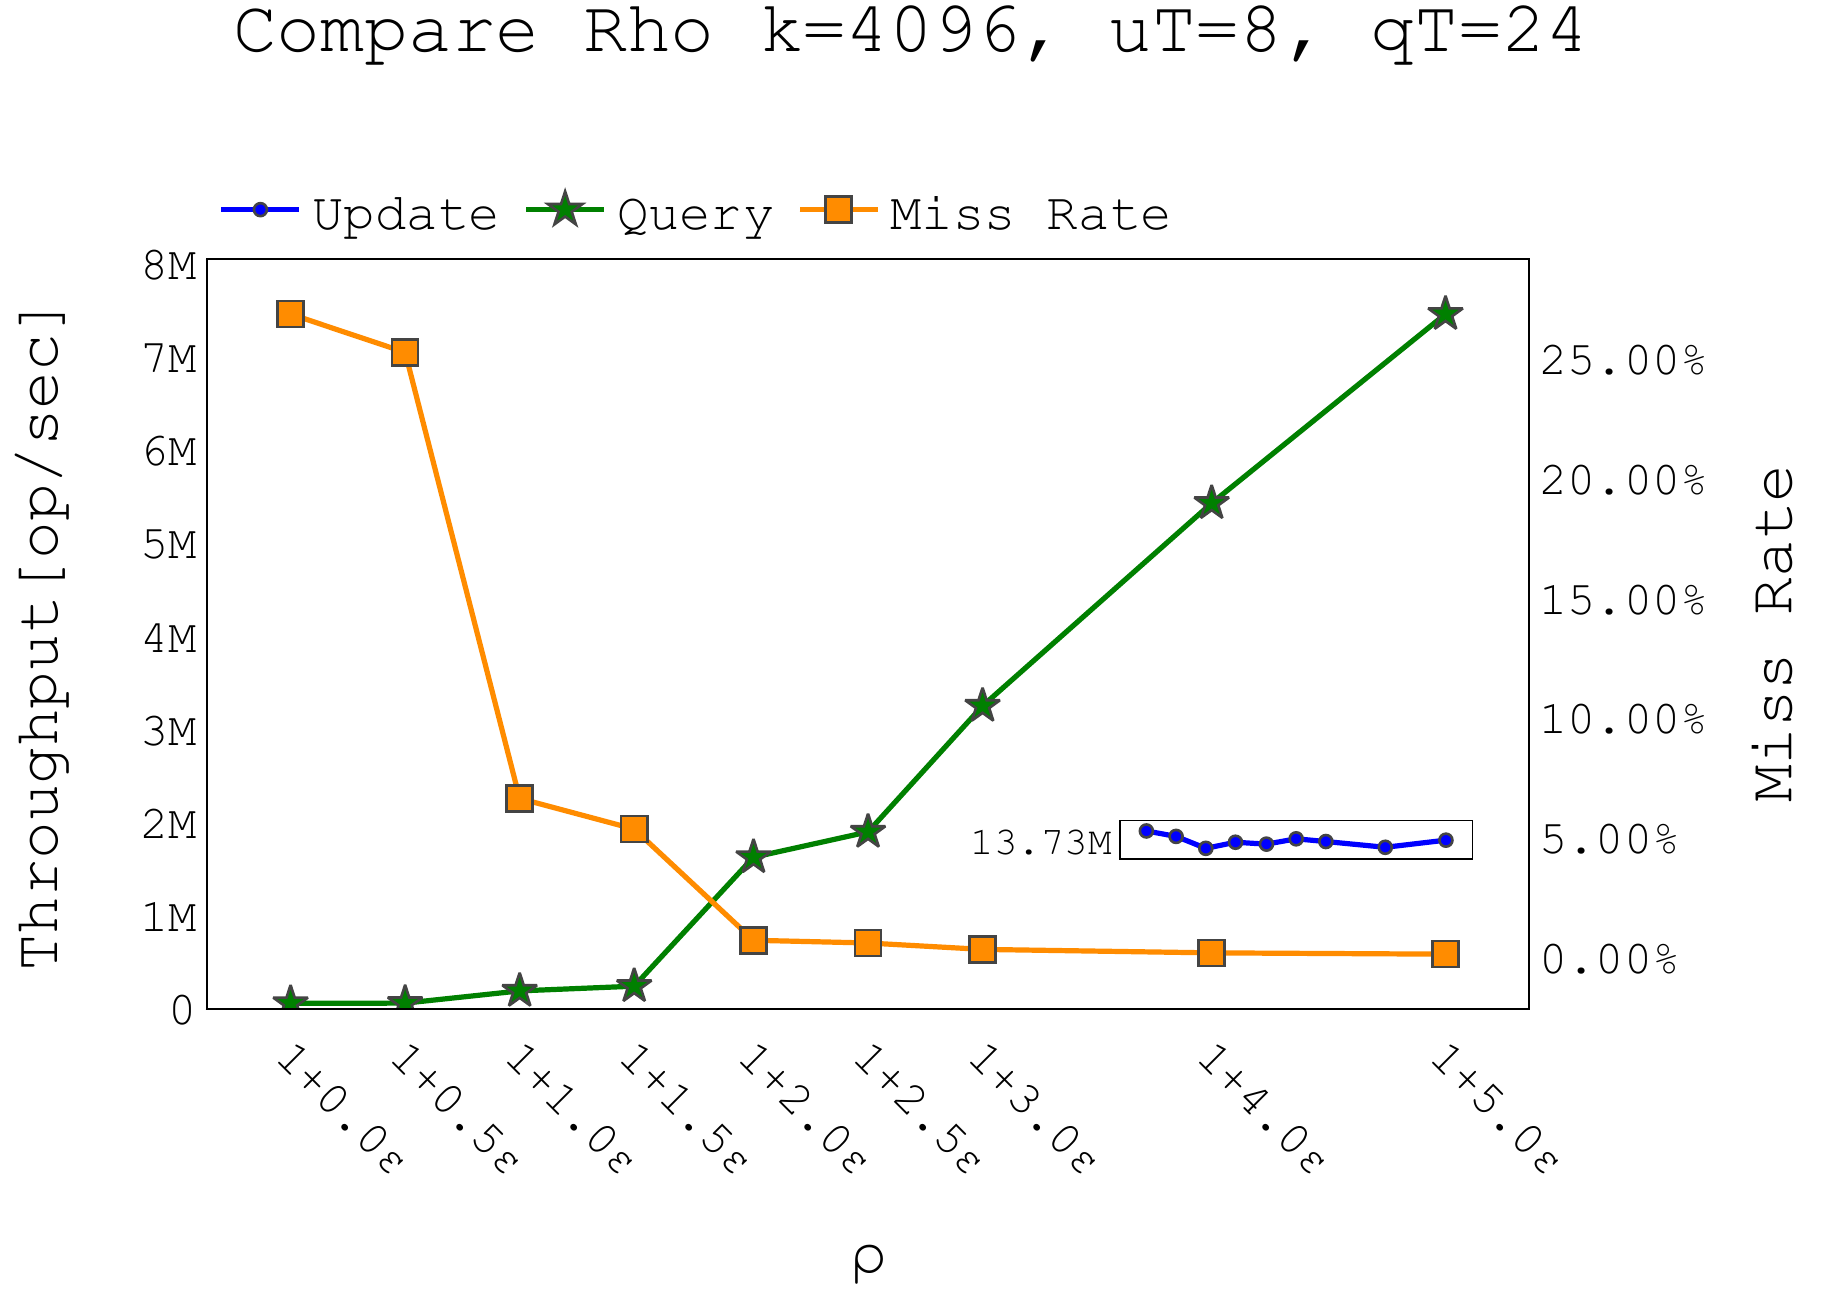}
    \caption{8 update threads, 24 query threads, 10M elements.}
    \label{fig: compare_rho_k4096_8-24_appendix}
    \end{subfigure}
   
    \caption{\mysketch compare rho, k = 4096.}
    \label{fig: compare_rho_k4096_appendix}
\end{figure*}
\FloatBarrier
