# Supplementary material for: Quancurrent: A Concurrent Quantiles Sketch
Source: arXiv:2208.09265 source file (2022-08-19)
Supplement: Supplementary file 3 [file QuancurrentVsFCDS.tex]

\subsubsection{k = 4096}
\FloatBarrier
\begin{figure}[b]
    \centering
    \includegraphics[width=\columnwidth,trim={0.1cm 0.2cm 1.9cm 0.1cm},clip]
    {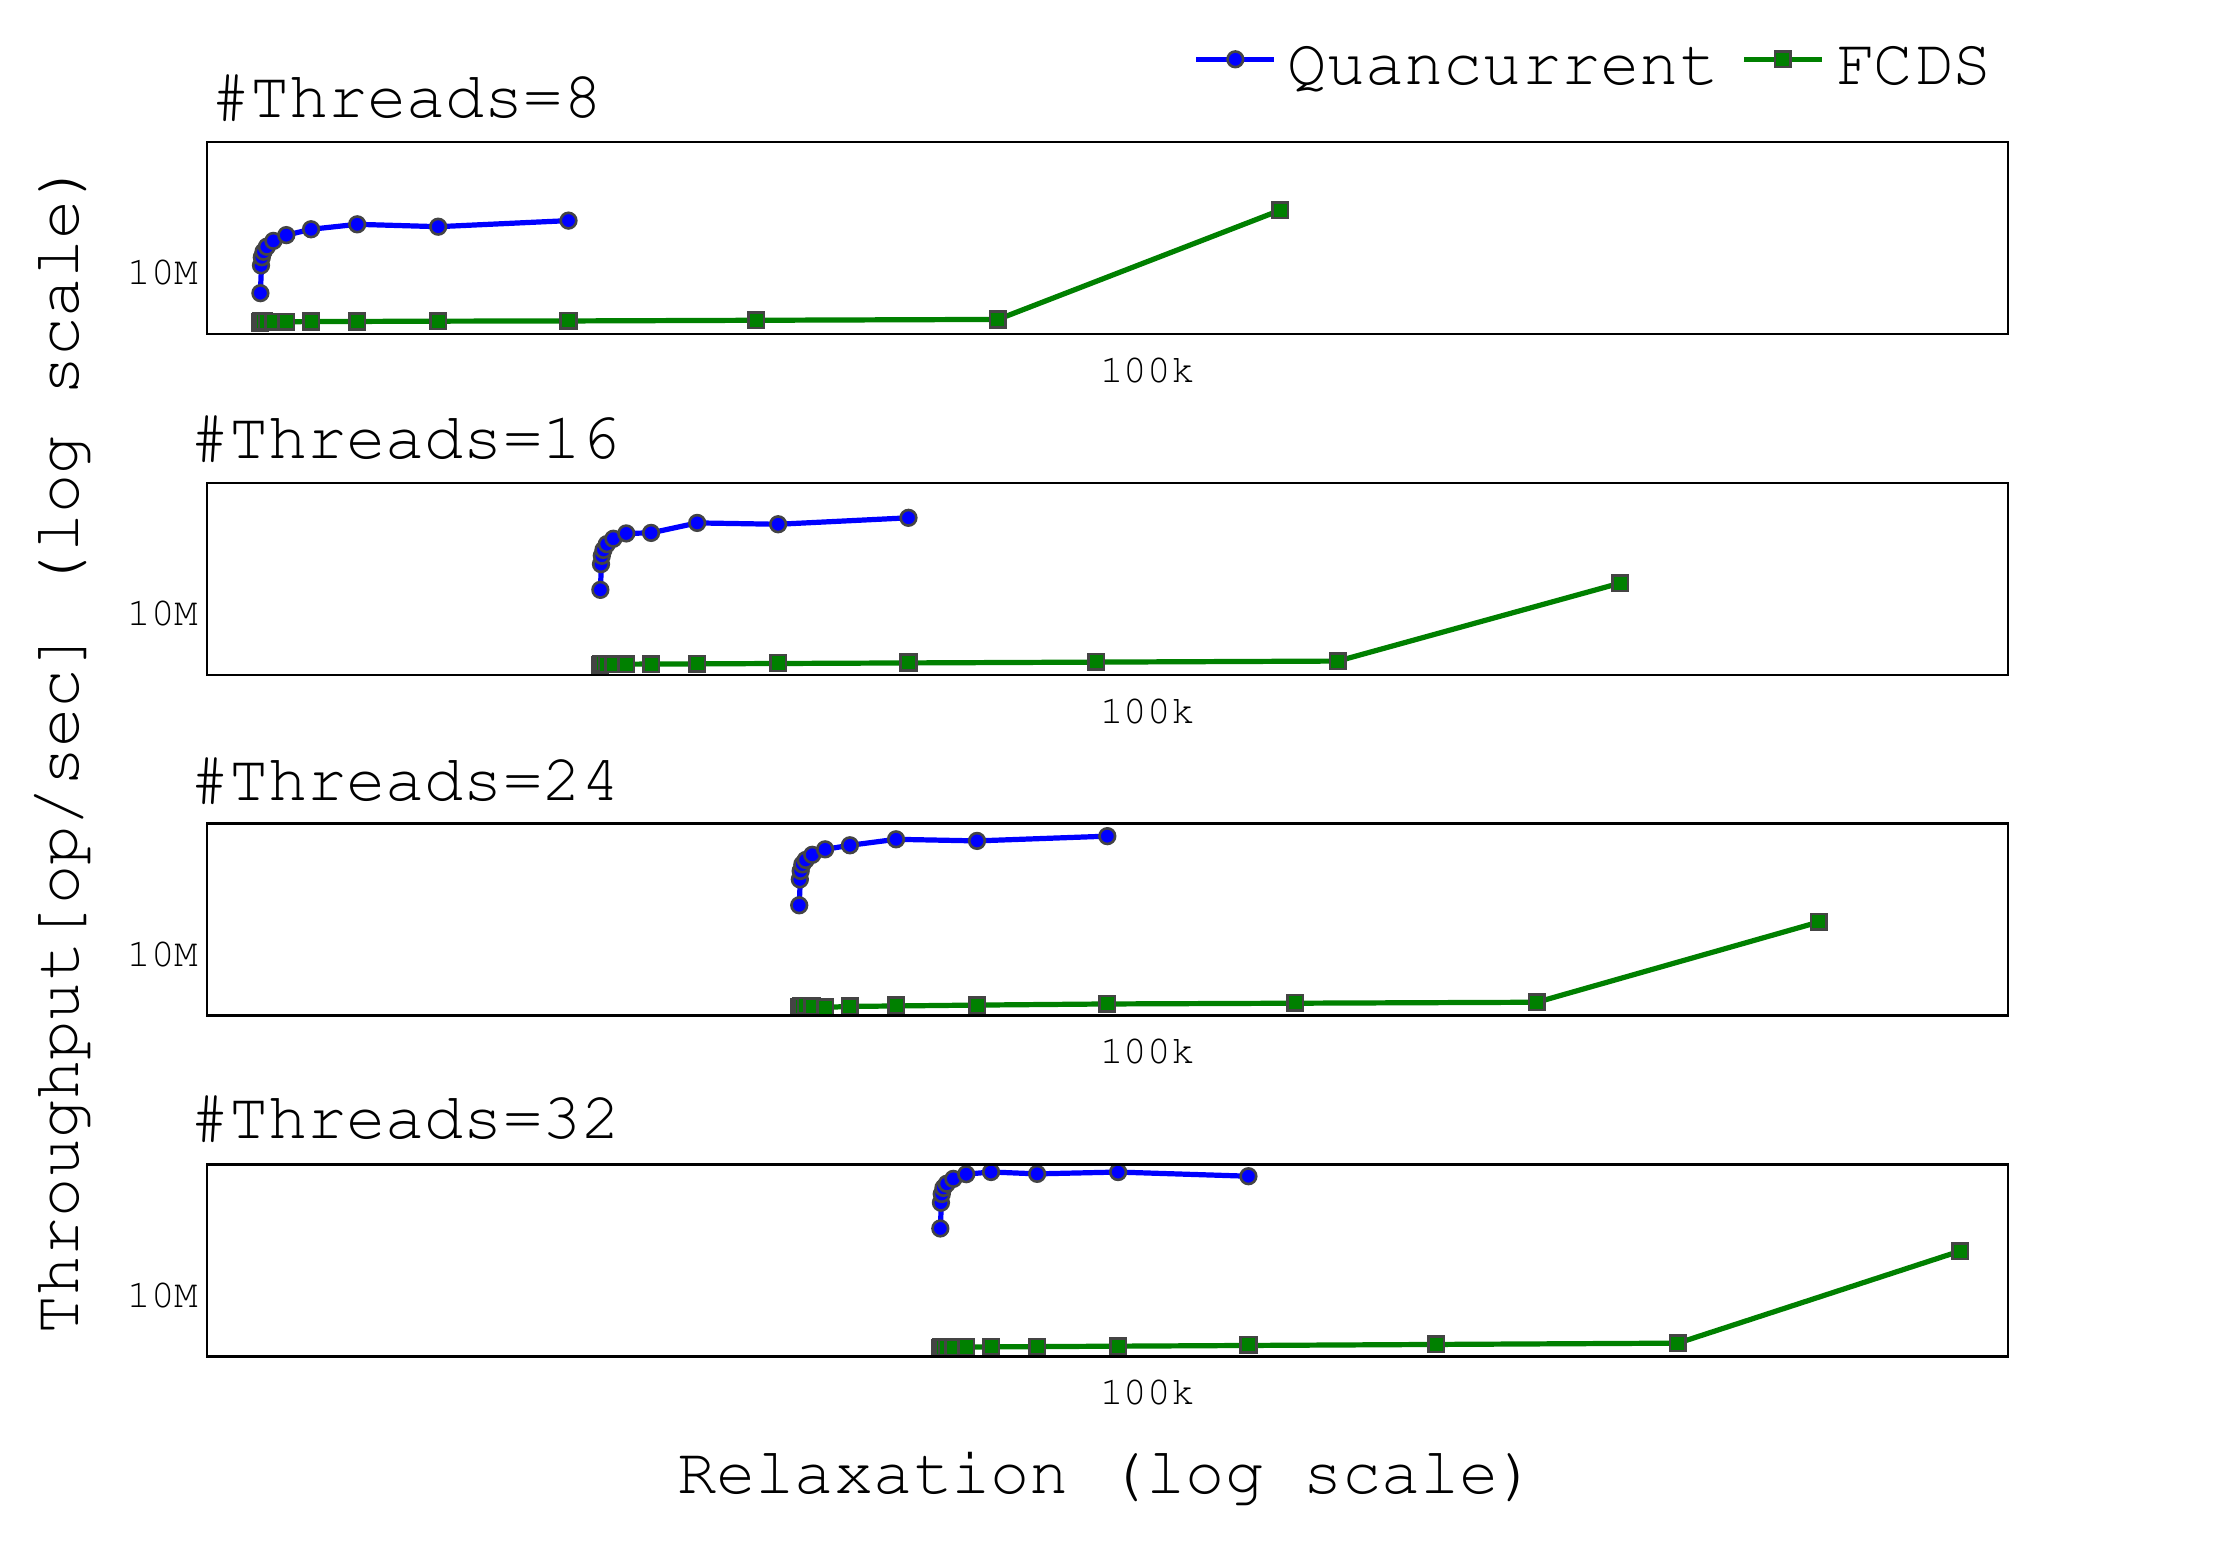}
    \caption{\mysketch vs. FCDS, k = 4096.}
    \label{fig: FCDS k4096 (full)}
\end{figure}
\FloatBarrier

\begin{table}[t]
\captionsetup{skip=0pt}
\caption{\mysketch vs. FCDS, k = 4096, \#keys = 10M}
\label{table: FCDS 4096 (full)}
\centering
\footnotesize
% \resizebox{\textwidth}{} {
% \begin{tabular} {c{20pt}|l{30pt}|l{50pt}|c{25pt}c{25pt}|r{30pt}|r{50pt}}
% \resizebox{\textwidth}{!}{%
\begin{tabular} {@{}c|lc|cc|lc@{}} \toprule
%  & \multicolumn{6}{c}{k = 256} \\
% \cmidrule(r){2-7}
 \multicolumn{1}{c}{}  & \multicolumn{3}{c|}{Quancurrent}  & \multicolumn{3}{c}{FCDS} \\  
        \cmidrule(r){1-7}
        % &       &                       &    \phantom{xxx}  &    \phantom{xxx}       &           &          \\[-\normalbaselineskip] % fake/empty row
N      &    b    &   Throughput$[\frac{\textit{op}}{\textit{sec}}]$  &   \multicolumn{2}{c|}{r}  &   B       &   Throughput$[\frac{\textit{op}}{\textit{sec}}]$ \\ \midrule
        &       &                       &    \phantom{xxx}  &    \phantom{xxx}       &           &          \\[-\normalbaselineskip] % fake/empty row
8        &   1       &   \prefix{7.10E+06}    &   \multicolumn{2}{c|}{\prefix{1.64E+04}}    &   1024    &   \prefix{4.5E+6}\\
        &   4       &   \prefix{1.09E+07}    &   \multicolumn{2}{c|}{\prefix{1.64E+04}}    &   1026    &   \prefix{4.6E+6}\\
        &   8       &   \prefix{1.24E+07}    &   \multicolumn{2}{c|}{\prefix{1.64E+04}}    &   1028    &   \prefix{4.6E+6}\\
        &   16      &   \prefix{1.35E+07}    &   \multicolumn{2}{c|}{\prefix{1.65E+04}}    &   1031    &   \prefix{4.6E+6}\\
        &   32      &   \prefix{1.46E+07}    &   \multicolumn{2}{c|}{\prefix{1.66E+04}}    &   1038    &   \prefix{4.5E+6}\\
        &   64      &   \prefix{1.60E+07}    &   \multicolumn{2}{c|}{\prefix{1.68E+04}}    &   1052    &   \prefix{4.5E+6}\\
        &   128     &   \prefix{1.75E+07}    &   \multicolumn{2}{c|}{\prefix{1.73E+04}}    &   1080    &   \prefix{4.5E+6}\\
        &   256     &   \prefix{1.92E+07}    &   \multicolumn{2}{c|}{\prefix{1.82E+04}}    &   1136    &   \prefix{4.6E+6}\\
        &   512     &   \prefix{2.07E+07}    &   \multicolumn{2}{c|}{\prefix{2.00E+04}}    &   1248    &   \prefix{4.6E+6}\\
        &   1024    &   \prefix{2.00E+07}    &   \multicolumn{2}{c|}{\prefix{2.36E+04}}    &   1472    &   \prefix{4.6E+6}\\
        &   2048    &   \prefix{2.20E+07}    &   \multicolumn{2}{c|}{\prefix{3.07E+04}}    &   1920    &   \prefix{4.6E+6}\\
        &   4096    &   \prefix{1.30E+07}    &   \multicolumn{2}{c|}{\prefix{4.51E+04}}    &   2816    &   \prefix{4.7E+6}\\
        &   8192    &   \prefix{7.13E+06}    &   \multicolumn{2}{c|}{\prefix{7.37E+04}}    &   4608    &   \prefix{4.7E+6}\\
        &           &                        &   \multicolumn{2}{c|}{\prefix{1.31E+05}}    &   8192    &   \prefix{25.8E+6}\\
        &           &                        &   \multicolumn{2}{c|}{\prefix{2.46E+05}}    &   15360   &   \prefix{9.7E+6}\\
16        &   1       &   \prefix{1.41E+07}    &   \multicolumn{2}{c|}{\prefix{3.28E+04}}    &   1024    &   \prefix{4.4E+6}\\
        &   4       &   \prefix{2.11E+07}    &   \multicolumn{2}{c|}{\prefix{3.28E+04}}    &   1026    &   \prefix{4.4E+6}\\
        &   8       &   \prefix{2.40E+07}    &   \multicolumn{2}{c|}{\prefix{3.29E+04}}    &   1028    &   \prefix{4.4E+6}\\
        &   16      &   \prefix{2.63E+07}    &   \multicolumn{2}{c|}{\prefix{3.30E+04}}    &   1031    &   \prefix{4.5E+6}\\
        &   32      &   \prefix{2.88E+07}    &   \multicolumn{2}{c|}{\prefix{3.32E+04}}    &   1038    &   \prefix{4.4E+6}\\
        &   64      &   \prefix{3.13E+07}    &   \multicolumn{2}{c|}{\prefix{3.37E+04}}    &   1052    &   \prefix{4.4E+6}\\
        &   128     &   \prefix{3.40E+07}    &   \multicolumn{2}{c|}{\prefix{3.46E+04}}    &   1080    &   \prefix{4.4E+6}\\
        &   256     &   \prefix{3.43E+07}    &   \multicolumn{2}{c|}{\prefix{3.64E+04}}    &   1136    &   \prefix{4.4E+6}\\
        &   512     &   \prefix{4.00E+07}    &   \multicolumn{2}{c|}{\prefix{3.99E+04}}    &   1248    &   \prefix{4.5E+6}\\
        &   1024    &   \prefix{3.92E+07}    &   \multicolumn{2}{c|}{\prefix{4.71E+04}}    &   1472    &   \prefix{4.5E+6}\\
        &   2048    &   \prefix{4.33E+07}    &   \multicolumn{2}{c|}{\prefix{6.14E+04}}    &   1920    &   \prefix{4.6E+6}\\
        &   4096    &   \prefix{2.53E+07}    &   \multicolumn{2}{c|}{\prefix{9.01E+04}}    &   2816    &   \prefix{4.6E+6}\\
        &   8192    &   \prefix{1.40E+07}    &   \multicolumn{2}{c|}{\prefix{1.47E+05}}    &   4608    &   \prefix{4.7E+6}\\
        &           &                        &   \multicolumn{2}{c|}{\prefix{2.62E+05}}    &   8192    &   \prefix{15.7E+6}\\
        &           &                        &   \multicolumn{2}{c|}{\prefix{4.92E+05}}    &   15360   &   \prefix{9.4E+6}\\
24        &   1       &   \prefix{2.10E+07}    &   \multicolumn{2}{c|}{\prefix{4.92E+04}}    &   1024    &   \prefix{4.3E+6}\\
        &   4       &   \prefix{3.14E+07}    &   \multicolumn{2}{c|}{\prefix{4.92E+04}}    &   1026    &   \prefix{4.3E+6}\\
        &   8       &   \prefix{3.58E+07}    &   \multicolumn{2}{c|}{\prefix{4.93E+04}}    &   1028    &   \prefix{4.4E+6}\\
        &   16      &   \prefix{3.96E+07}    &   \multicolumn{2}{c|}{\prefix{4.95E+04}}    &   1031    &   \prefix{4.3E+6}\\
        &   32      &   \prefix{4.24E+07}    &   \multicolumn{2}{c|}{\prefix{4.98E+04}}    &   1038    &   \prefix{4.4E+6}\\
        &   64      &   \prefix{4.60E+07}    &   \multicolumn{2}{c|}{\prefix{5.05E+04}}    &   1052    &   \prefix{4.4E+6}\\
        &   128     &   \prefix{5.01E+07}    &   \multicolumn{2}{c|}{\prefix{5.18E+04}}    &   1080    &   \prefix{4.3E+6}\\
        &   256     &   \prefix{5.33E+07}    &   \multicolumn{2}{c|}{\prefix{5.45E+04}}    &   1136    &   \prefix{4.3E+6}\\
        &   512     &   \prefix{5.86E+07}    &   \multicolumn{2}{c|}{\prefix{5.99E+04}}    &   1248    &   \prefix{4.4E+6}\\
        &   1024    &   \prefix{5.71E+07}    &   \multicolumn{2}{c|}{\prefix{7.07E+04}}    &   1472    &   \prefix{4.4E+6}\\
        &   2048    &   \prefix{6.15E+07}    &   \multicolumn{2}{c|}{\prefix{9.22E+04}}    &   1920    &   \prefix{4.5E+6}\\
        &   4096    &   \prefix{3.69E+07}    &   \multicolumn{2}{c|}{\prefix{1.35E+05}}    &   2816    &   \prefix{4.6E+6}\\
        &   8192    &   \prefix{2.08E+07}    &   \multicolumn{2}{c|}{\prefix{2.21E+05}}    &   4608    &   \prefix{4.6E+6}\\
        &           &                        &   \multicolumn{2}{c|}{\prefix{3.93E+05}}    &   8192    &   \prefix{16.2E+6}\\
        &           &                        &   \multicolumn{2}{c|}{\prefix{7.37E+05}}    &   15360   &   \prefix{8.9E+6}\\
32        &   1       &   \prefix{2.76E+07}    &   \multicolumn{2}{c|}{\prefix{6.55E+04}}    &   1024    &   \prefix{4.3E+6}\\
        &   4       &   \prefix{4.12E+07}    &   \multicolumn{2}{c|}{\prefix{6.57E+04}}    &   1026    &   \prefix{4.3E+6}\\
        &   8       &   \prefix{4.72E+07}    &   \multicolumn{2}{c|}{\prefix{6.58E+04}}    &   1028    &   \prefix{4.3E+6}\\
        &   16      &   \prefix{5.19E+07}    &   \multicolumn{2}{c|}{\prefix{6.60E+04}}    &   1031    &   \prefix{4.3E+6}\\
        &   32      &   \prefix{5.54E+07}    &   \multicolumn{2}{c|}{\prefix{6.64E+04}}    &   1038    &   \prefix{4.3E+6}\\
        &   64      &   \prefix{5.97E+07}    &   \multicolumn{2}{c|}{\prefix{6.73E+04}}    &   1052    &   \prefix{4.4E+6}\\
        &   128     &   \prefix{6.43E+07}    &   \multicolumn{2}{c|}{\prefix{6.91E+04}}    &   1080    &   \prefix{4.4E+6}\\
        &   256     &   \prefix{6.65E+07}    &   \multicolumn{2}{c|}{\prefix{7.27E+04}}    &   1136    &   \prefix{4.4E+6}\\
        &   512     &   \prefix{6.46E+07}    &   \multicolumn{2}{c|}{\prefix{7.99E+04}}    &   1248    &   \prefix{4.4E+6}\\
        &   1024    &   \prefix{6.64E+07}    &   \multicolumn{2}{c|}{\prefix{9.42E+04}}    &   1472    &   \prefix{4.4E+6}\\
        &   2048    &   \prefix{6.23E+07}    &   \multicolumn{2}{c|}{\prefix{1.23E+05}}    &   1920    &   \prefix{4.5E+6}\\
        &   4096    &   \prefix{4.81E+07}    &   \multicolumn{2}{c|}{\prefix{1.80E+05}}    &   2816    &   \prefix{4.6E+6}\\
        &   8192    &   \prefix{2.73E+07}    &   \multicolumn{2}{c|}{\prefix{2.95E+05}}    &   4608    &   \prefix{4.6E+6}\\
        &           &                        &   \multicolumn{2}{c|}{\prefix{5.24E+05}}    &   8192    &   \prefix{19.4E+6}\\
        &           &                        &   \multicolumn{2}{c|}{\prefix{9.83E+05}}    &   15360   &   \prefix{9.4E+6}\\
\bottomrule
\end{tabular} 
% }
% \caption{\mysketch vs. FCDS, k = 4096, \#keys = 10M}
% \label{table: FCDS 4096 (full)}
\end{table}

\FloatBarrier

\newpage
\subsubsection{k = 256}

\FloatBarrier
\begin{figure}[b]
    \centering
    \includegraphics[width=\columnwidth,trim={0.1cm 0.2cm 1.9cm 0.1cm},clip]
    {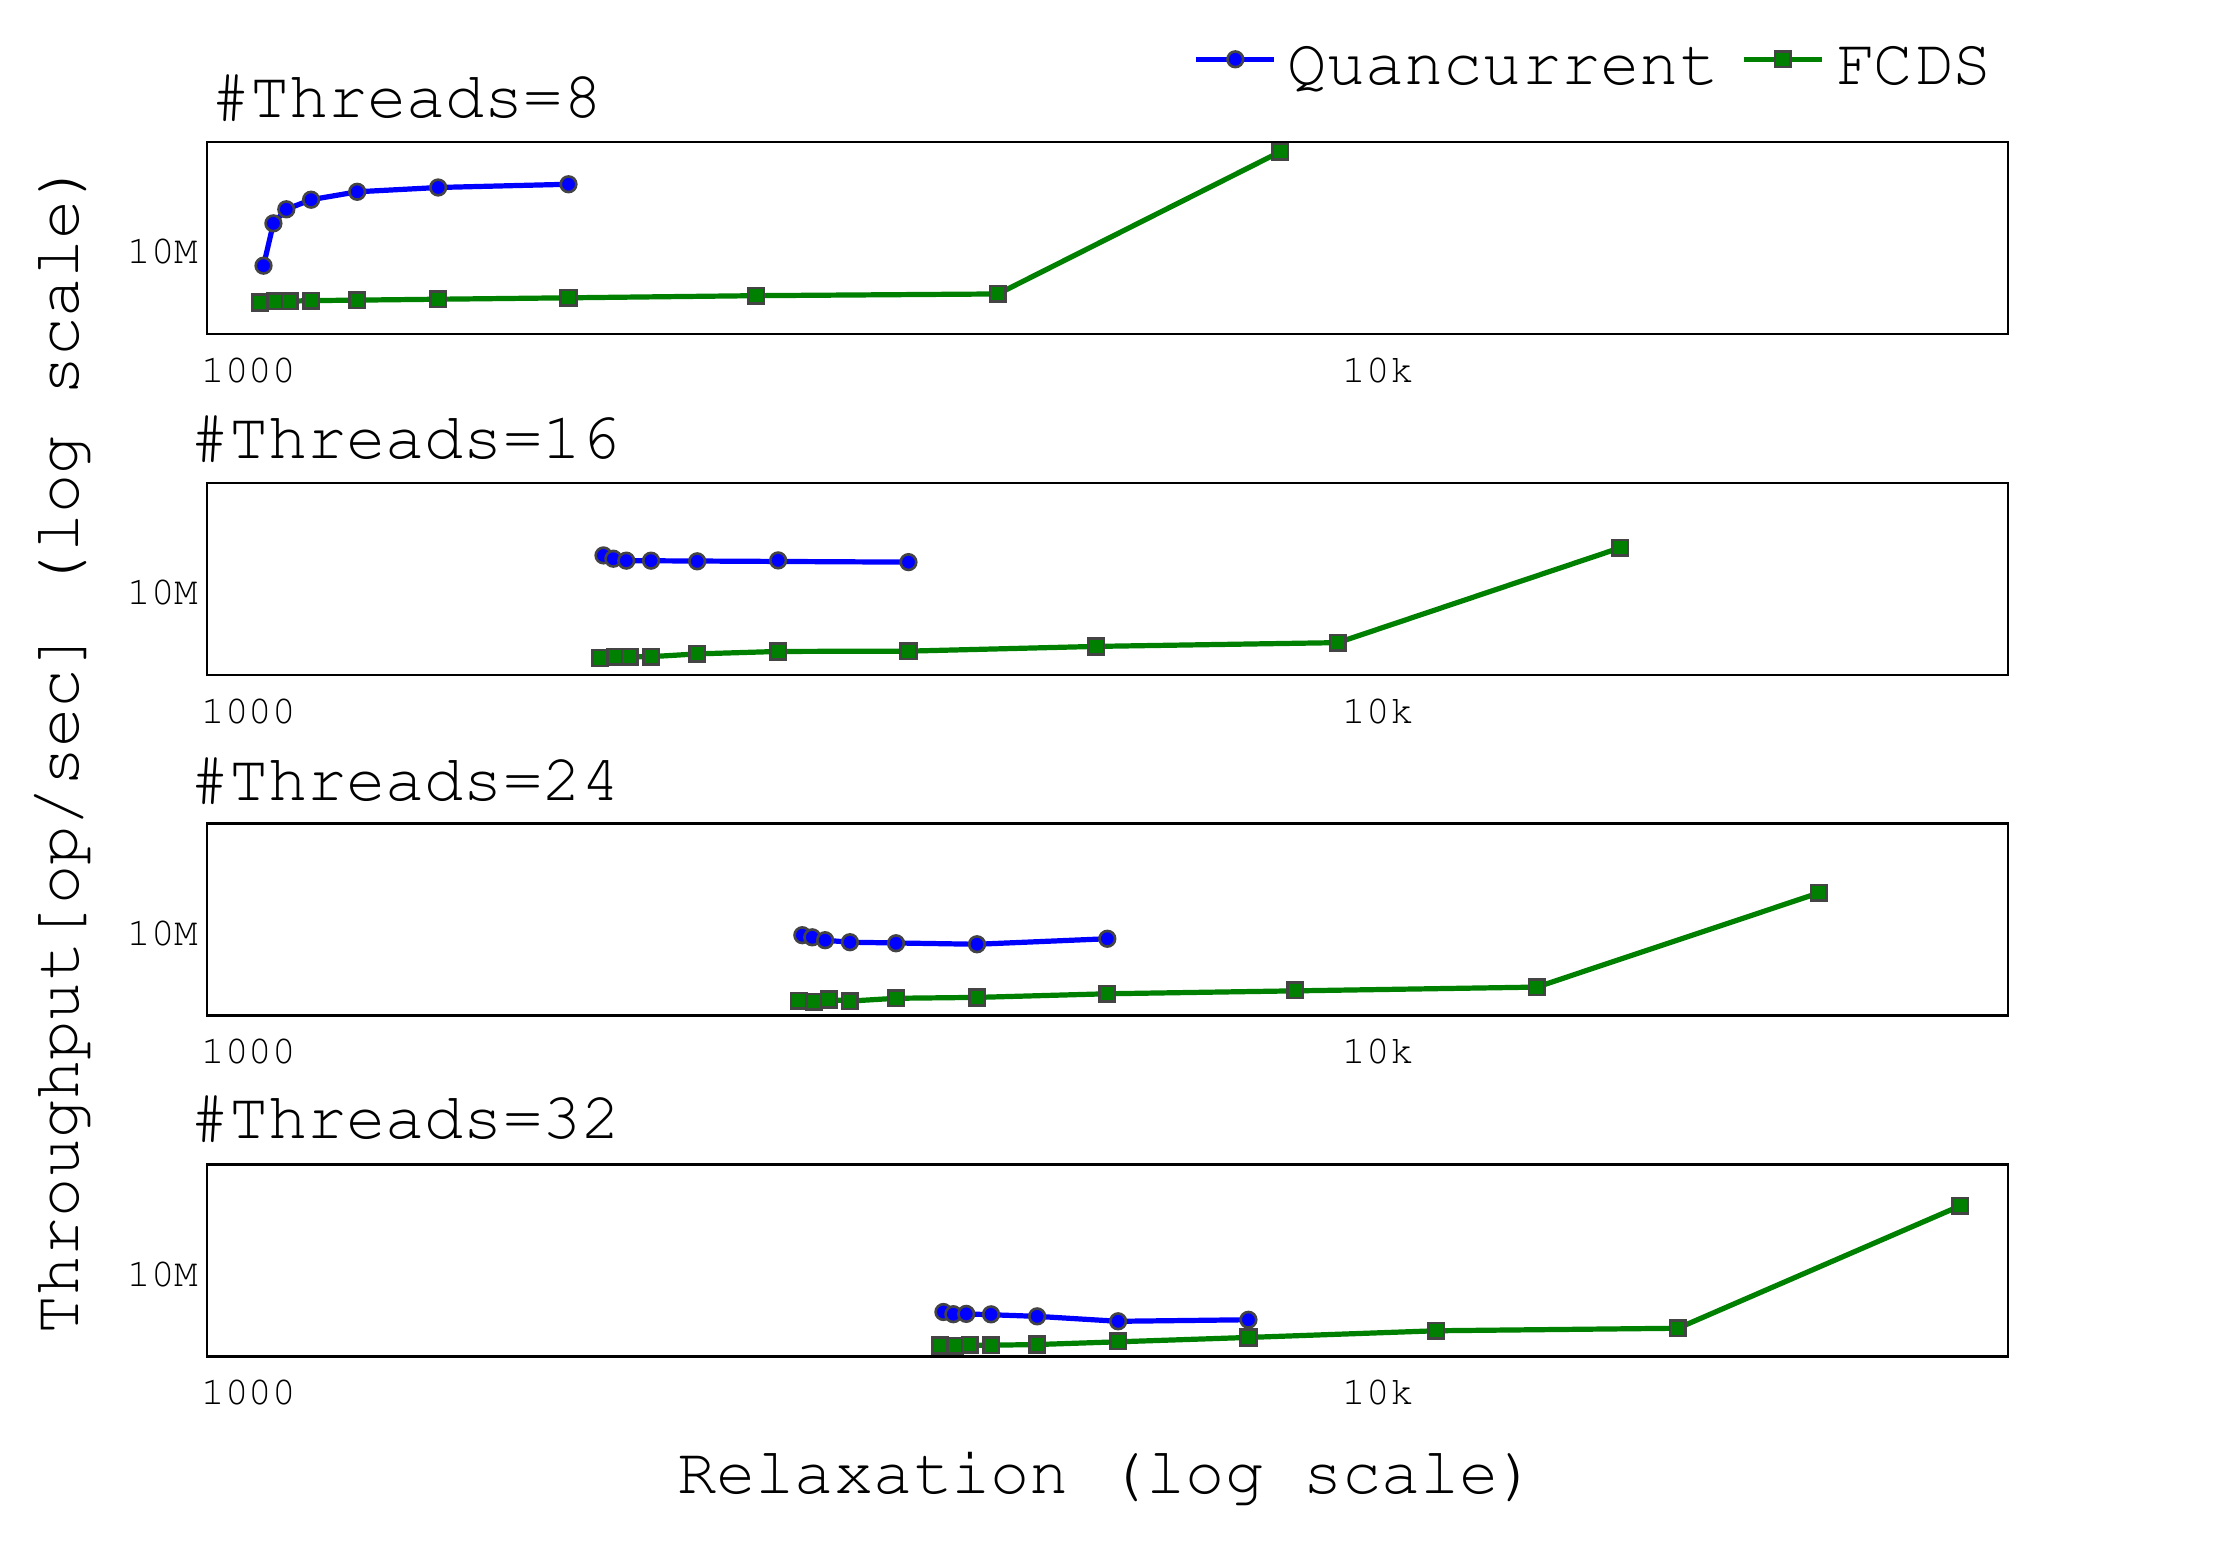}
    \caption{\mysketch vs. FCDS, k = 256, \#keys = 10M.}
    \label{fig: FCDS k256 (full)}
\end{figure}
\FloatBarrier

\begin{table}[t]
\captionsetup{skip=0pt}
\caption{\mysketch vs. FCDS, k = 256, \#keys = 10M}
\label{table: FCDS 256 (full)}
\centering
\small
% \resizebox{\textwidth}{} {
% \begin{tabular} {c{20pt}|l{30pt}|l{50pt}|c{25pt}c{25pt}|r{30pt}|r{50pt}}
% \resizebox{\columnwidth}{!}{%
\begin{tabular} {@{}c|lc|cc|lc@{}} \toprule
%  & \multicolumn{6}{c}{k = 256} \\
% \cmidrule(r){2-7}
 \multicolumn{1}{c}{}  & \multicolumn{3}{c|}{Quancurrent}  & \multicolumn{3}{c}{FCDS} \\  
        \cmidrule(r){1-7}
        % &       &                       &    \phantom{xxx}  &    \phantom{xxx}       &           &          \\[-\normalbaselineskip] % fake/empty row
N      &    b    &   Throughput$[\frac{\textit{op}}{\textit{sec}}]$  &   \multicolumn{2}{c|}{r}  &   B       &   Throughput$[\frac{\textit{op}}{\textit{sec}}]$ \\ \midrule
        &       &                       &    \phantom{xxx}  &    \phantom{xxx}       &           &          \\[-\normalbaselineskip] % fake/empty row
8      &   1    &  \prefix{8.41E+06}    &   \multicolumn{2}{c|}{\prefix{1.02E+03}}   &    64     &    \prefix{5.60E+06}\\
       &   4    &  \prefix{1.35E+07}    &   \multicolumn{2}{c|}{\prefix{1.06E+03}}   &    66     &    \prefix{5.60E+06}\\
       &   8    &  \prefix{1.58E+07}    &   \multicolumn{2}{c|}{\prefix{1.09E+03}}   &    68     &    \prefix{5.70E+06}\\
       &   16   &  \prefix{1.76E+07}    &   \multicolumn{2}{c|}{\prefix{1.14E+03}}   &    71     &    \prefix{5.70E+06}\\
       &   32   &  \prefix{1.93E+07}    &   \multicolumn{2}{c|}{\prefix{1.25E+03}}   &    78     &    \prefix{5.70E+06}\\
       &   64   &  \prefix{2.02E+07}    &   \multicolumn{2}{c|}{\prefix{1.47E+03}}   &    92     &    \prefix{5.80E+06}\\
       &   128  &  \prefix{2.10E+07}    &   \multicolumn{2}{c|}{\prefix{1.92E+03}}   &    120    &    \prefix{5.90E+06}\\
       &   256  &  \prefix{1.53E+07}    &   \multicolumn{2}{c|}{\prefix{2.82E+03}}   &    176    &    \prefix{6.00E+06}\\
       &   512  &  \prefix{8.13E+06}    &   \multicolumn{2}{c|}{\prefix{4.61E+03}}   &    288    &    \prefix{6.10E+06}\\
       &        &                       &   \multicolumn{2}{c|}{\prefix{8.19E+03}}   &    512    &    \prefix{3.01E+07}\\
       &        &                       &   \multicolumn{2}{c|}{\prefix{1.54E+04}}   &    960    &    \prefix{1.25E+07}\\
       &        &                       &   \multicolumn{2}{c|}{\prefix{2.97E+04}}   &    1856   &    \prefix{2.95E+07}\\
16     &   1    &  \prefix{1.49E+07}    &   \multicolumn{2}{c|}{\prefix{2.05E+03}}   &    64     &    \prefix{4.70E+06}\\
       &   4    &  \prefix{1.44E+07}    &   \multicolumn{2}{c|}{\prefix{2.11E+03}}   &    66     &    \prefix{4.80E+06}\\
       &   8    &  \prefix{1.41E+07}    &   \multicolumn{2}{c|}{\prefix{2.18E+03}}   &    68     &    \prefix{4.80E+06}\\
       &   16   &  \prefix{1.41E+07}    &   \multicolumn{2}{c|}{\prefix{2.27E+03}}   &    71     &    \prefix{4.80E+06}\\
       &   32   &  \prefix{1.40E+07}    &   \multicolumn{2}{c|}{\prefix{2.50E+03}}   &    78     &    \prefix{4.90E+06}\\
       &   64   &  \prefix{1.41E+07}    &   \multicolumn{2}{c|}{\prefix{2.94E+03}}   &    92     &    \prefix{5.10E+06}\\
       &   128  &  \prefix{1.38E+07}    &   \multicolumn{2}{c|}{\prefix{3.84E+03}}   &    120    &    \prefix{5.10E+06}\\
       &   256  &  \prefix{1.46E+07}    &   \multicolumn{2}{c|}{\prefix{5.63E+03}}   &    176    &    \prefix{5.40E+06}\\
       &   512  &  \prefix{1.39E+07}    &   \multicolumn{2}{c|}{\prefix{9.22E+03}}   &    288    &    \prefix{5.60E+06}\\
       &        &                       &   \multicolumn{2}{c|}{\prefix{1.64E+04}}   &    512    &    \prefix{1.62E+07}\\
       &        &                       &   \multicolumn{2}{c|}{\prefix{3.07E+04}}   &    960    &    \prefix{1.15E+07}\\
       &        &                       &   \multicolumn{2}{c|}{\prefix{5.94E+04}}   &    1856   &    \prefix{1.62E+07}\\
24     &   1    &  \prefix{9.64E+06}    &   \multicolumn{2}{c|}{\prefix{3.07E+03}}   &    64     &    \prefix{4.60E+06}\\
       &   4    &  \prefix{9.42E+06}    &   \multicolumn{2}{c|}{\prefix{3.17E+03}}   &    66     &    \prefix{4.60E+06}\\
       &   16   &  \prefix{8.91E+06}    &   \multicolumn{2}{c|}{\prefix{3.26E+03}}   &    71     &    \prefix{4.60E+06}\\
       &   8    &  \prefix{9.11E+06}    &   \multicolumn{2}{c|}{\prefix{3.41E+03}}   &    68     &    \prefix{4.70E+06}\\
       &   32   &  \prefix{8.81E+06}    &   \multicolumn{2}{c|}{\prefix{3.74E+03}}   &    78     &    \prefix{4.80E+06}\\
       &   64   &  \prefix{8.71E+06}    &   \multicolumn{2}{c|}{\prefix{4.42E+03}}   &    92     &    \prefix{4.80E+06}\\
       &   128  &  \prefix{9.26E+06}    &   \multicolumn{2}{c|}{\prefix{5.76E+03}}   &    120    &    \prefix{5.00E+06}\\
       &   256  &  \prefix{8.79E+06}    &   \multicolumn{2}{c|}{\prefix{8.45E+03}}   &    176    &    \prefix{5.20E+06}\\
       &   512  &  \prefix{1.04E+07}    &   \multicolumn{2}{c|}{\prefix{1.38E+04}}   &    288    &    \prefix{5.40E+06}\\
       &        &                       &   \multicolumn{2}{c|}{\prefix{2.46E+04}}   &    512    &    \prefix{1.55E+07}\\
       &        &                       &   \multicolumn{2}{c|}{\prefix{4.61E+04}}   &    960    &    \prefix{1.07E+07}\\
       &        &                       &   \multicolumn{2}{c|}{\prefix{8.91E+04}}   &    1856   &    \prefix{1.84E+07}\\
32     &   1    &  \prefix{6.44E+06}    &   \multicolumn{2}{c|}{\prefix{4.10E+03}}   &    64     &    \prefix{4.40E+06}\\
       &   4    &  \prefix{6.28E+06}    &   \multicolumn{2}{c|}{\prefix{4.22E+03}}   &    66     &    \prefix{4.40E+06}\\
       &   8    &  \prefix{6.31E+06}    &   \multicolumn{2}{c|}{\prefix{4.35E+03}}   &    68     &    \prefix{4.50E+06}\\
       &   16   &  \prefix{6.27E+06}    &   \multicolumn{2}{c|}{\prefix{4.54E+03}}   &    71     &    \prefix{4.40E+06}\\
       &   32   &  \prefix{6.13E+06}    &   \multicolumn{2}{c|}{\prefix{4.99E+03}}   &    78     &    \prefix{4.50E+06}\\
       &   64   &  \prefix{5.80E+06}    &   \multicolumn{2}{c|}{\prefix{5.89E+03}}   &    92     &    \prefix{4.60E+06}\\
       &   128  &  \prefix{5.90E+06}    &   \multicolumn{2}{c|}{\prefix{7.68E+03}}   &    120    &    \prefix{4.80E+06}\\
       &   256  &  \prefix{6.38E+06}    &   \multicolumn{2}{c|}{\prefix{1.13E+04}}   &    176    &    \prefix{5.20E+06}\\
       &   512  &  \prefix{6.12E+06}    &   \multicolumn{2}{c|}{\prefix{1.84E+04}}   &    288    &    \prefix{5.40E+06}\\
       &        &                       &   \multicolumn{2}{c|}{\prefix{3.28E+04}}   &    512    &    \prefix{2.12E+07}\\
       &        &                       &   \multicolumn{2}{c|}{\prefix{6.14E+04}}   &    960    &    \prefix{1.11E+07}\\
       &        &                       &   \multicolumn{2}{c|}{\prefix{1.19E+05}}   &    1856   &    \prefix{1.93E+07}\\ 
\bottomrule
\end{tabular} 
% }
% \caption{\mysketch vs. FCDS, k = 256, \#keys = 10M}
% \label{table: FCDS 256 (full)}
\end{table}
\FloatBarrier
