# Supplementary material for: Quancurrent: A Concurrent Quantiles Sketch
Source: arXiv:2208.09265 source file (2022-08-19)
Supplement: Supplementary file 4 [file Throughput.tex]

\subsubsection{Query only}
\FloatBarrier
\begin{figure*}[]
 \centering
    \begin{subfigure}[t]{0.49\textwidth}
    \includegraphics[width=\textwidth,trim={0 0.3cm 1.9cm 2.5cm},clip]{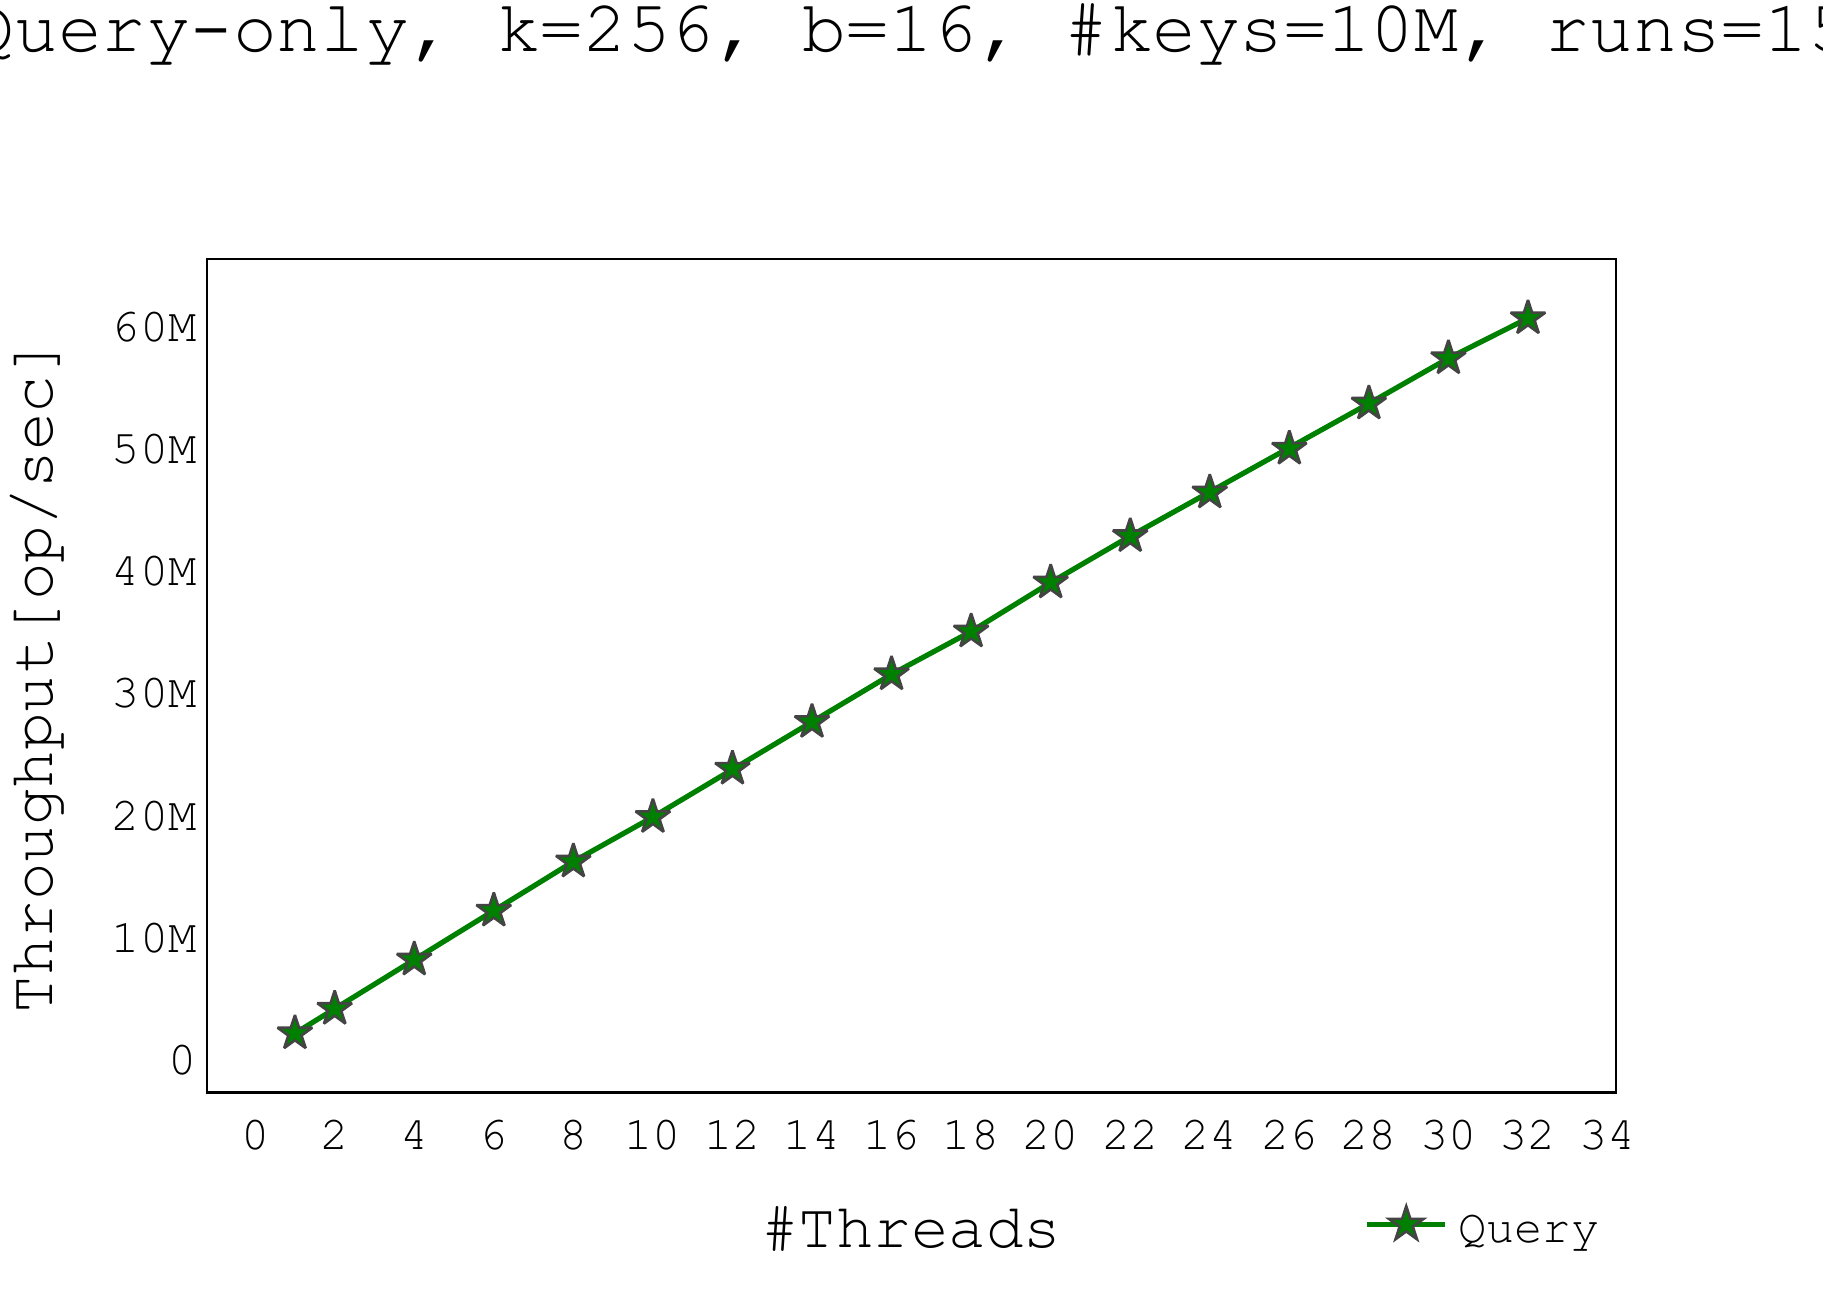}
    \caption{Query-only, k = 256, 10M elements.}
    \label{fig: query_only_k256_appendix}
    \end{subfigure}
    \hfill
    \begin{subfigure}[t]{0.49\textwidth}
    \includegraphics[width=\textwidth,trim={0 0.3cm 1.9cm 2.5cm},clip]{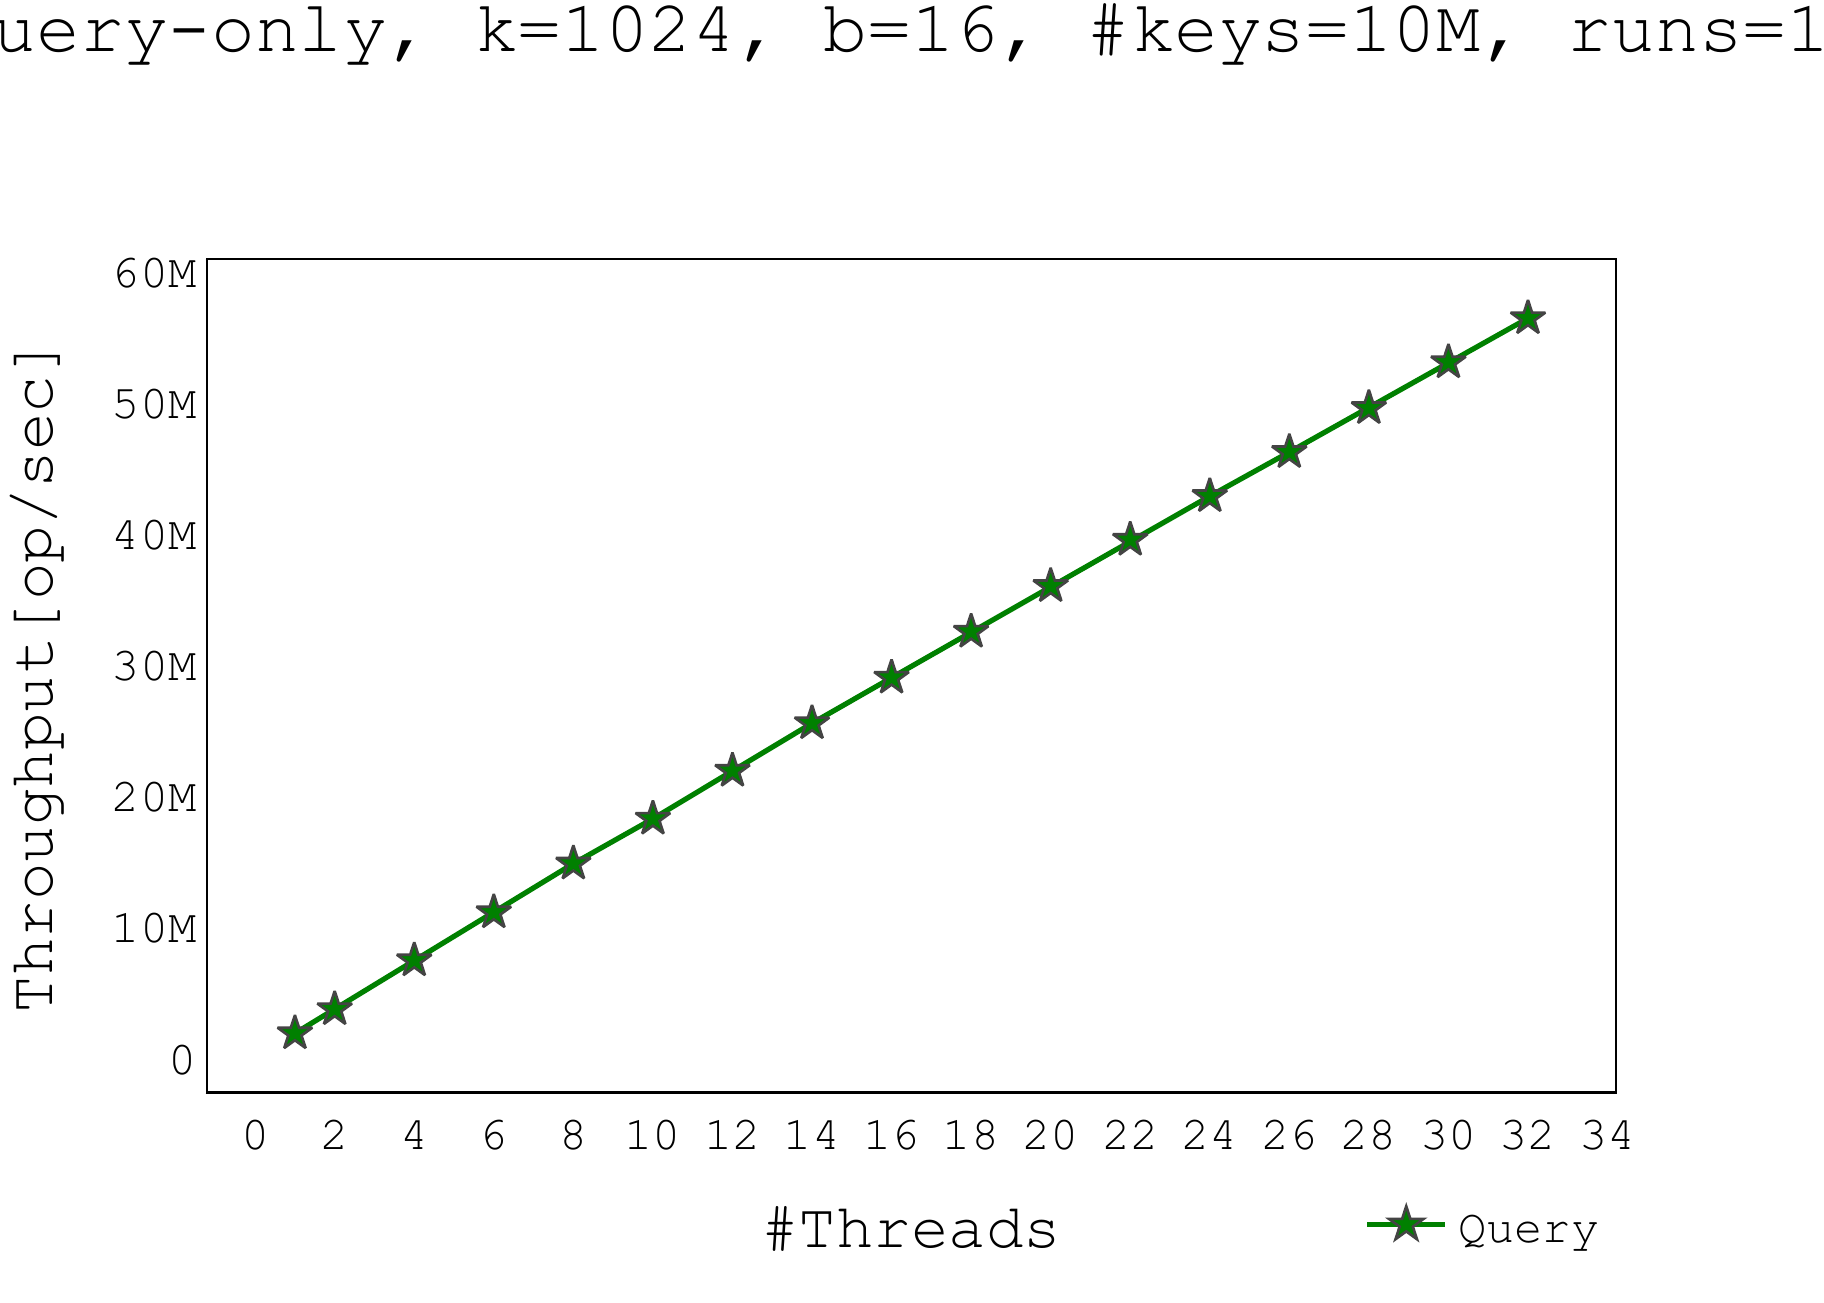}
    \caption{Query-only, k = 1024, 10M elements.}
    \label{fig: query_only_k1024_appendix}
    \end{subfigure}
    \vfill
    \begin{subfigure}[t]{0.49\textwidth}
    \includegraphics[width=\textwidth,trim={0 0.3cm 1.9cm 2.5cm},clip]{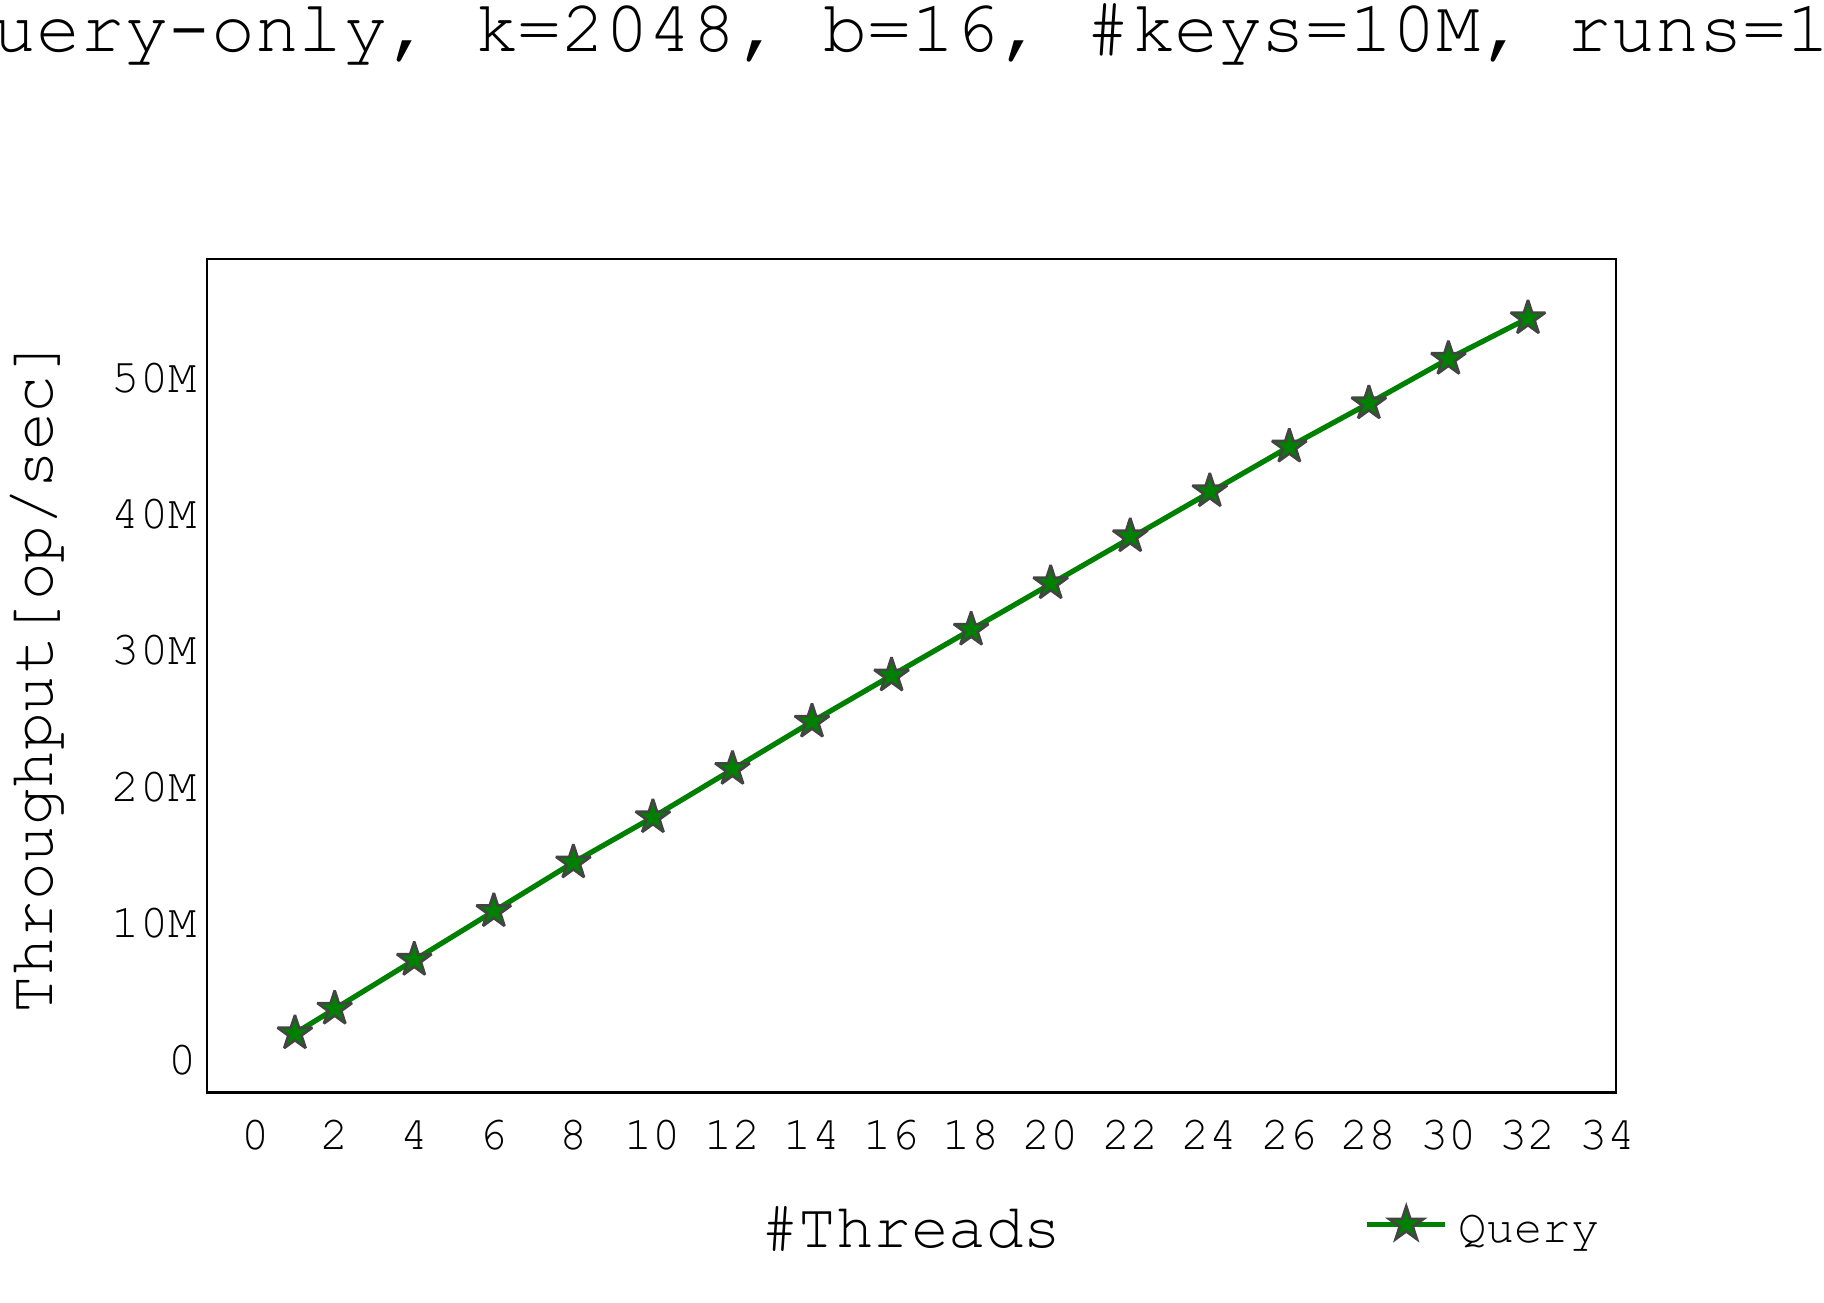}
    \caption{Query-only, k = 2048, 10M elements.}
    \label{fig: query_only_k2048_appendix}
    \end{subfigure}
    \hfill
    \begin{subfigure}[t]{0.49\textwidth}
    \includegraphics[width=\textwidth,trim={0 0.3cm 1.9cm 2.5cm},clip]{images/graphs/throughput/oracle_Quancurrent_blocking_numa_query_only_k4096_b16_keys10M_Tup32_runs15_06-07-2022_08-25-03.pdf}
    \caption{Query-only, k = 4096, 10M elements.}
    \label{fig: query_only_k4096_appendix}
    \end{subfigure}
    \caption{\mysketch Query-only throughput.}
    \label{fig: query_only_throughput_appendix}
\end{figure*}
\FloatBarrier

\newpage
\subsubsection{1-2 update threads in the presence of multiple queries threads}

 $\epsilon$' is $c_1$, where $c_1$ is a constant.
 I executed this test with the following constants and choose the best results for each $k$: 
 \[ c_2 \in [0, 0.0025, 0.005, 0.01, 0.02, 0.05, 0.1, 0.2, 0.5]\]
\begin{figure*}[]
 \centering
\includegraphics[width=\textwidth,trim={0 0cm 0cm 2cm},clip]{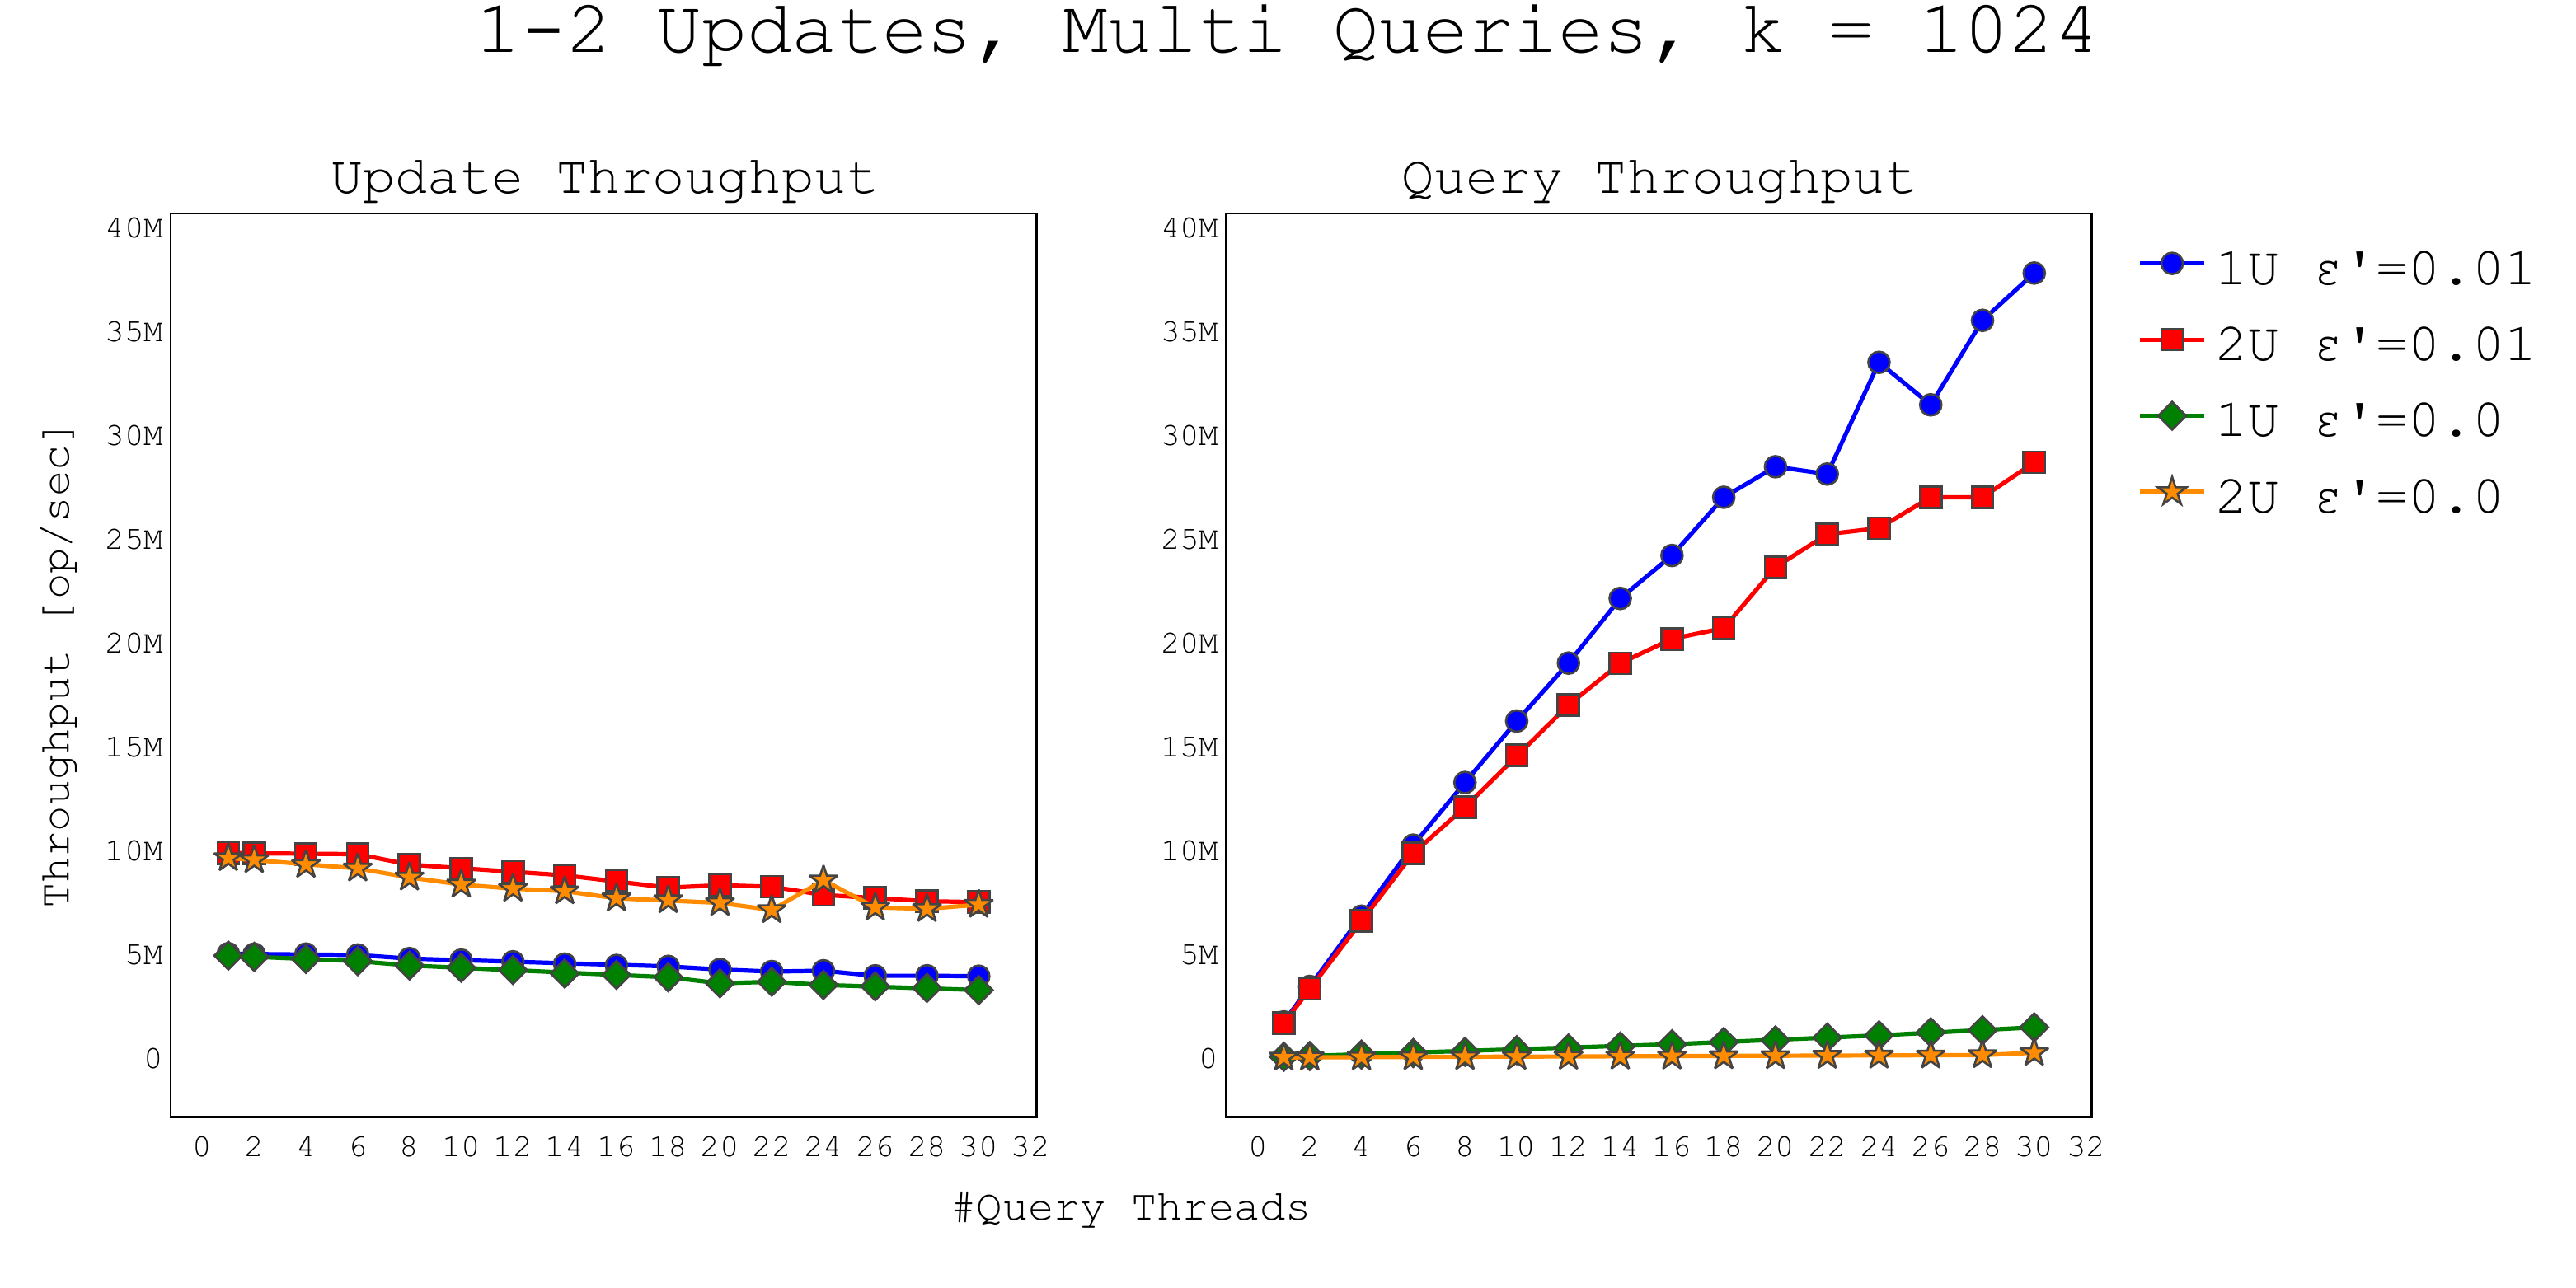}
\caption{\mysketch 1-2 updates, multiple queries, k = 1024, 10M elements.}
\label{fig: 1_2update_multi_query_k1024_1M_appendix}
\end{figure*}

\begin{figure*}[]
 \centering
\includegraphics[width=\textwidth,trim={0 0cm 0cm 2cm},clip]{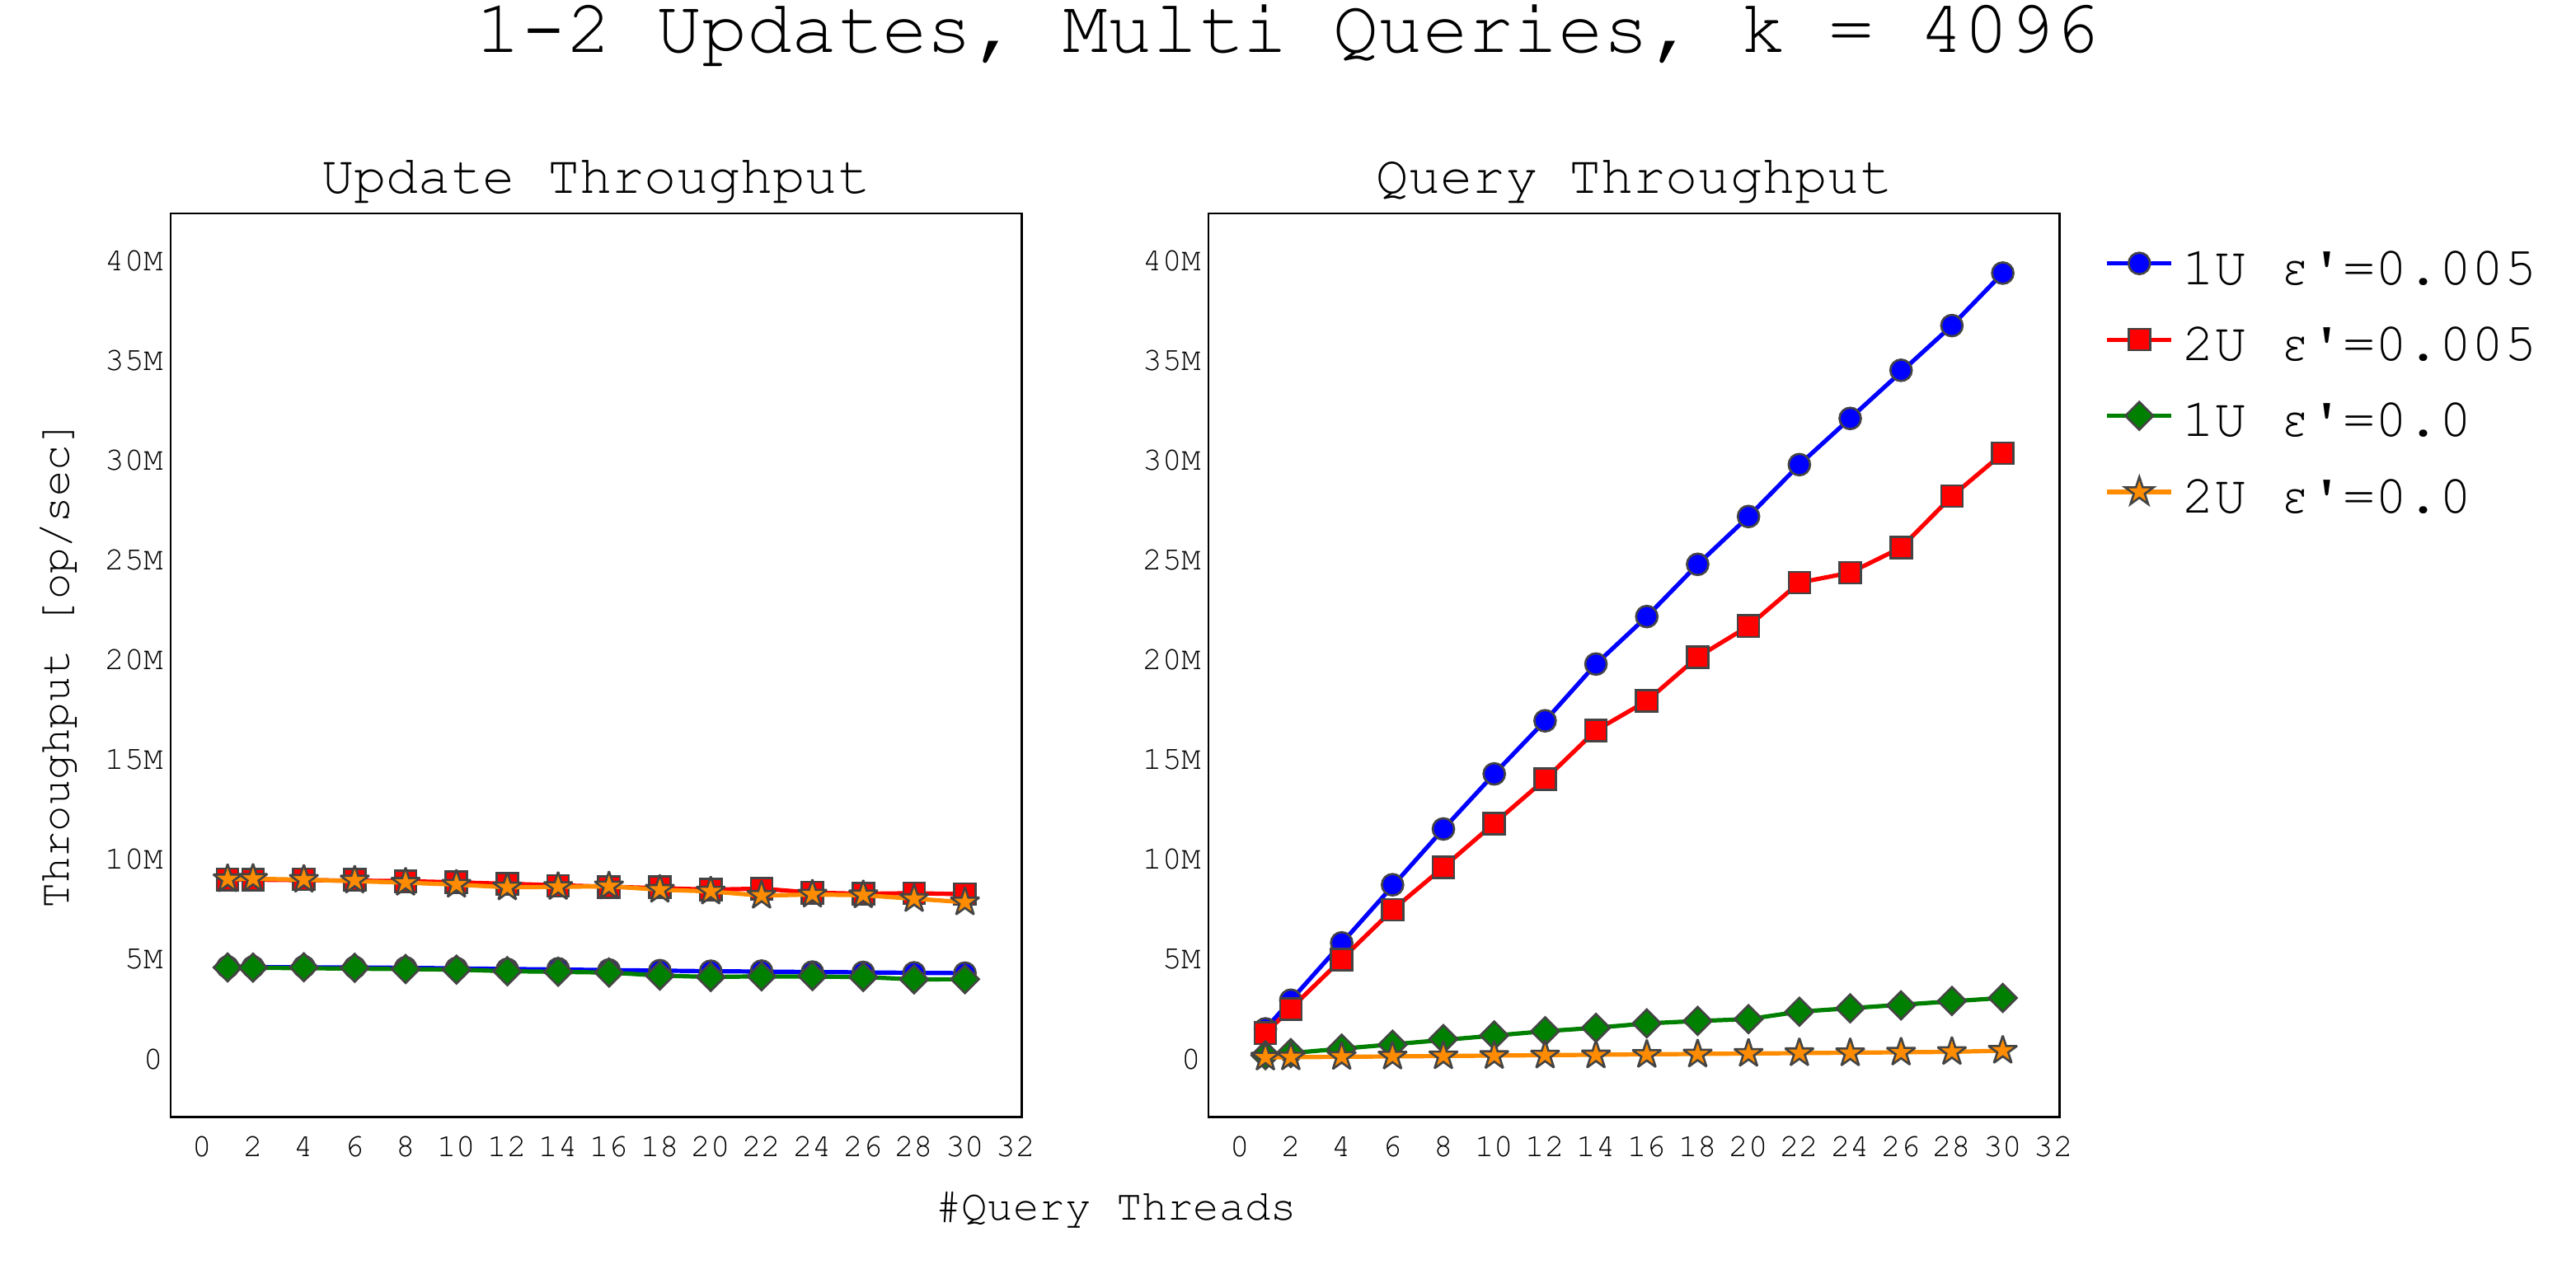}
\caption{\mysketch 1-2 updates, multiple queries, k = 4096, 10M elements.}
\label{fig: 1_2update_multi_query_k4096_1M_appendix}
\end{figure*}
\FloatBarrier

\newpage
 $\epsilon$' is $c_2\cdot \epsilon_{seq}$, where $c_2$ is a constant and $\epsilon_{seq}$ is calculated based on $k$

\FloatBarrier
\begin{figure*}[]
 \centering
    \begin{subfigure}[t]{0.49\textwidth}
    \includegraphics[width=\textwidth,trim={0 0.3cm 1.9cm 2.5cm},clip]{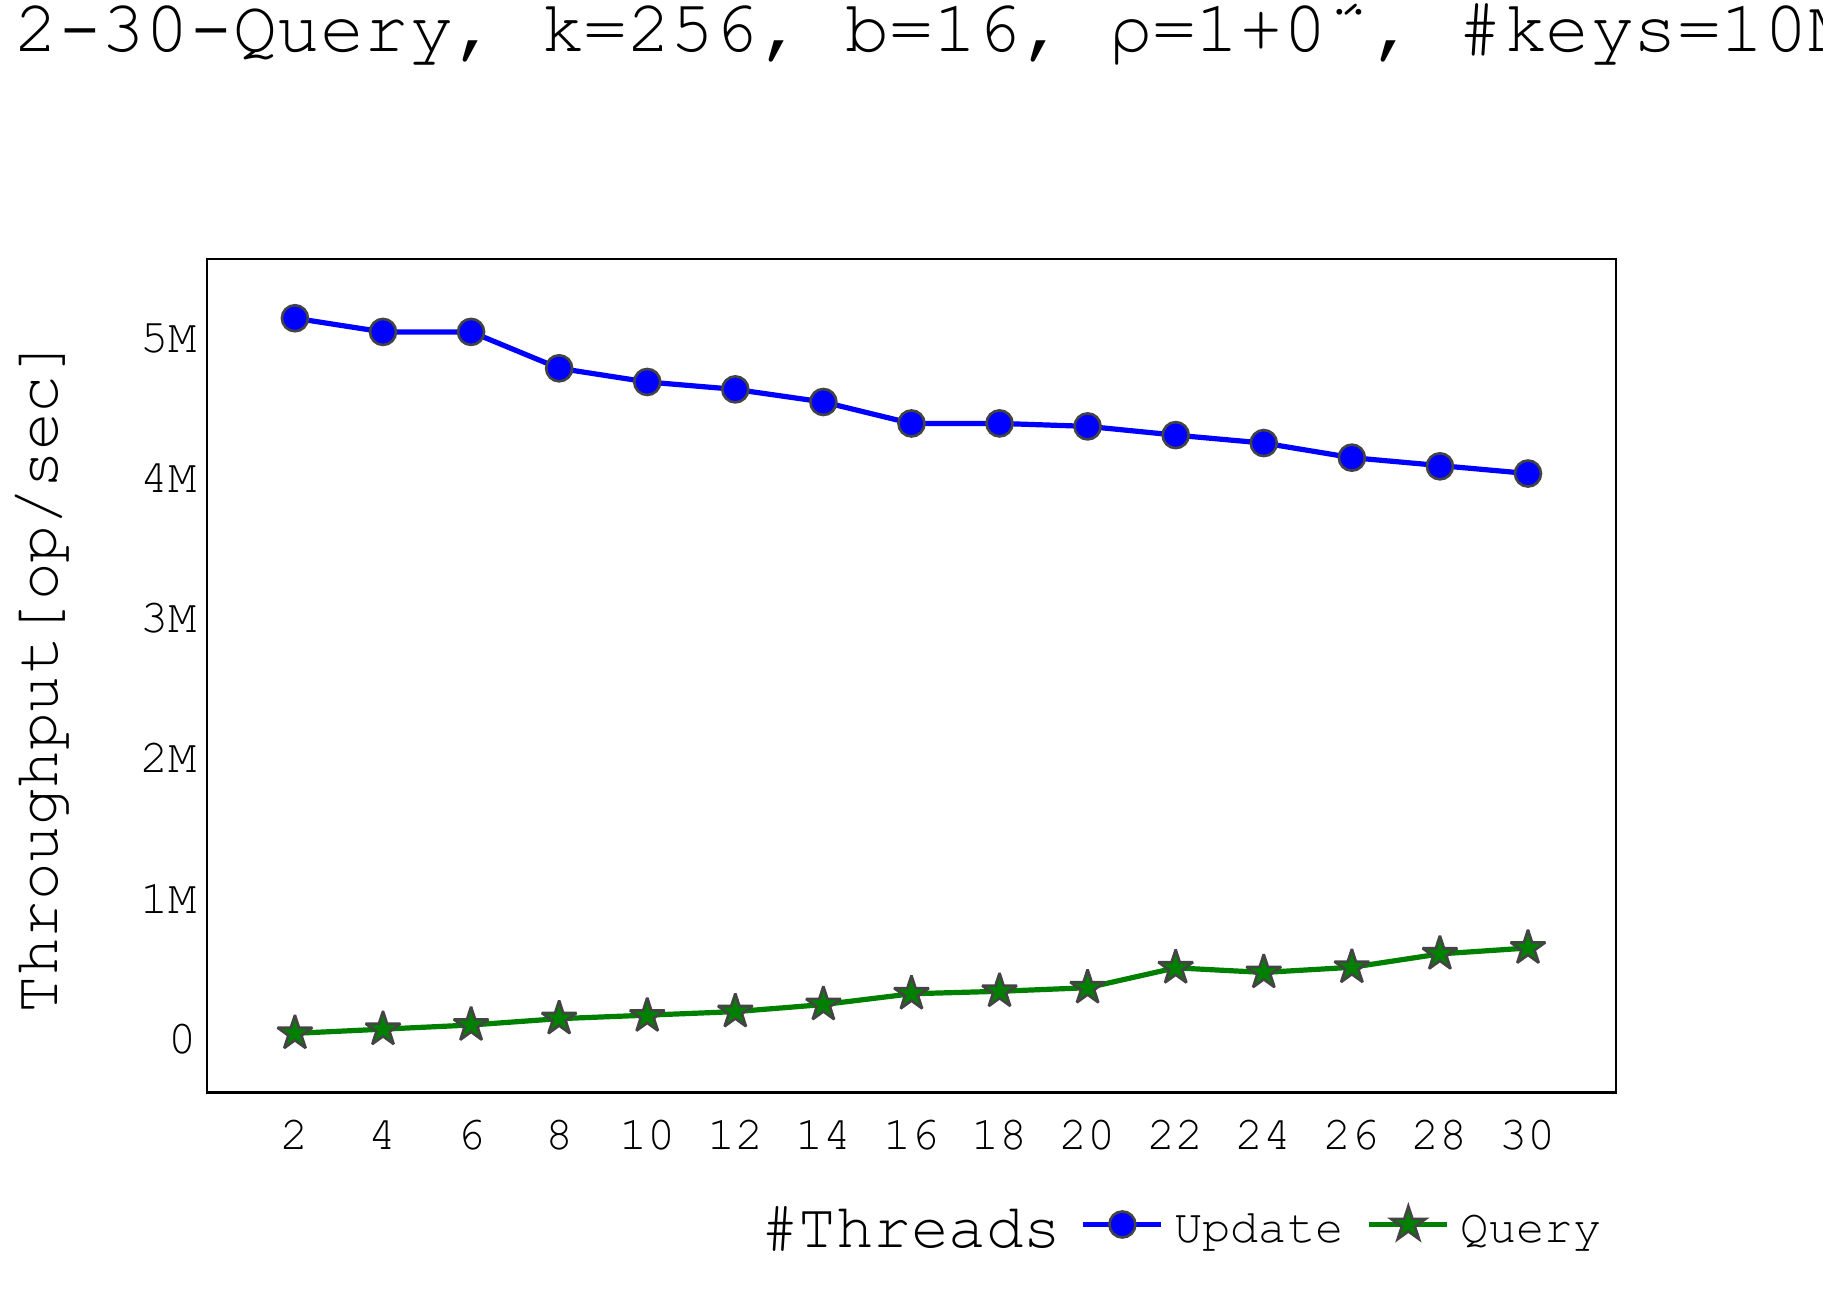}
    \caption{1 update, $\rho=1$, 10M elements.}
    \label{fig: 1update_multi_query_k256_rho_1_0_appendix}
    \end{subfigure}
    \hfill
    \begin{subfigure}[t]{0.49\textwidth}
    \includegraphics[width=\textwidth,trim={0 0.3cm 1.9cm 2.5cm},clip]{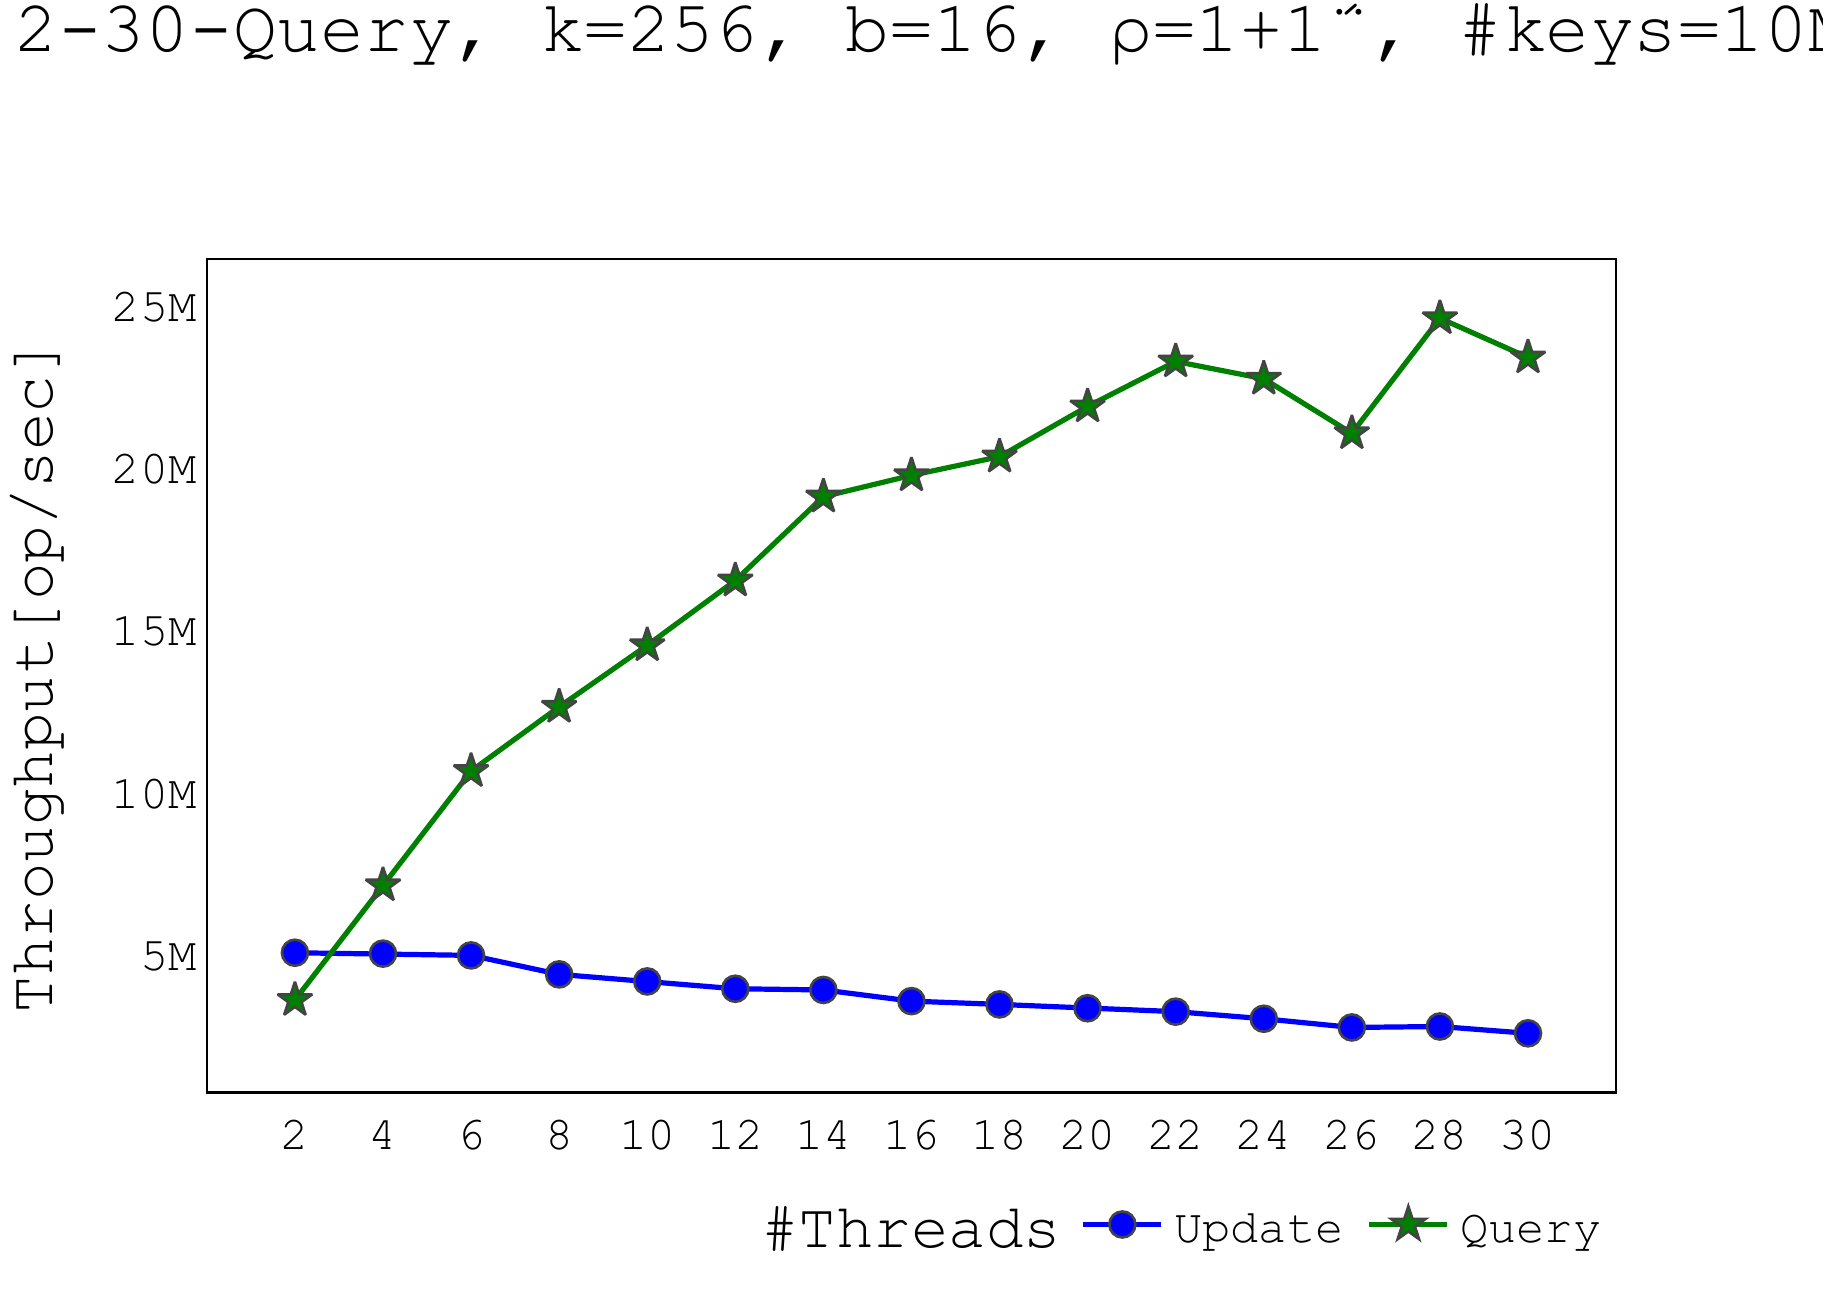}
    \caption{1 update, $\rho=1+\epsilon$, 10M elements.}
    \label{fig: 1update_multi_query_k256_rho_1_1_appendix}
    \end{subfigure}
    \vfill
    \begin{subfigure}[t]{0.49\textwidth}
    \includegraphics[width=\textwidth,trim={0 0.3cm 1.9cm 2.5cm},clip]{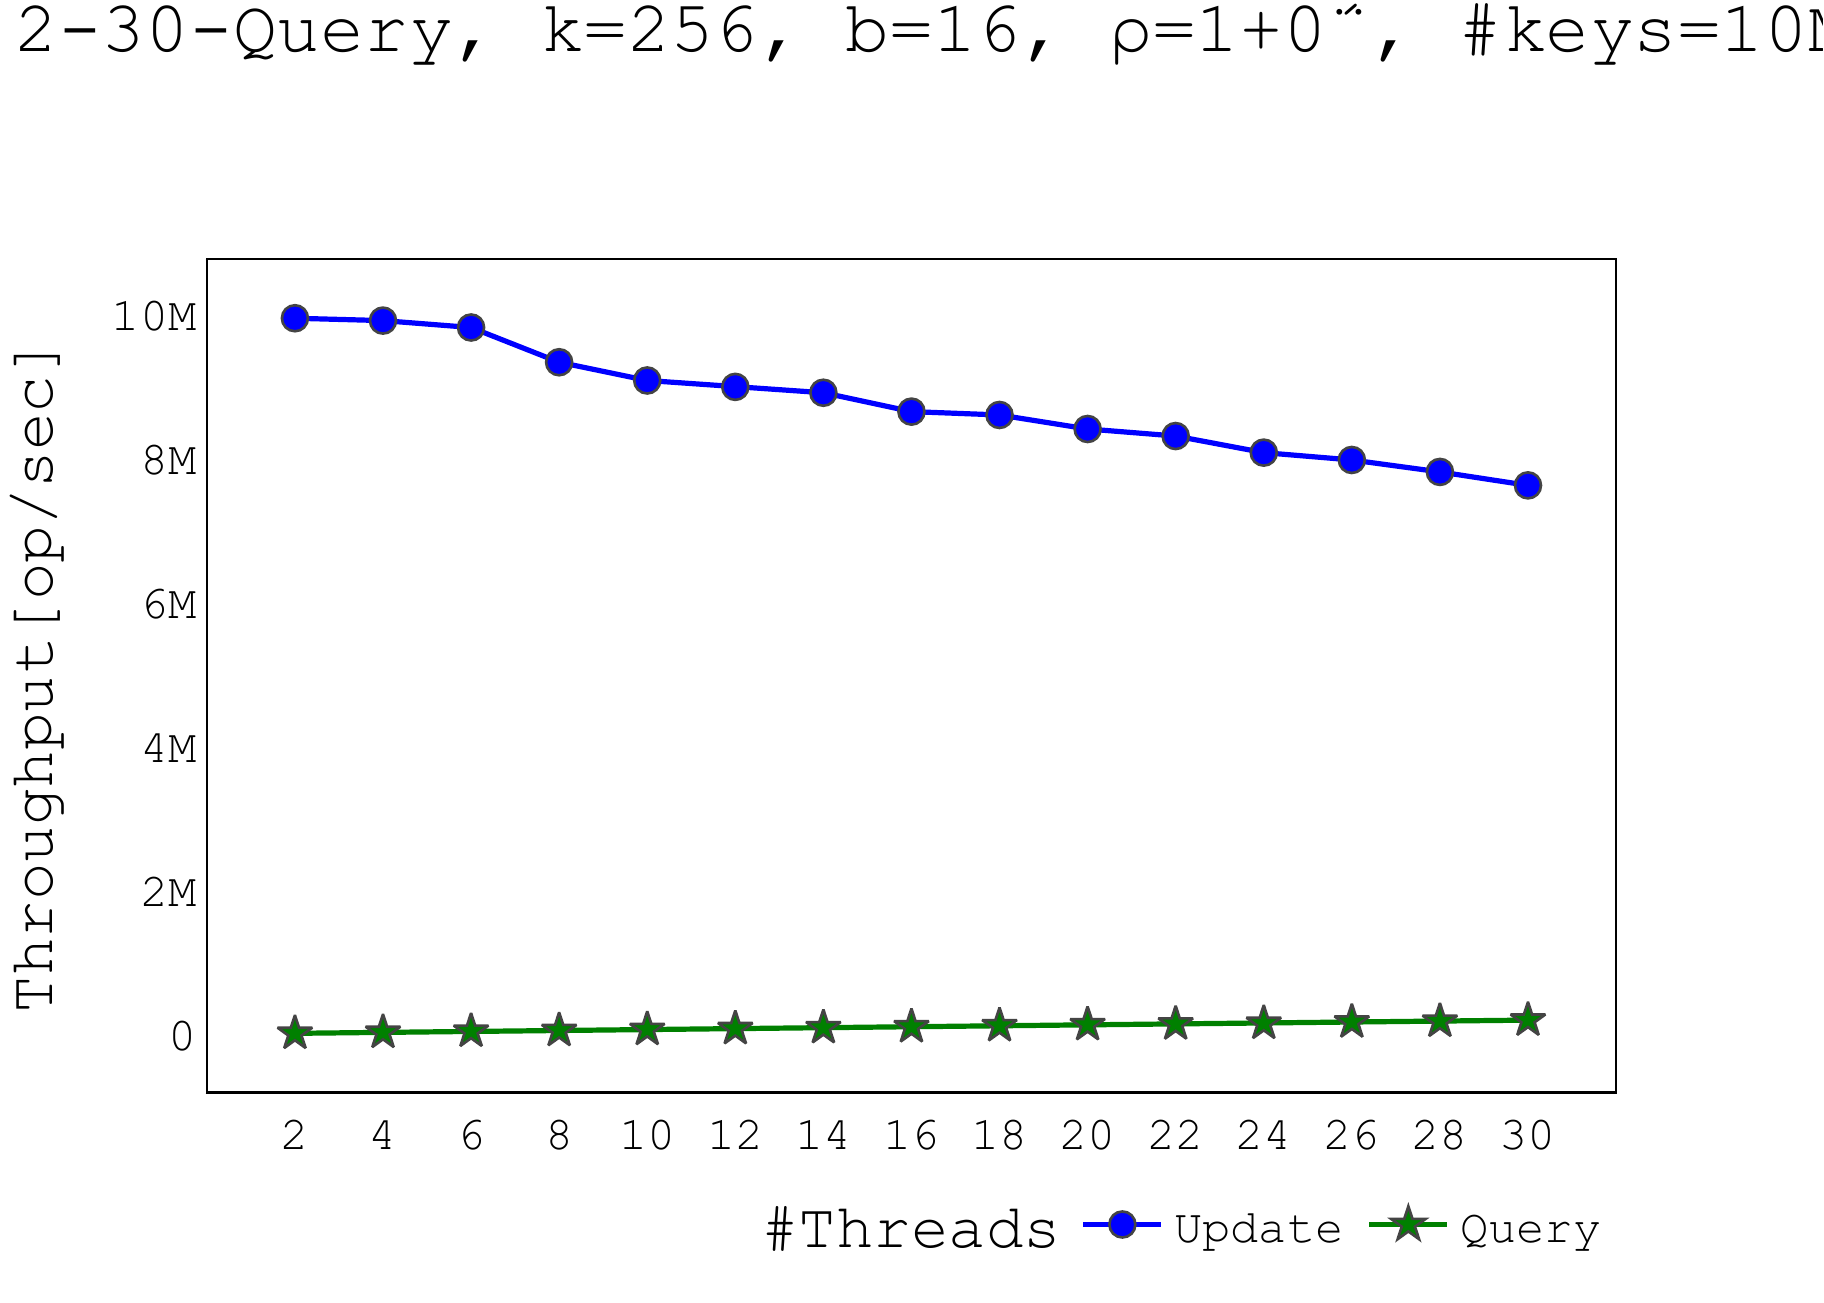}
    \caption{2 update, $\rho=1$, 10M elements.}
    \label{fig: 2update_multi_query_k256_rho_1_0_appendix}
    \end{subfigure}
    \hfill
    \begin{subfigure}[t]{0.49\textwidth}
    \includegraphics[width=\textwidth,trim={0 0.3cm 1.9cm 2.5cm},clip]{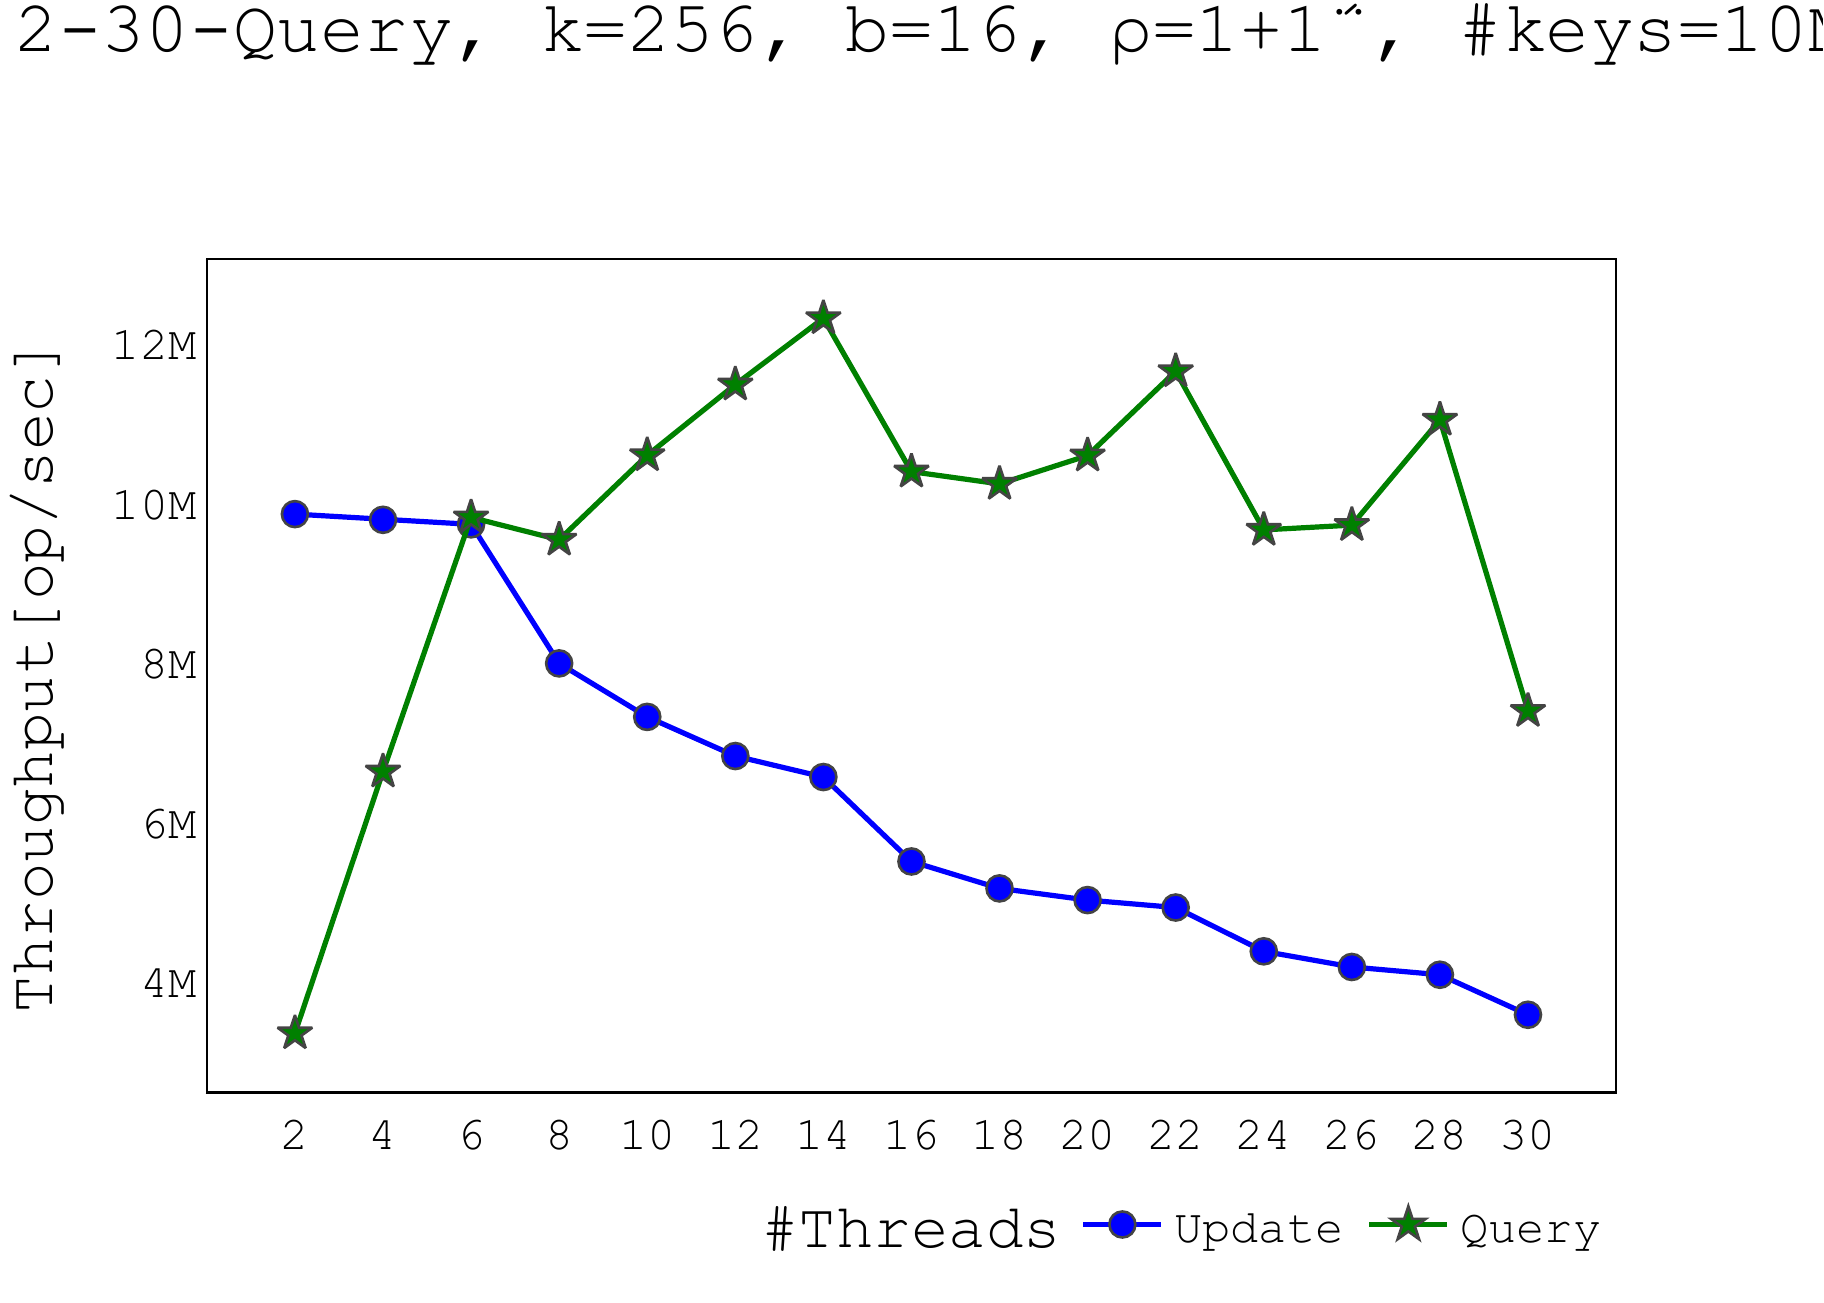}
    \caption{2 update, $\rho=1+\epsilon$, 10M elements.}
    \label{fig: 2update_multi_query_k256_rho_1_1_appendix}
    \end{subfigure}
    \caption{\mysketch 1-2 updates, multiple queries, k = 256.}
    \label{fig: 1_2update_multi_query_k256_rho_appendix}
\end{figure*}
\FloatBarrier

\FloatBarrier
\begin{figure*}[]
 \centering
    \begin{subfigure}[t]{0.49\textwidth}
    \includegraphics[width=\textwidth,trim={0 0.3cm 1.9cm 2.5cm},clip]{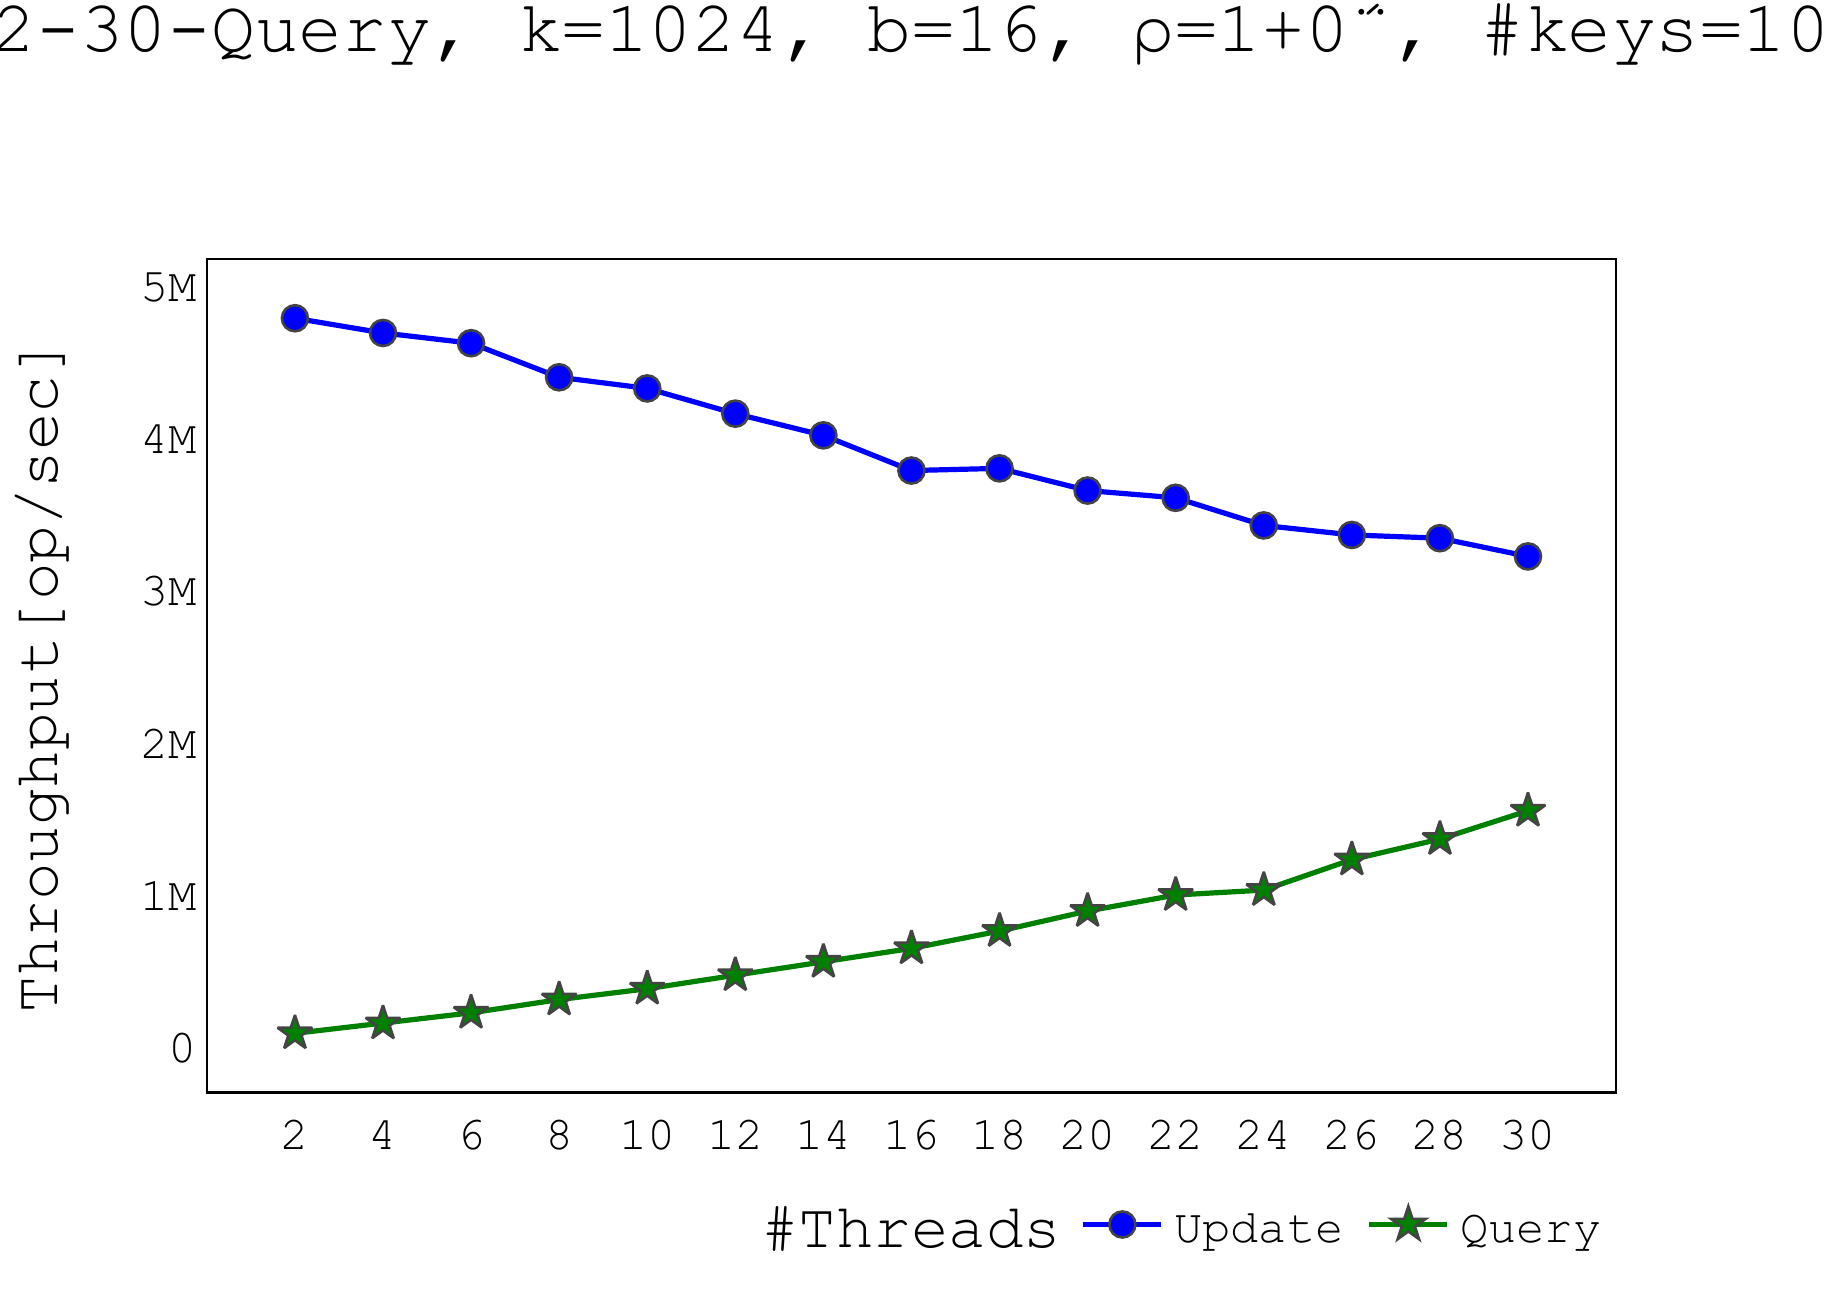}
    \caption{1 update, $\rho=1$, 10M elements.}
    \label{fig: 1update_multi_query_k1024_rho_1_0_appendix}
    \end{subfigure}
    \hfill
    \begin{subfigure}[t]{0.49\textwidth}
    \includegraphics[width=\textwidth,trim={0 0.3cm 1.9cm 2.5cm},clip]{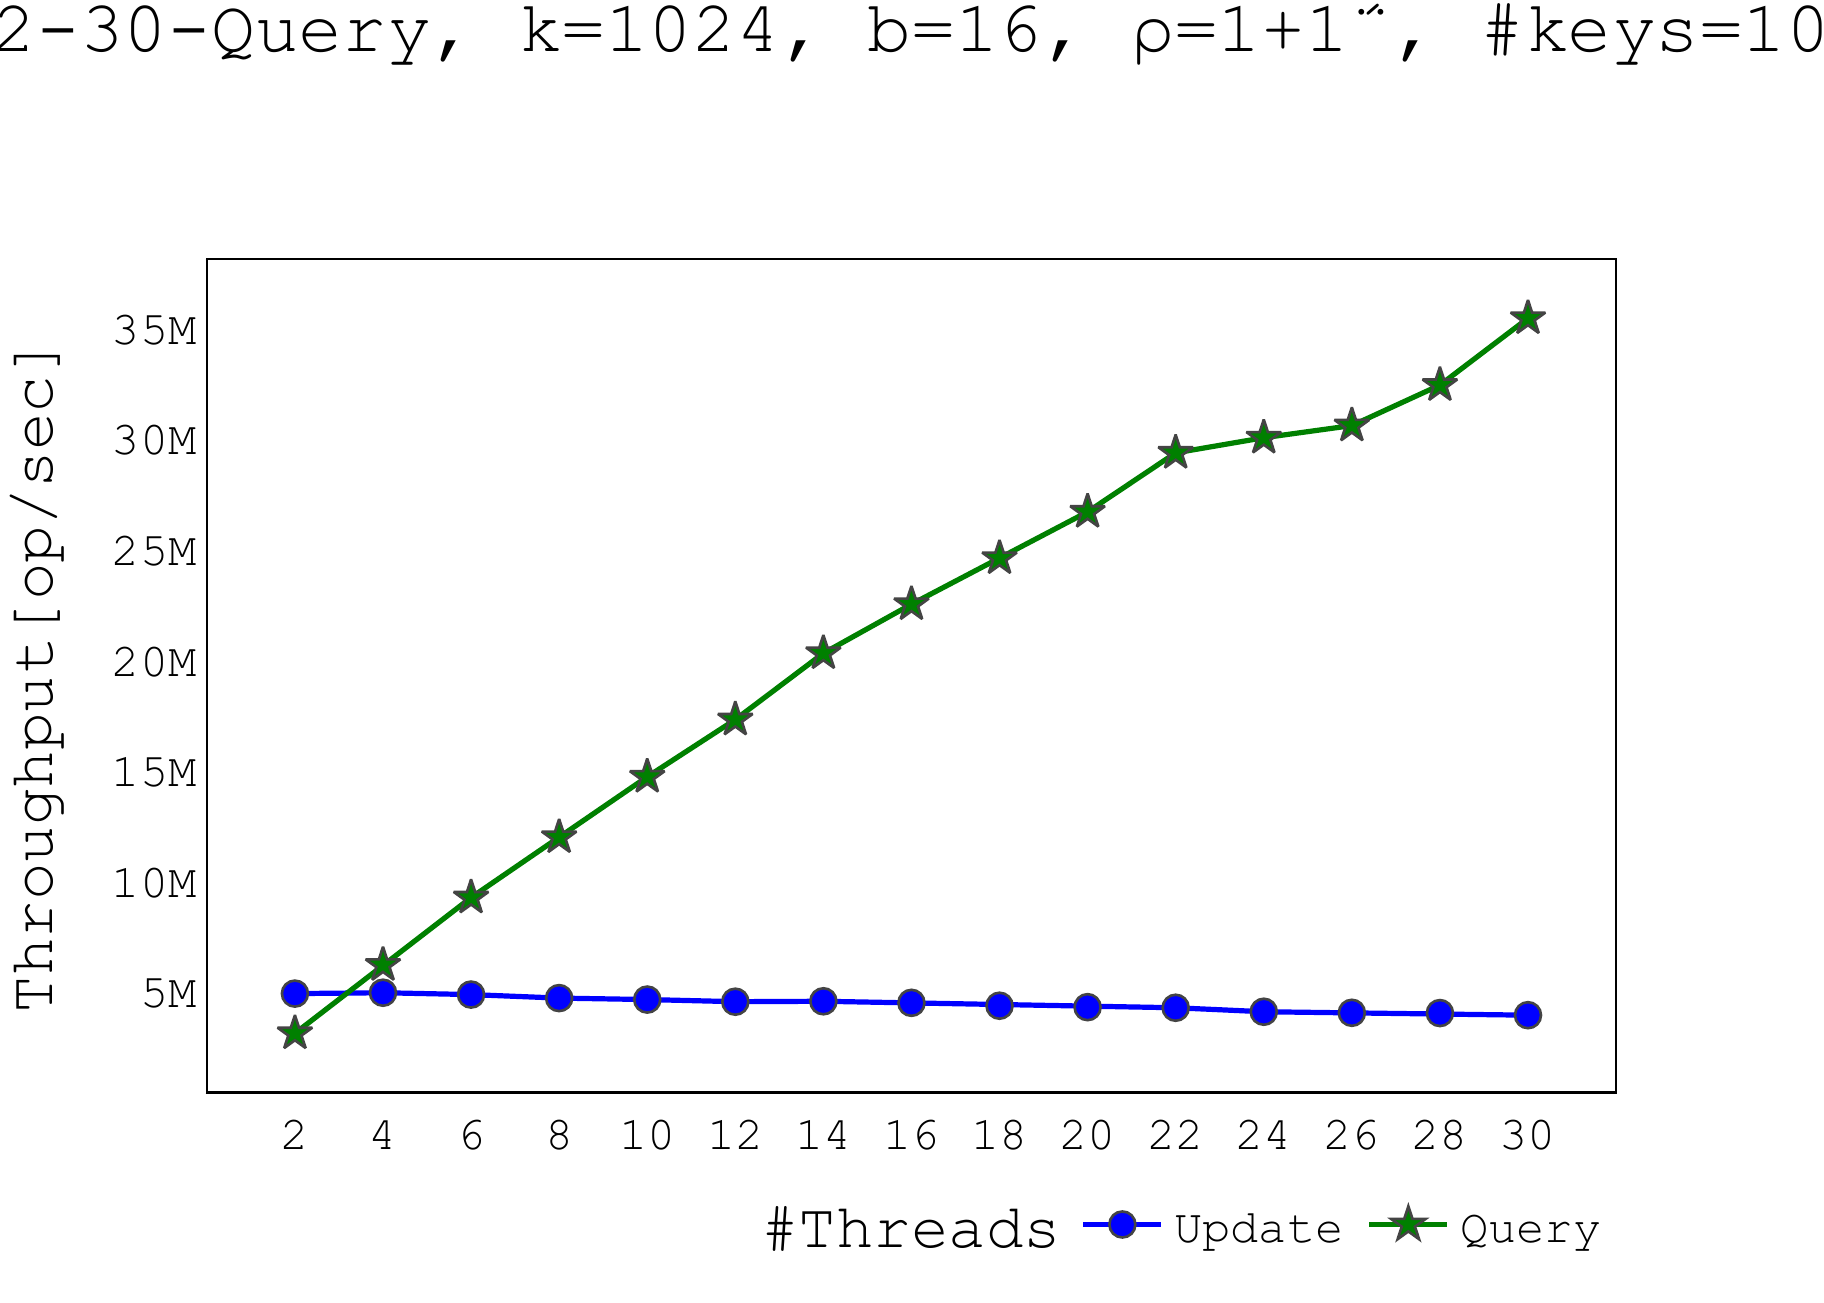}
    \caption{1 update, $\rho=1+\epsilon$, 10M elements.}
    \label{fig: 1update_multi_query_k1024_rho_1_1_appendix}
    \end{subfigure}
    \vfill
    \begin{subfigure}[t]{0.49\textwidth}
    \includegraphics[width=\textwidth,trim={0 0.3cm 1.9cm 2.5cm},clip]{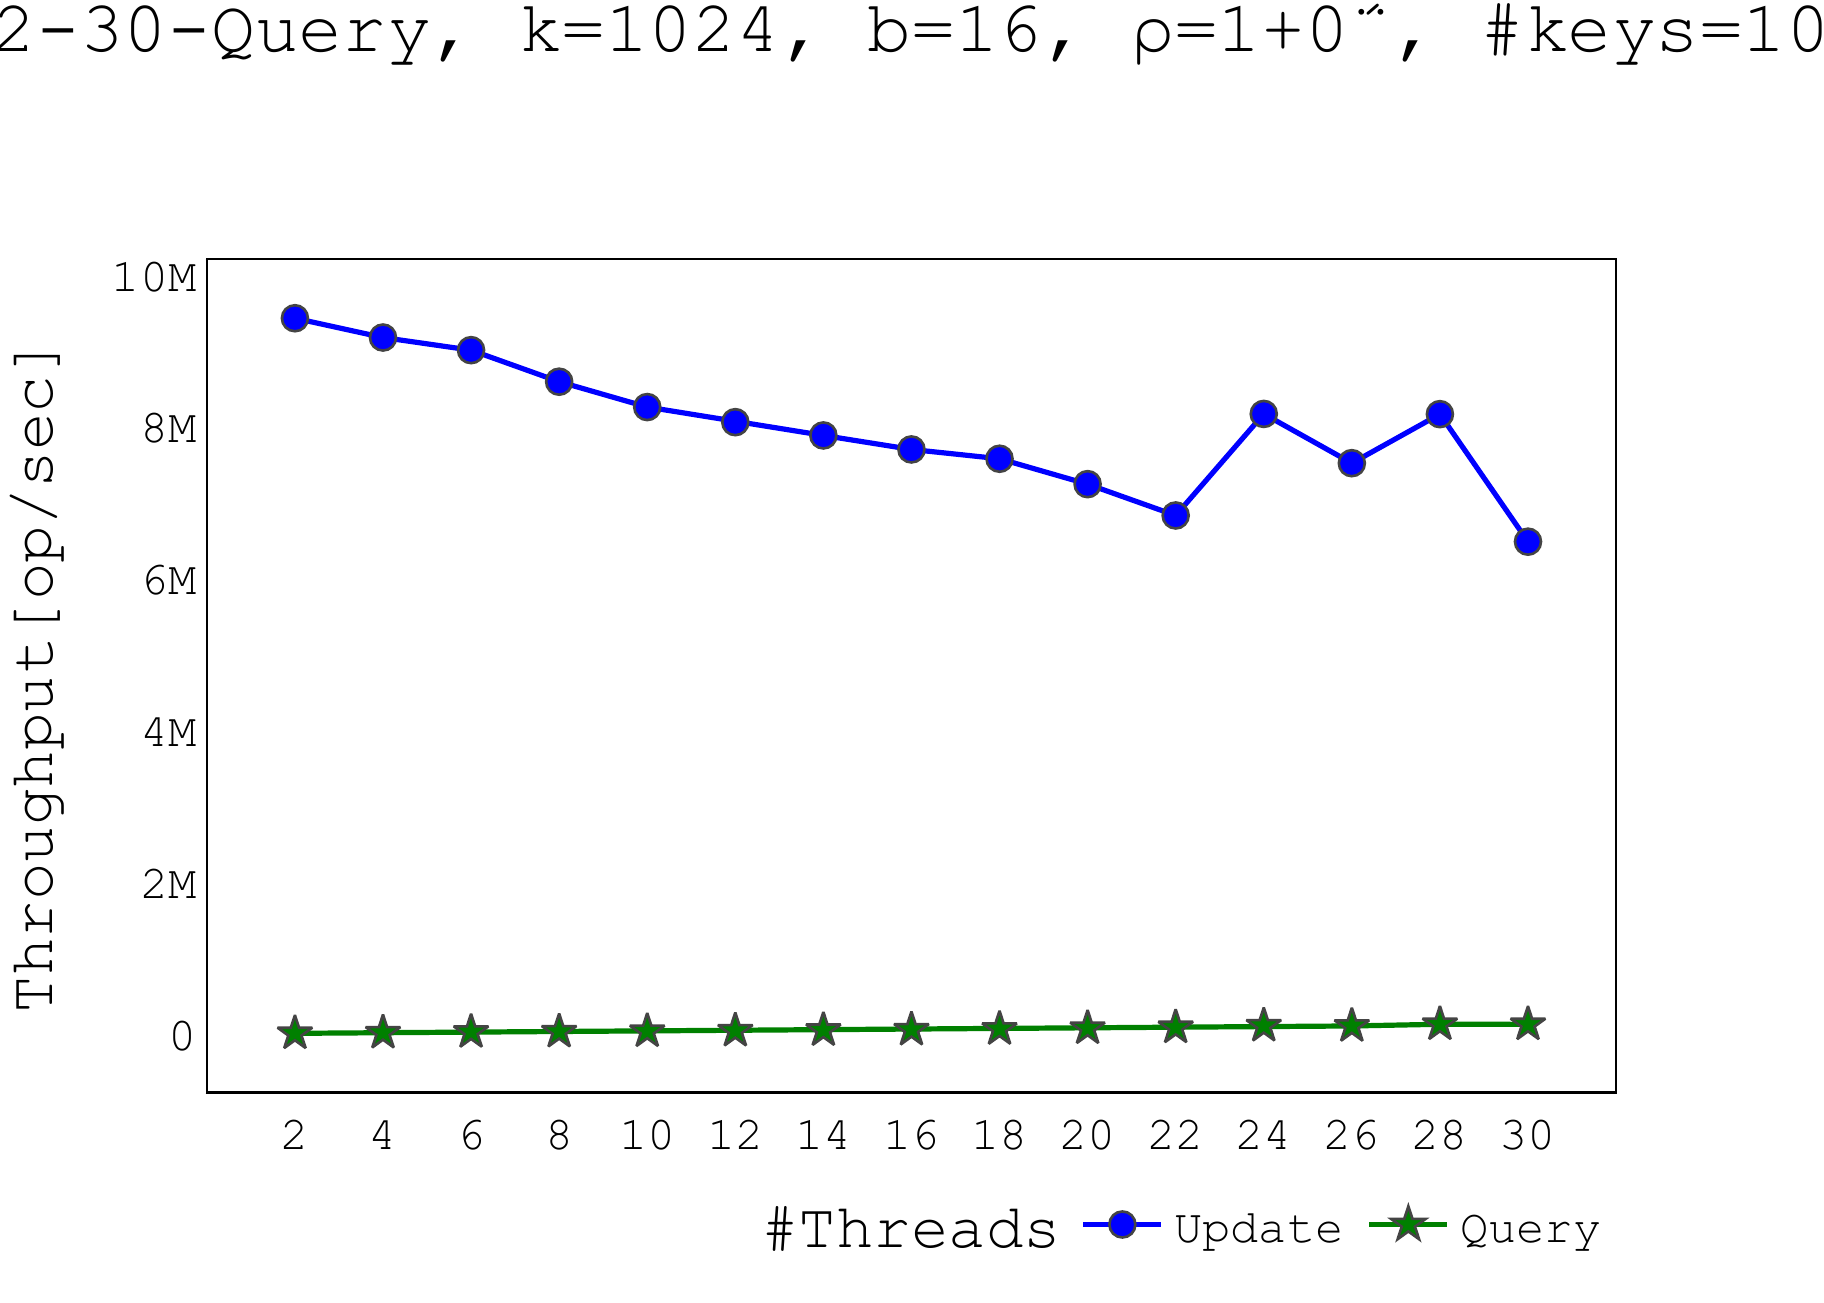}
    \caption{2 update, $\rho=1$, 10M elements.}
    \label{fig: 2update_multi_query_k1024_rho_1_0_appendix}
    \end{subfigure}
    \hfill
    \begin{subfigure}[t]{0.49\textwidth}
    \includegraphics[width=\textwidth,trim={0 0.3cm 1.9cm 2.5cm},clip]{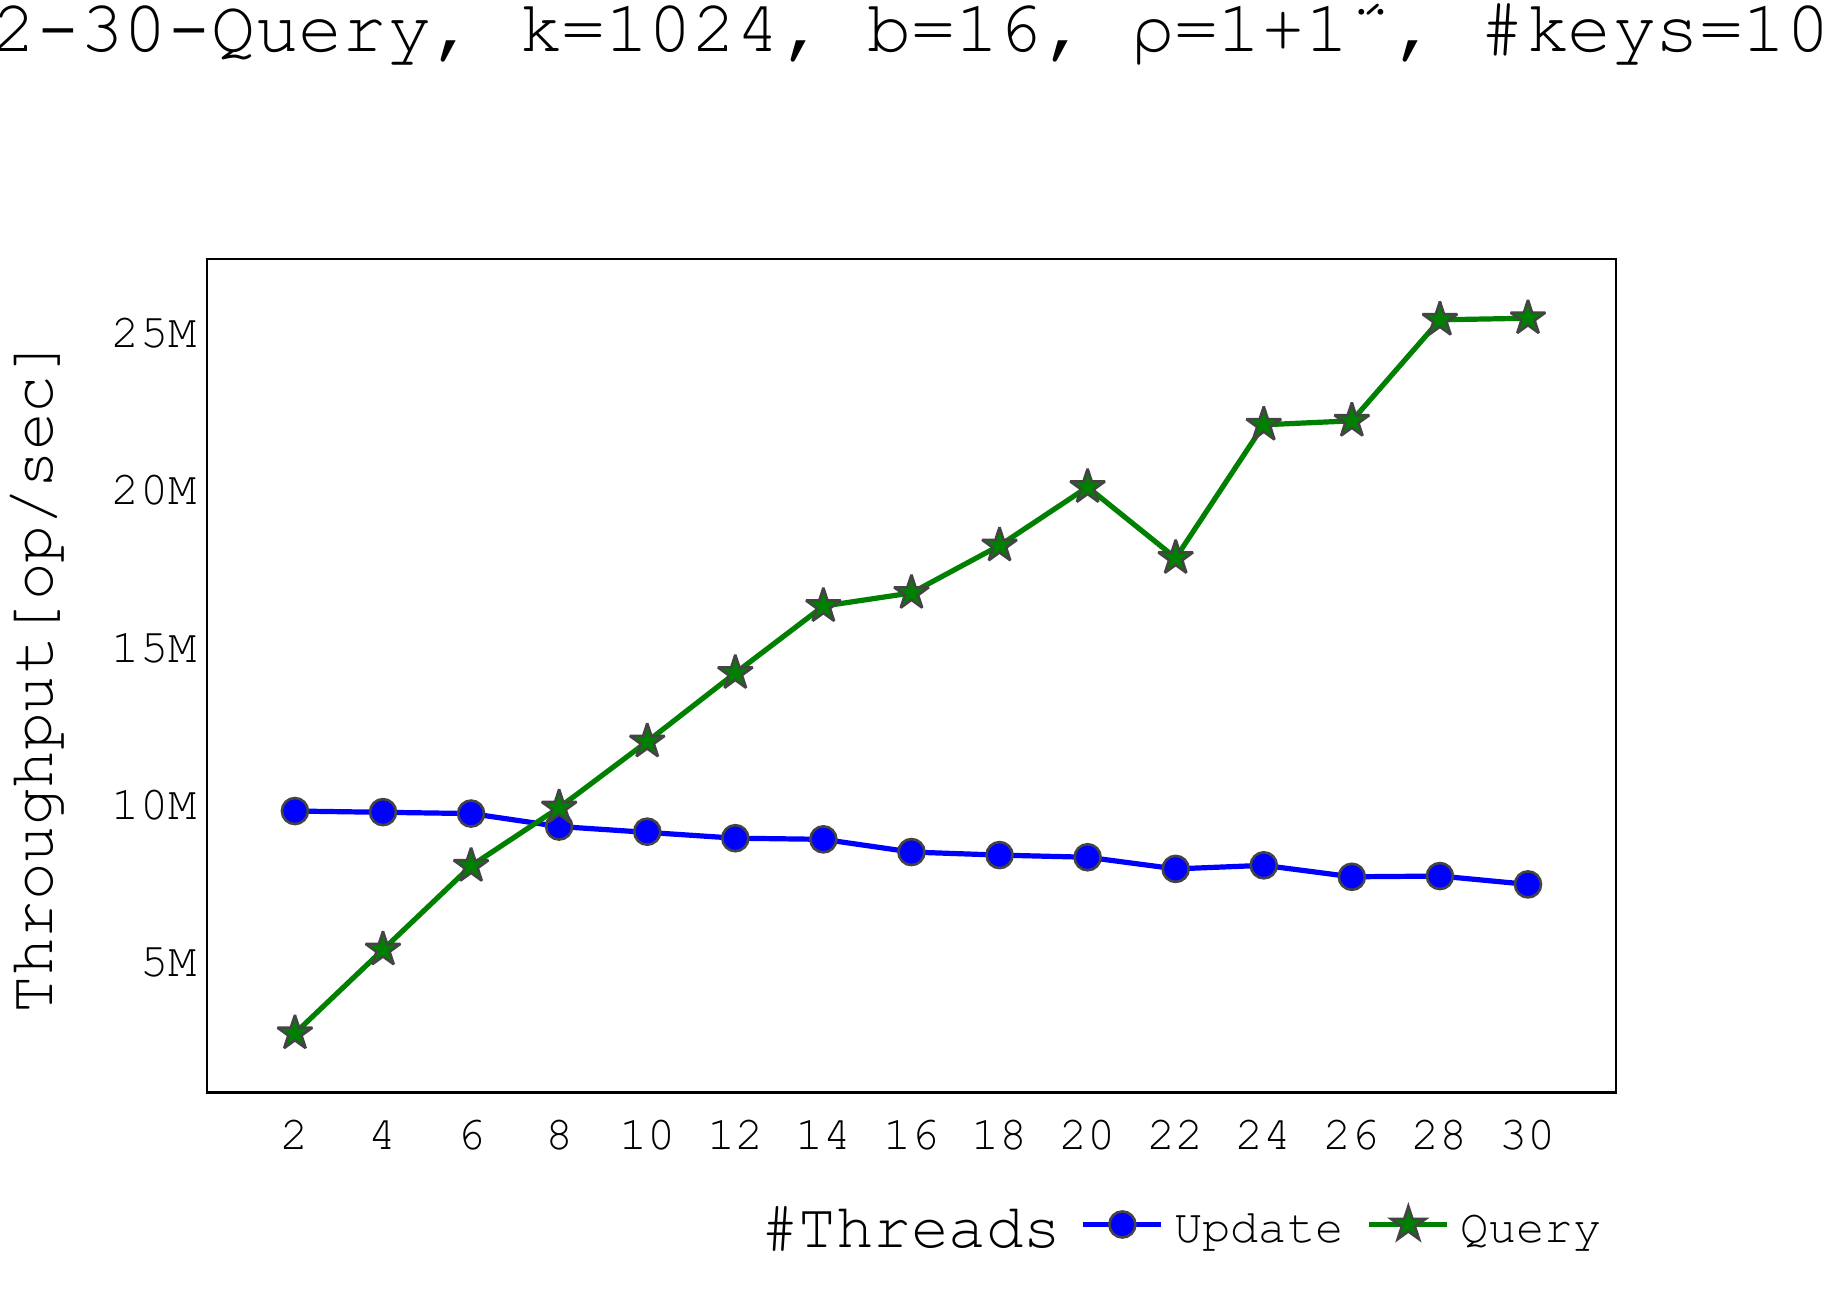}
    \caption{2 update, $\rho=1+\epsilon$, 10M elements.}
    \label{fig: 2update_multi_query_k1024_rho_1_1_appendix}
    \end{subfigure}
    \caption{\mysketch 1-2 updates, multiple queries, k = 1024.}
    \label{fig: 1_2update_multi_query_k1024_rho_appendix}
\end{figure*}
\FloatBarrier

\FloatBarrier
\begin{figure*}[]
 \centering
    \begin{subfigure}[t]{0.49\textwidth}
    \includegraphics[width=\textwidth,trim={0 0.3cm 1.9cm 2.5cm},clip]{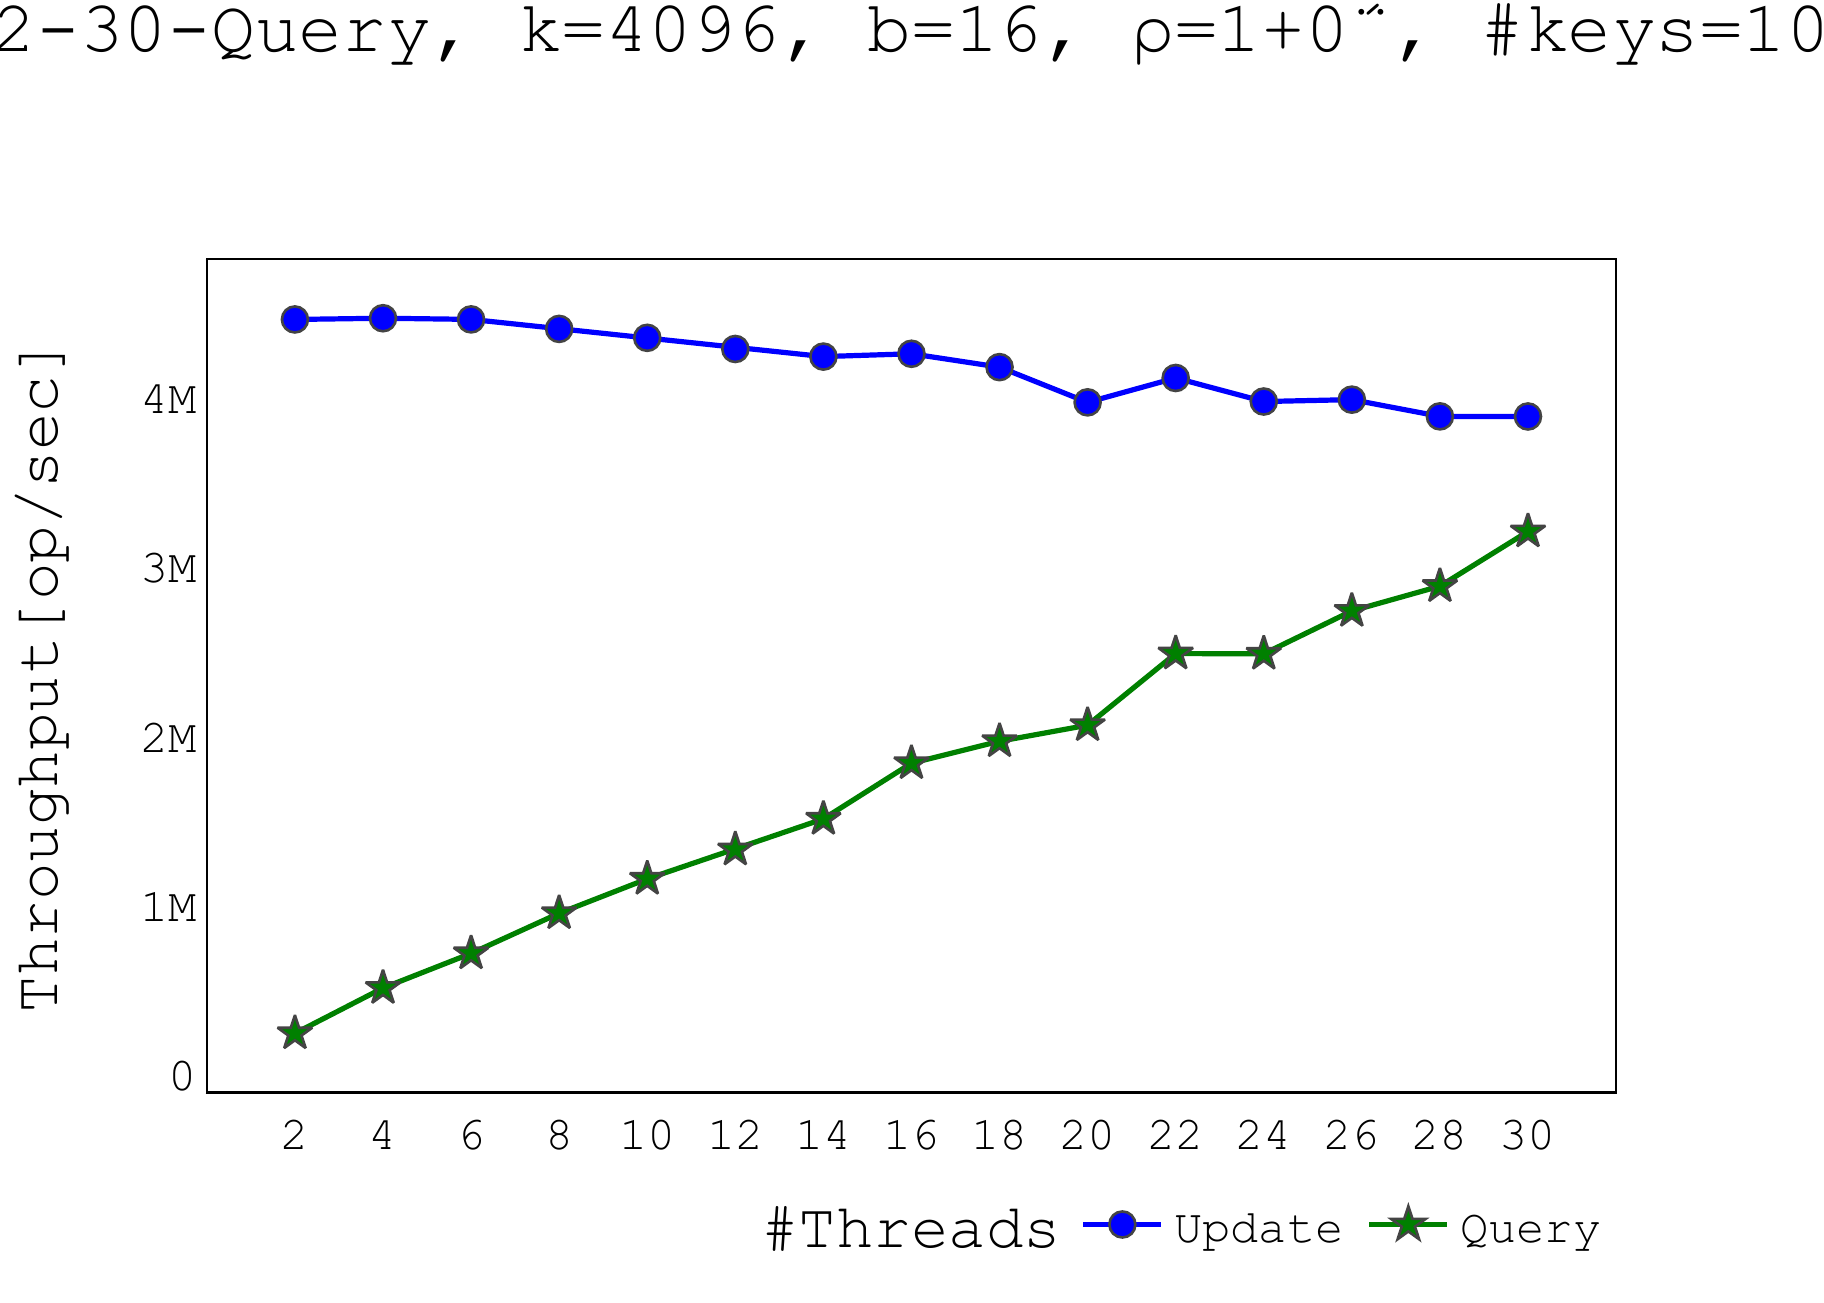}
    \caption{1 update, $\rho=1$, 10M elements.}
    \label{fig: 1update_multi_query_k4096_rho_1_0_appendix}
    \end{subfigure}
    \hfill
    \begin{subfigure}[t]{0.49\textwidth}
    \includegraphics[width=\textwidth,trim={0 0.3cm 1.9cm 2.5cm},clip]{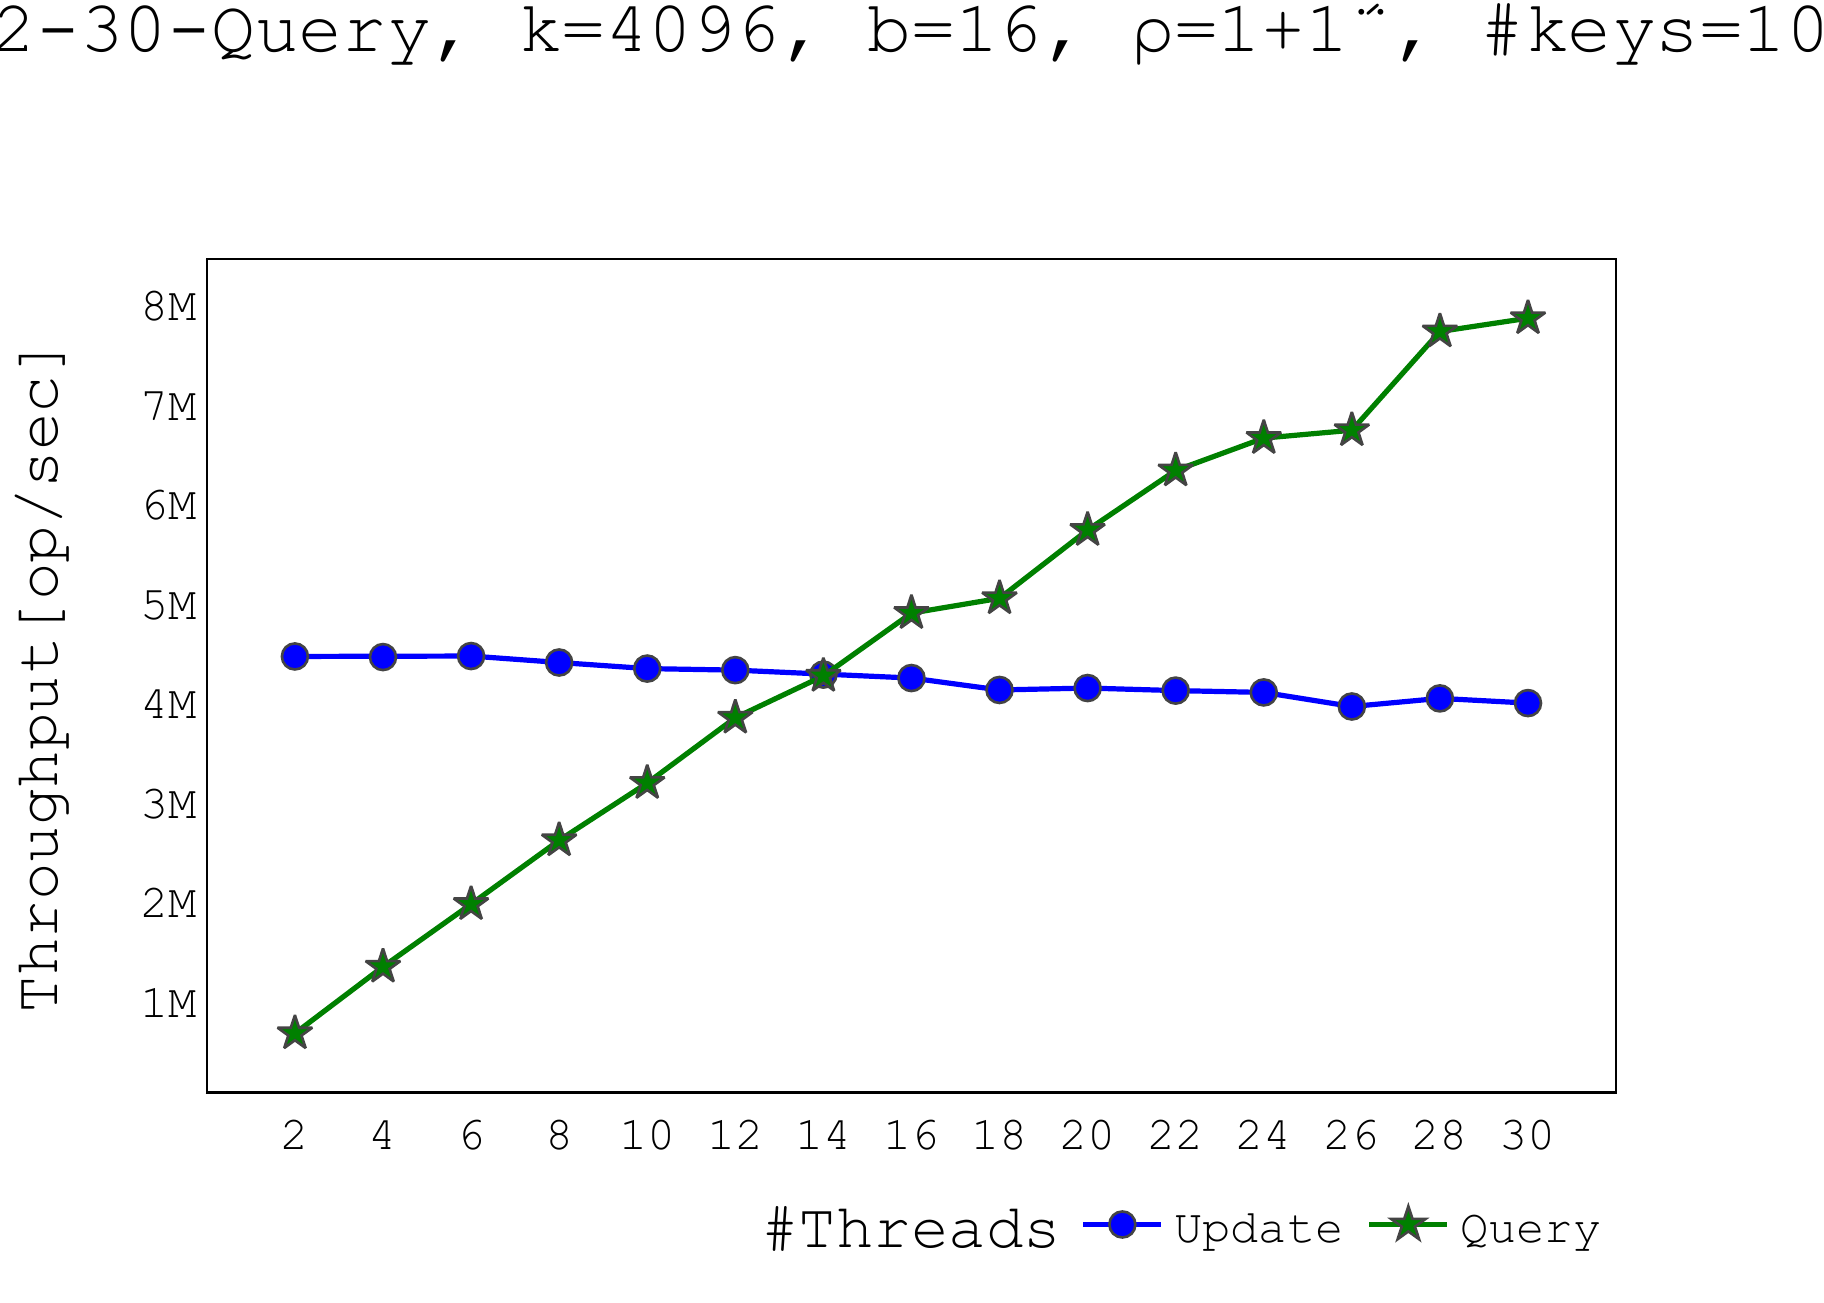}
    \caption{1 update, $\rho=1+\epsilon$, 10M elements.}
    \label{fig: 1update_multi_query_k4096_rho_1_1_appendix}
    \end{subfigure}
    \vfill
    \begin{subfigure}[t]{0.49\textwidth}
    \includegraphics[width=\textwidth,trim={0 0.3cm 1.9cm 2.5cm},clip]{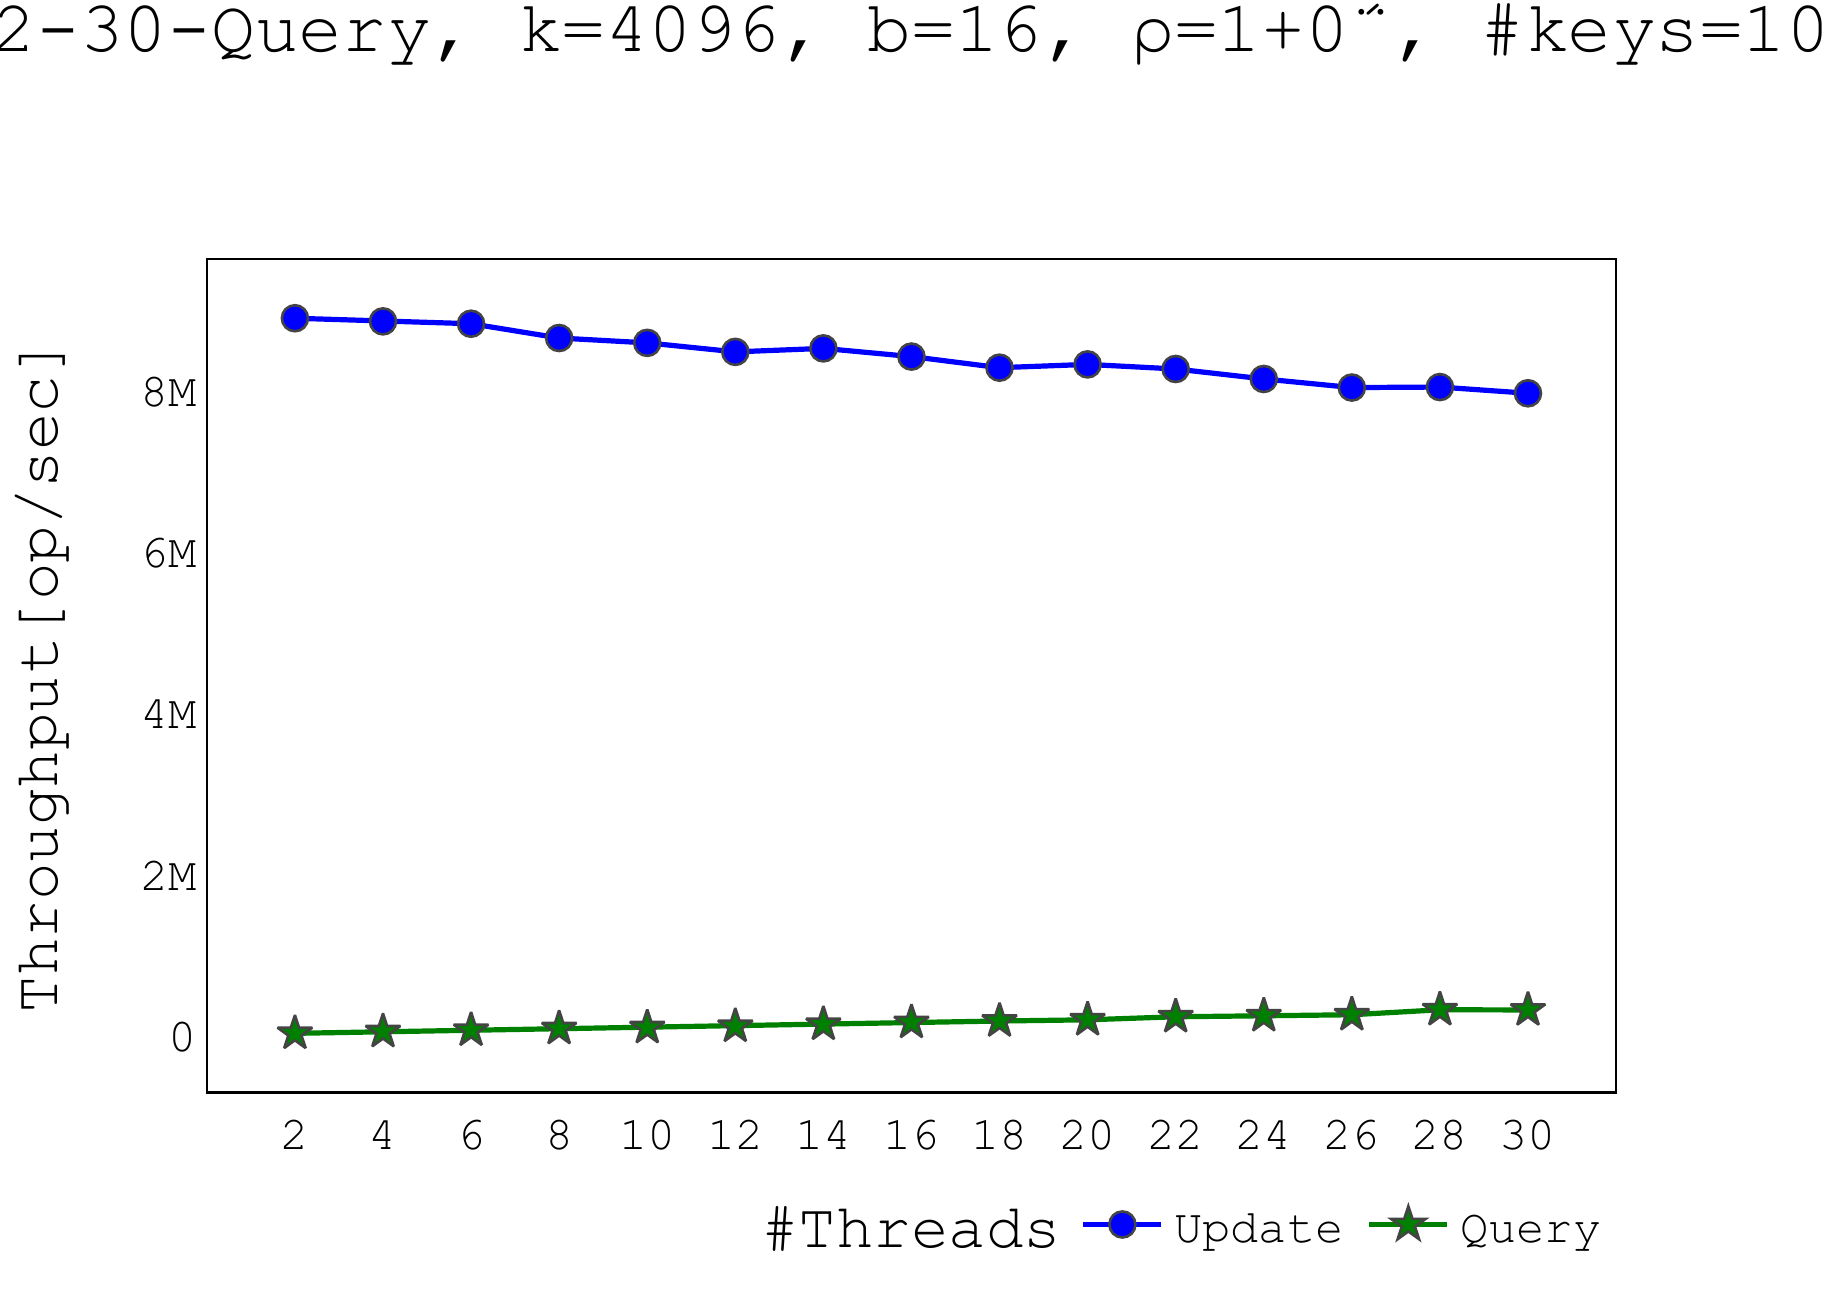}
    \caption{2 update, $\rho=1$, 10M elements.}
    \label{fig: 2update_multi_query_k4096_rho_1_0_appendix}
    \end{subfigure}
    \hfill
    \begin{subfigure}[t]{0.49\textwidth}
    \includegraphics[width=\textwidth,trim={0 0.3cm 1.9cm 2.5cm},clip]{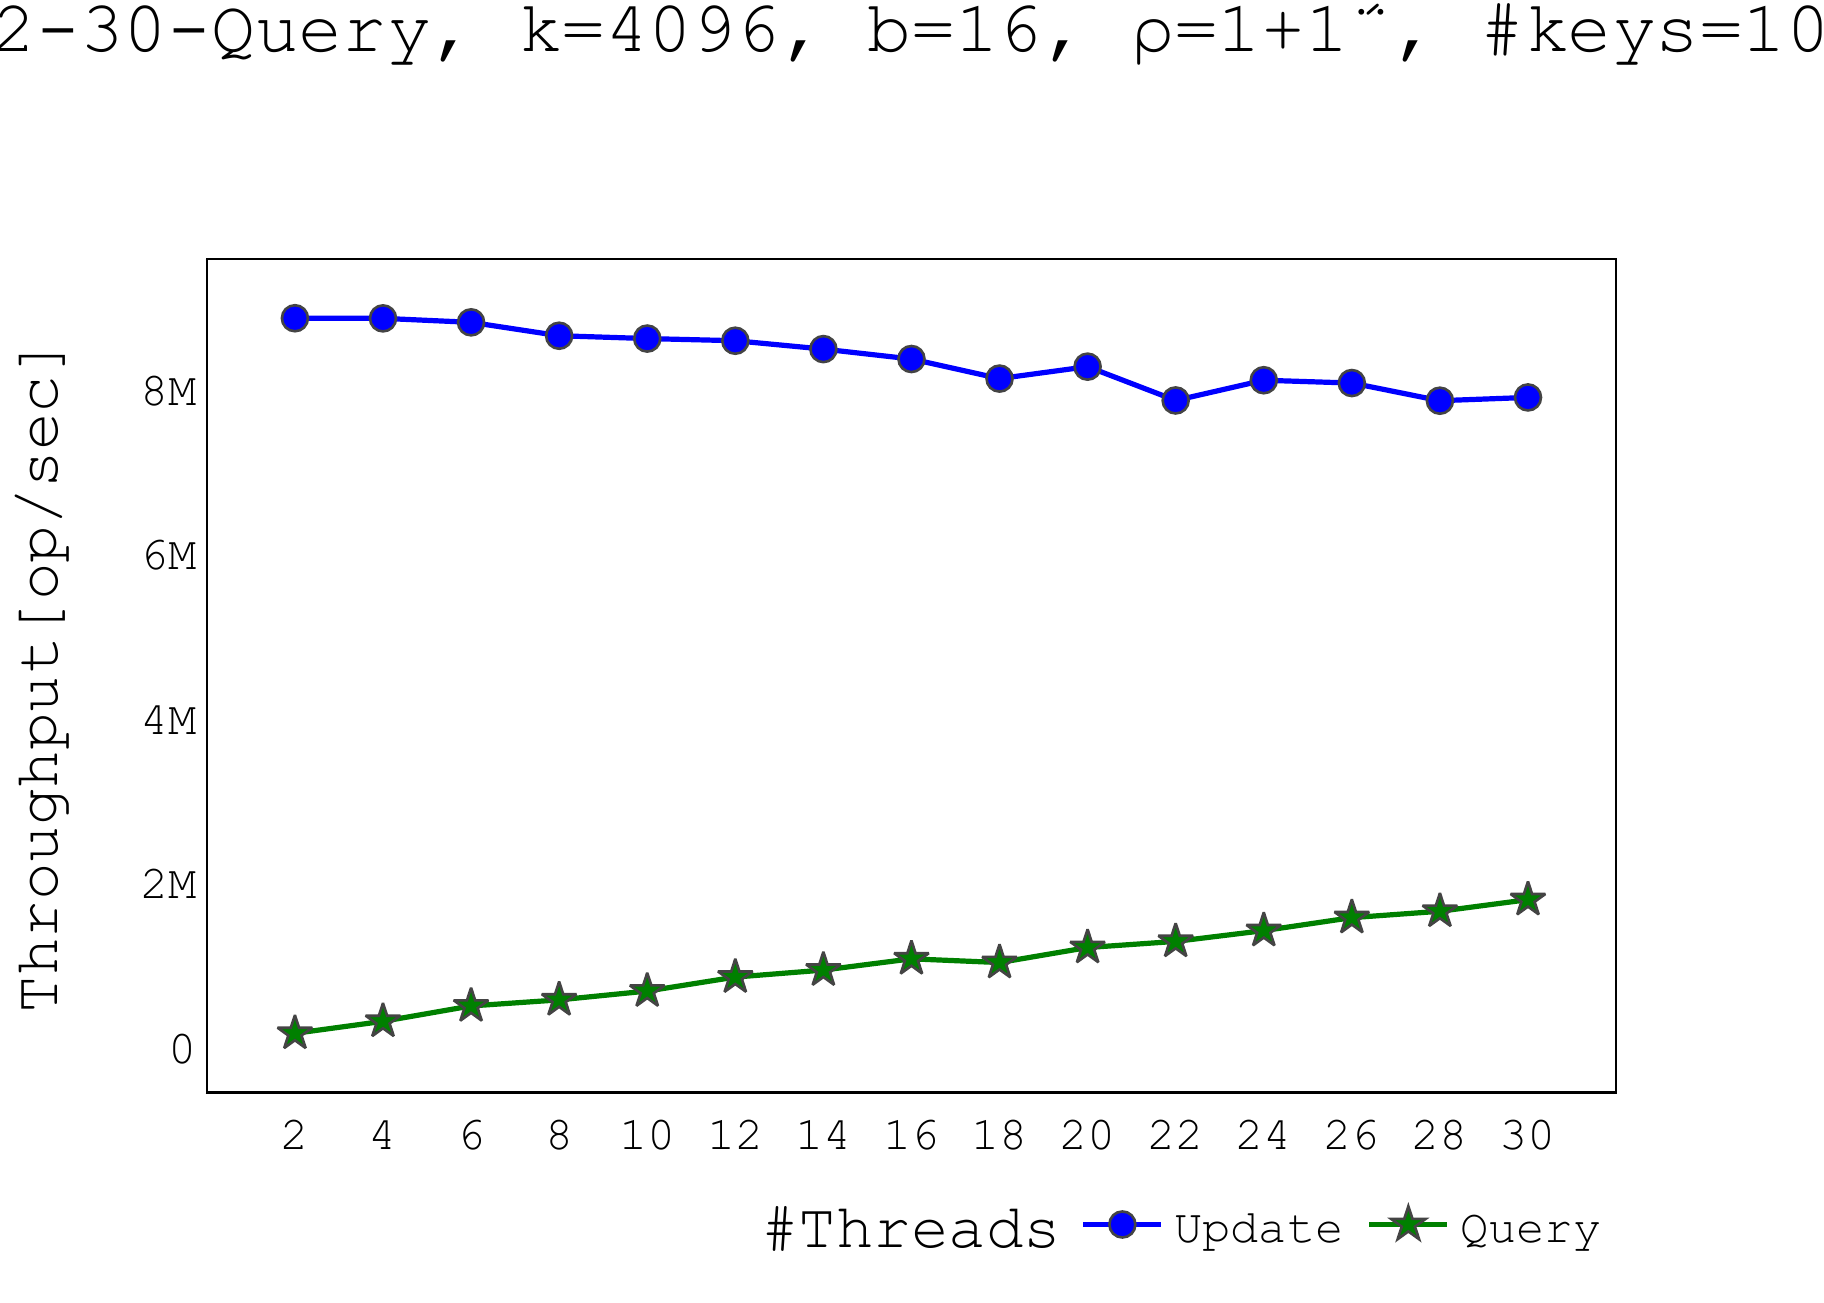}
    \caption{2 update, $\rho=1+\epsilon$, 10M elements.}
    \label{fig: 2update_multi_query_k4096_rho_1_1_appendix}
    \end{subfigure}
    \caption{\mysketch 1-2 updates, multiple queries, k = 4096.}
    \label{fig: 1_2update_multi_query_k4096_rho_appendix}
\end{figure*}
\FloatBarrier
