# Supplementary material for: Quancurrent: A Concurrent Quantiles Sketch
Source: arXiv:2208.09265 source file (2022-08-19)
Supplement: Supplementary file 5 [file holes-analysis-proof.tex]

We now discuss our concurrent Quantiles sketch's error induced by holes.

\subsection{Adversarial Scheduler}
Quantiles sketch implementation (e.g., \cite{mergeables_summaries,Rinberg_2020_fast_sketches}) are sensitive to the processing order. That is, advanced knowledge of the coin flips can increased the error already in the sequential Quantiles sketch. Therefore, we do not consider a strong adversary, but rather discuss only the weak one.

Given a stream \(A = \{x_1, ... , x_n\}\), we refer the stream with holes as \(A'\). Consider a query approximating the $\phi$ quantile.
Consider a summary size of $k_c$, therefore a propagation round happens every $2k_c$ updates.
Let $m$ be the total number of propagation rounds, i.e., $m=n/2k_c$.
Consider some round $j$. Let $h_j \leq h $ be the number of replacements in round $j$. The number of replacements at each round is bounded by
\begin{flalign*}
0 \leq h \leq (N-1)\cdot b
\end{flalign*}
As the duplicated and dropped elements are decided by the adversary, and as we consider only an oblivious adversary, the duplicated and dropped elements are uniformly distributed.
Therefore, the probability that the adversary will choose to replace an element whose rank is smaller than $R$ (the $\phi$ quantile for some $\phi$) is: \[P[\leq R] = \frac{R}{n} = \frac{\phi n}{n} = \phi, \]
And the probability to choose an element whose rank is greater than $R$ is: \[P[\geq R] = \frac{n-R}{n} = \frac{n-\phi n}{n} = 1-\phi \] 

Each replacement \(i\), such that \(0 \leq i \leq h_j\), the overcount error is \(X_{i,j}\).
We consider the error \[\sum_{i=1}^{h_j}X_{i,j} \] of all \(h_j\) \emph{replacements} of round \(j\), ans sum them over all \(m\) rounds.

\(X_{i,j}\) is a uniform random variable that counts the change in \(R\) and its distribution is:
\begin{flalign*}
P[X_{i,j}=1] &= P[duplicate\ element\ with\ rank \leq R]\\
            &    \cdot P[drop\ element\ with\ rank \geq R] = \phi(1-\phi) \\ 
P[X_{i,j}=-1] &= P[duplicate\ element\ with\ rank \geq R]\\
            &   \cdot P[drop\ element\ with\ rank \leq R] = (1-\phi)\phi \\
P[X_{i,j}=0] &= P[duplicate\ element\ with\ rank \leq R]\\
            &   \cdot P[drop\ element\ with\ rank \leq R] \\
            &+ P[duplicate\ element\ with\ rank \geq R]\\
            &   \cdot P[drop\ element\ with\ rank \geq R]= 1-2\phi(1-\phi)
\end{flalign*}
Note that \(|X_{i,j}| \leq 1\) and that
\begin{flalign*}
    \mathbb{E}[X_{i,j}]= 1\cdot \phi(1-\phi) + (-1)\cdot (1-\phi)\phi + 0\cdot (1-2\phi(1-\phi)) = 0
\end{flalign*}

The overcount error is maximized and is minimized at \(\phi=\frac{1}{2}\) so we will assume the distribution of \(X_{i,j}\) is as following:
\begin{flalign*}
X_{i,j} =\begin{cases} 
          1 & w.p \  \frac{1}{4} \\
          -1 & w.p \  \frac{1}{4} \\
          0 & w.p \  \frac{1}{2} \\
          \end{cases}
\end{flalign*}

Quantiles sketches are randomized and at each merge during propagation we retain either the even-indexed elements or odd-indexed elements with equal probability. Since each choice of even/odd is made independently, this produces \(h_j\) independent random variables \(\{X_{1,j},...,X_{h_j,j}\}\) at each round \(j\). Let their total overcount error be denoted \(M_j'\). We bound the probability for each \(X_{i,j} \) to be in the total summary. The probability for a hole to ``survive'' after \(m\) rounds is \(\frac{1}{2}\) to the power of the number of times it was chosen. The number of random choices is bounded below by \({\lfloor \log_{2}{m-j+1} \rfloor}\). 
\begin{flalign*}
 M' &\triangleq \sum_{j=1}^{m}M_j' \\
 M_j &\triangleq \frac{1}{2}^{\lfloor \log_{2}{m-j+1} \rfloor}\sum_{i=1}^{h_j}X_{i,j} \\
 M' &\leq \sum_{j=1}^{m}\frac{1}{2}^{\lfloor \log_{2}{m-j+1} \rfloor}\sum_{i=1}^{h_j}X_{i,j}
\end{flalign*}

We now analyze \(M=\sum_{j=1}^{m}M_j\) using the following Chernoff-Hoeffding bound.

\textbf{Chernoff-Hoeffding bound} given a set \(\{Y_1,...,Y_t\}\) of independent random variables such that \(abs(Y_j-\mathbb{E}[Y_j]) \leq \Upsilon_j\), then for  \(\sum_{j=1}^{t}Y_j\), \[P[abs(T-\sum_{j=1}^{t}\mathbb{E}[Y_j]) > \alpha] \leq 2e^{\frac{-2\alpha^2}{\sum_{j=1}^{t}(2\Upsilon_j)^2}}\]
In our case, the random variables are \(\{M_1,...,M_j\}\), each with \(\mathbb{E}[M_j]=0\) and
\begin{align*}
abs(M_j-\mathbb{E}[M_j]) &= abs(M_j) \\
                         &\leq abs(\frac{1}{2}^{\lfloor \log_{2}{m-j+1} \rfloor+1}\sum_{i=1}^{h_j}X_{i,j})\\
                        &\leq \frac{1}{2}^{\lfloor \log_{2}{m-j+1} \rfloor+1}\sum_{i=1}^{h_j}|X_{i,j}| && |X_{i,j}|\leq 1\\
                        &\leq \frac{1}{2}^{\lfloor \log_{2}{m-j+1} \rfloor+1}h_j\\
                        &= 2^{\lfloor-\log_{2}{m-j+1} \rfloor+1}h_j && x<\lfloor x \rfloor+1\\
                        &< 2^{-\log_{2}{m-j+1}}h_j\\
                        &= \frac{h_j}{(m-j+1} && h_j\leq h\\
                        &\leq \frac{h}{(m-j+1}
\end{align*}

Setting \(\alpha=z\cdot m\) for some parameter \(z\):
\begin{align*}
    Pr[abs(M)>\alpha] 
                      &\leq2exp\left(\frac{-2h^2m^2}{\sum_{j=1}^{m}\left(\frac{2h_j}{m-j+1}\right)^2}\right)\\
                      &= 2exp\left(\frac{-2h^2m^2}{4h^2\sum_{j=1}^{m}\left(\frac{1}{m-j+1}\right)^2}\right) && t\triangleq m-j+1\\
                      &= 2exp\left(\frac{-z^2m^2}{2h^2\sum_{t=1}^{m}\left(\frac{1}{t^2}\right)}\right) && \sum_{t=1}^{\infty}\left(\frac{1}{t^2}\right)\approx \frac{\pi^2}{6}\leq2\\
                      &\leq 2exp\left(\frac{-z^2}{4h^2}\right)\\
\end{align*}
Thus if we set \(z=2h\sqrt{\ln{\frac{2}{\delta_c}}}\), with probability at least \(1-\delta_c\) we have \[abs(M)<zm=z\cdot\frac{n}{2k_c}\]
Thus for \(k_c=\frac{h}{\epsilon}\sqrt{\ln{\frac{2}{\delta_c}}}\) the error will be smaller than \(\epsilon_c n\), as desired.

Given a stream with $A'$ with holes, and summary of size \(k_c=\frac{h}{\epsilon_c}\sqrt{\ln{\frac{2}{\delta_c}}}\), let \(R_c\) be the rank returned by the query such that \(R_c \in [R-\epsilon_c,R+\epsilon_c]\): 
\begin{equation} \label{Eq:conc_rank}
    R-\epsilon_c \leq R_c \leq R+\epsilon_c \qquad\text{w.p.}\quad 1-\delta_c
\end{equation}

Agarwal et al. showed that any implementation of the sequential quantiles sketch, with summary size \(k_s=\frac{1}{\epsilon_s}\sqrt{\ln{\frac{2}{\delta_s}}}\), returns an element whose rank is between \((\phi-\epsilon_s)n\) and \((\phi+\epsilon_s)n\) with probability at least \(1-\delta_s\) for some parameters \(\epsilon_s\) and \(\delta_s\)~\cite{mergeables_summaries}. Let \(R_s\) be the rank returned by the query such that \(R_s \in [R_c-\epsilon_s,R_c+\epsilon_s]\):
\begin{equation} \label{Eq:seq_rank}
    R_c-\epsilon_s \leq R_s \leq R_c+\epsilon_s \qquad\text{w.p.}\quad 1-\delta_s
\end{equation}

\begin{theorem}
There exists a concurrent quantiles sketch that computes an \(\epsilon-approximation\) for the \({\phi}-th\) quantile of a stream with n elements. For an error parameter \(0<\epsilon<1\), returns an element whose rank is in \([({\phi}-\epsilon)n,(\phi+\epsilon)n]\) with probability at least \(1-\delta\)
\end{theorem}

We assume for simplicity \(\delta_c=\delta_s=\delta'\) and \(\epsilon_c=\alpha\epsilon_s\) for some parameter \(\alpha>0\).
We define the summary size \(k=\max\{k_s,k_c\}\) and set the error parameter \(\epsilon=\epsilon_c+\epsilon_s\).

\begin{equation}\label{Eq: max_k}
\begin{split}
    k = \max\{k_s,k_c\} &= \max\left\{\frac{1}{\epsilon_s}\sqrt{\ln{\frac{2}{\delta'}}},\frac{h}{\epsilon_c}\sqrt{\ln{\frac{2}{\delta'}}}\right\} \\
    &= \max\left\{\frac{1}{\epsilon_s}\sqrt{\ln{\frac{2}{\delta'}}},\frac{h}{\alpha\epsilon_s}\sqrt{\ln{\frac{2}{\delta'}}}\right\}\\
    &= \max\left\{\frac{1+\alpha}{\epsilon}\sqrt{\ln{\frac{2}{\delta'}}},\frac{h(1+\alpha)}{\alpha\epsilon}\sqrt{\ln{\frac{2}{\delta'}}}\right\}
\end{split}
\end{equation}

 We want to minimize the summary size k. 
 
\begin{equation}\label{Eq: max_k_cases}
\begin{split}
k =\begin{cases} 
          \frac{1+\alpha}{\epsilon}\sqrt{\ln{\frac{2}{\delta'}}}&  \  \alpha \leq h \\
          \frac{h(1+\alpha)}{\alpha\epsilon}\sqrt{\ln{\frac{2}{\delta'}}} &  \  0 < \alpha < h \\
          \end{cases}
\end{split}
\end{equation}

\begin{equation*}\label{Eq: k_derv}
\begin{split}
 \frac{\partial k}{\partial \alpha} =\begin{cases} 
          \frac{1}{\epsilon}\sqrt{\ln{\frac{2}{\delta'}}}&  \  h \leq \alpha \ \text{function increasing} \\
          \frac{-h}{\alpha^2\epsilon}\sqrt{\ln{\frac{2}{\delta'}}} &  \  0 < \alpha < h  \ \text{function decreasing} \\
          \end{cases}
\end{split}
\end{equation*}

The non-differentiable point \(\alpha=h\) is where k is minimised. We will show it by taking 3 points, one point from each interval. 
\begin{equation*}\label{Eq: non_differential}
\begin{split}
k =\begin{cases} 
          \frac{2+h}{\epsilon}\sqrt{\ln{\frac{2}{\delta'}}}&  \  \alpha = \frac{h}{2} \\
          \frac{1}{\epsilon}\sqrt{\ln{\frac{2}{\delta'}}}&  \  \alpha = h \\
          \frac{(1+2h)}{\epsilon}\sqrt{\ln{\frac{2}{\delta'}}} &  \  \alpha = 2h \\
          \end{cases}
\end{split}
\end{equation*}

Note that \(k = k_c = k_s\), therefore 

\begin{equation} \label{Eq: eps_ration}
    \epsilon_s = \frac{\epsilon_c}{h}
\end{equation}

With probability at least \((1-\delta')^2\), using \ref{Eq:conc_rank} and \ref{Eq:seq_rank}, 
\begin{equation} \label{Eq:seq_conc_rank}
  R-(\epsilon_c+\epsilon_s) \leq  R_c-\epsilon_s \leq R_s \leq R_c+\epsilon_s \leq R+(\epsilon_c +\epsilon_s)
\end{equation}

We define \(\delta \triangleq 2\delta'-{\delta'}^2 \), and then with probability at least \(1-\delta\):
\begin{equation} \label{Eq: error_range}
    R_s \in [R-\epsilon,R+\epsilon]
\end{equation}

We showed above that under an adversarial scheduler our concurrent sketch's error induced by holes is coarsely bounded by $h$ times that of the corresponding sequential sketch, where $h$ is a bound on the number of holes in a batch. That is, the number of holes can be massive. 

\subsection{Stochastic Scheduler}

We now analyze the number of holes under the assumption of a fair scheduler. As we explained in Sections \ref{Section: part1_update}-\ref{Section: part2_batch_update}, our concurrent algorithm is essentially a "batched streaming" algorithm. A buffer of $2k$ elements is "batched updated" into the sketch's first level. Denote by $H$ the total number of holes in a batch. A $2k$ sized G\&SBuffer's array is split into $2k/b$ slots, where $k$ is the sketch's summary size and $b$ is the size of threads local buffers. Denote by $H_1,\dots, H_{2k/b}$ the number of holes in slot $1, \dots, H_{2k/b}$, respectively.

Threads insert elements to the G\&SBuffer in slots. A slot $j$ is written by the thread who successfully incremented the shared index from $j$ to $j+b$, we refer this thread as $T_j$. The owner thread, $T_O$, is the last to increment the shared index. To initiate a batch update, $T_O$ needs to create a local copy of the G\&SBuffer's array, i.e., after copying its own local buffer's element, the owner thread reads the G\&SBuffer's array, starting from the first slot. For a hole to be read in some slot $j$, the owner thread, must read an index in this slot, before the write thread $T_j$ writes the corresponding index in the slot.

\paragraph*{Analysis of $\boldsymbol{H_1}$.} We first analyze $H_1$. We assume an extreme, high unlikely scenario in which $T_O$ incremented the index from $\frac{2k}{b}-1$ to $\frac{2k}{b}$ and thread $T_1$ hasn't copied any value from its local buffer to the first slot, yet. In this instance, $T_O$ must overtake $T_1$, i.e., $T_O$ must write $b$ values (copy its own local buffer) and then read values from slot $1$ overtaking $T_1$. If $T_O$ is scheduled $b+1$ times before $T_1$, it reads the first index before $T_1$ writes it, reading a hole. If $T_1$ executes $1$ write, $T_O$ must execute an additional read to overtake $T_1$. Generalized, for every $i$ writes by $T_1$, $T_O$ must execute a $i+1$ reads to read at least one hole. The probability that $T_O$ reads at least $1$ hole in slot $1$ is bounded by:
\[P_1 = {3b \choose b} \cdot \left(\frac{1}{2}\right)^{3b}+\sum_{i=0}^{b-1} {b+2i+1 \choose i} \cdot \left(\frac{1}{2}\right)^{b+2i+1}\]

Note that we double count multiple schedules, therefore this is an upper bound on the probability that $T_O$ reads at least $1$ hole. Furthermore, we have assumed that $T_1$ hasn't executed any writes yet. Note that if $T_1$ has started writes, the probability that $T_O$ reads holes is even lower. The mean of the total number of holes in slot $1$ is:
\[E\left[H_1\right]= P(H_1=0)\cdot 0 + P(H_1=1)\cdot 1 + \dots + P(H_1=b)\cdot b\]
$T_O$ can read at most $b$ holes, therefore
\[E\left[H_1\right] \leq b \left( P(H_1=0) + P(H_1=1) + \dots + P(H_1=b) \right) = b\cdot P(H_1\geq1) \leq b\cdot P_1\]
For $b=16$, $E\left[H_1\right] \leq 0.039 \cdot 16 = 0.624$.

\paragraph*{Analysis of $\boldsymbol{H_j}$.} For slot $j$, again, we assume a high unlikely scenario in which $T_O$ has incremented the index and $T_j$ hasn't copied any element from its local buffer to the slot $j$. Before reading slot $j$, $T_O$ must execute $b$ writes to copy its local buffer and $(j-1)b$ reads of first $j-1$ slots. For $j=2$, it must execute $b$ writes and $b$ reads of slot $1$. For $j=3$, it must execute $b$ writes and $2b$ reads of slots $1-2$, etc. 
In order to read at least one hole, $T_O$ must read at least one index in slot $j$ before $T_j$ writes to the corresponding index in that slot. In general, for $i$ writes by $T_j$, $T_O$ must execute $i+1$ reads of slot $j$. The probability of read at least $1$ hole in slot $j$ is bounded by:
\[P(H_j\geq1) \leq P_j = {jb + 2b \choose b} \cdot \left(\frac{1}{2}\right)^{jb + 2b}+\sum_{i=0}^{b-1} {jb+2i+1 \choose i} \cdot \left(\frac{1}{2}\right)^{jb+2i+1}.\]
This is an upper bound on the probability that $T_O$ reads at least $1$ hole in slot $j$ as we double count multiple schedules. As before, we do not know where $T_j$ has started copying its local buffer, therefore:
\[E\left[H_j\right]= P(H_j=0)\cdot 0 + P(H_j=1)\cdot 1 + \dots + P(H_j=b)\cdot b\]
At each slot, $T_O$ can read at most $b$ holes, 
\[E\left[H_j\right] \leq b(P(H_j=0) + P(H_j=1) + \dots P(H_j=b)) = b\cdot P(H_j\geq1) \leq b\cdot P_j\]

The mean of the total number of holes in a batch is 
\[E\left[H\right]= \left[H_1\right] + \left[H_2\right] + \dots + \left[H_{2k/b}\right] \]
There can be at most $N-1$ slots from which to read holes, where $N$ is the number of update threads.
\[ E\left[H\right] \leq \sum_{j=0}^{N-1}P(H_j\geq1)\cdot b \leq \sum_{j=0}^{N-1}P_j\cdot b\]
For $b=16$ and $N=32$,
$E\left[H\right] \approx 0.618 < 1$.
